# Supplementary material for: ISP: Multi-Layered Garment Draping with Implicit Sewing Patterns
Source: arXiv:2305.14100 source file (2023-10-14)
Supplement: Supplementary file 1 [file 6_supp.tex]

% !TEX root = ../top.tex
% !TEX spellcheck = en-US

%In this appendix we first show additional results 

%%%%%%%%%%%%%%%%%%%%%%%%%%%%%%%%%%%%%%%%%%%%%%%%%%%%%%%%%%%%%%%%%%%%%%%%%%%%%%%%
%% CASE 1: standalone supplementary document, with full table of contents.
%%%%%%%%%%%%%%%%%%%%%%%%%%%%%%%%%%%%%%%%%%%%%%%%%%%%%%%%%%%%%%%%%%%%%%%%%%%%%%%%%

% {
%    % Table of content without a huge "CONTENTS" title, with links in blue instead of red.
%    \makeatletter
%    \renewcommand\tableofcontents{%
%        \@starttoc{toc}%
%    }
%    \makeatother
%    \hypersetup{linkcolor=blue}

%    \tableofcontents
% }

%%%%%%%%%%%%%%%%%%%%%%%%%%%%%%%%%%%%%%%%%%%%%%%%%%%%%%%%%%%%%%%%%%%%%%%%%%%%%%%%%
%% CASE 2: supp. is appended to the main paper, with a partial table of contents.
%%%%%%%%%%%%%%%%%%%%%%%%%%%%%%%%%%%%%%%%%%%%%%%%%%%%%%%%%%%%%%%%%%%%%%%%%%%%%%%%%
% \faketableofcontents % (uncomment for first compilation)
% \doparttoc % Tell minitoc to generate part-level ToCs
% \appendix
% \setcounter{part}{1} % Start counting parts from 2
% \part{Appendix}
% \parttoc

%%%%%%%%%%%%%%%%%%%%%%%%%%%%%%%%%%%%%%%%%%%%%%%%%%%%%%%%%%%%%%%%%%%%%%%%%%%%%%%%%
%% CASE 3: hardcoded partial ToC: the above was seemingly not compiling on arXiv.
%%%%%%%%%%%%%%%%%%%%%%%%%%%%%%%%%%%%%%%%%%%%%%%%%%%%%%%%%%%%%%%%%%%%%%%%%%%%%%%%%
\appendix
\part*{Appendix}
\par\noindent\rule{\textwidth}{0.6pt} \par
\qquad \textbf{\hyperref[supp:additional_results]{A ~ Additional Results}} \par
\qquad \qquad \hyperref[supp:texture_editing]{A.1 ~ Texture Editing} \par
\qquad \qquad \hyperref[supp:garment_reconstruction]{A.2 ~ Garment Reconstruction} \par
\qquad \qquad \hyperref[supp:garment_draping_results]{A.3 ~ Garment Draping} \par
\qquad \qquad \hyperref[supp:multilayer_draping_results]{A.4 ~ Multi-Layer Draping} \par
\qquad \textbf{\hyperref[supp:technical_details]{B ~ Technical Details}}  \par
\qquad \qquad \hyperref[supp:sewing_patters]{B.1 ~ Sewing Patterns for Trousers and Skirts}  \par
\qquad \qquad \hyperref[supp:mesh_triangulation]{B.2 ~ Mesh Triangulation}\par
\qquad \qquad \hyperref[supp:proof]{B.3 ~ Proof of the Differentiability of ISP}\par
\qquad \qquad \hyperref[supp:garment_draping]{B.4 ~ Garment Draping}\par
\qquad \qquad \hyperref[supp:recovering_multilayered]{B.5 ~ Recovering Multi-Layered Garments from Images}\par
\qquad \qquad \hyperref[supp:loss_terms]{B.6 ~ Loss Terms, Network Architectures and Training} \par
\qquad \textbf{\hyperref[supp:extension]{C ~ Extension to Sewing Patterns with More Panels}}  \par
\qquad \textbf{\hyperref[supp:failure_cases]{D ~ Failure Cases }}  \par
\par\noindent\rule{\textwidth}{0.6pt}

%%%%%%%%%%%%%%%%%%%%%%%%%%%%%%%%%%%%%%%%%%%%%%%%%%%%%%%%%%%%%%%%%%%%%%%%%%%%%%%%%
%%%%%%%%%%%%%%%%%%%%%%%%%%%%%%%%%%%%%%%%%%%%%%%%%%%%%%%%%%%%%%%%%%%%%%%%%%%%%%%%%

\section{Additional Results}
\label{supp:additional_results}
\subsection{Texture Editing} 
\label{supp:texture_editing}
% !TEX root = ../top.tex
% !TEX spellcheck = en-US

\begin{figure}[h]
    \centering
    \includegraphics[width=0.99\textwidth]{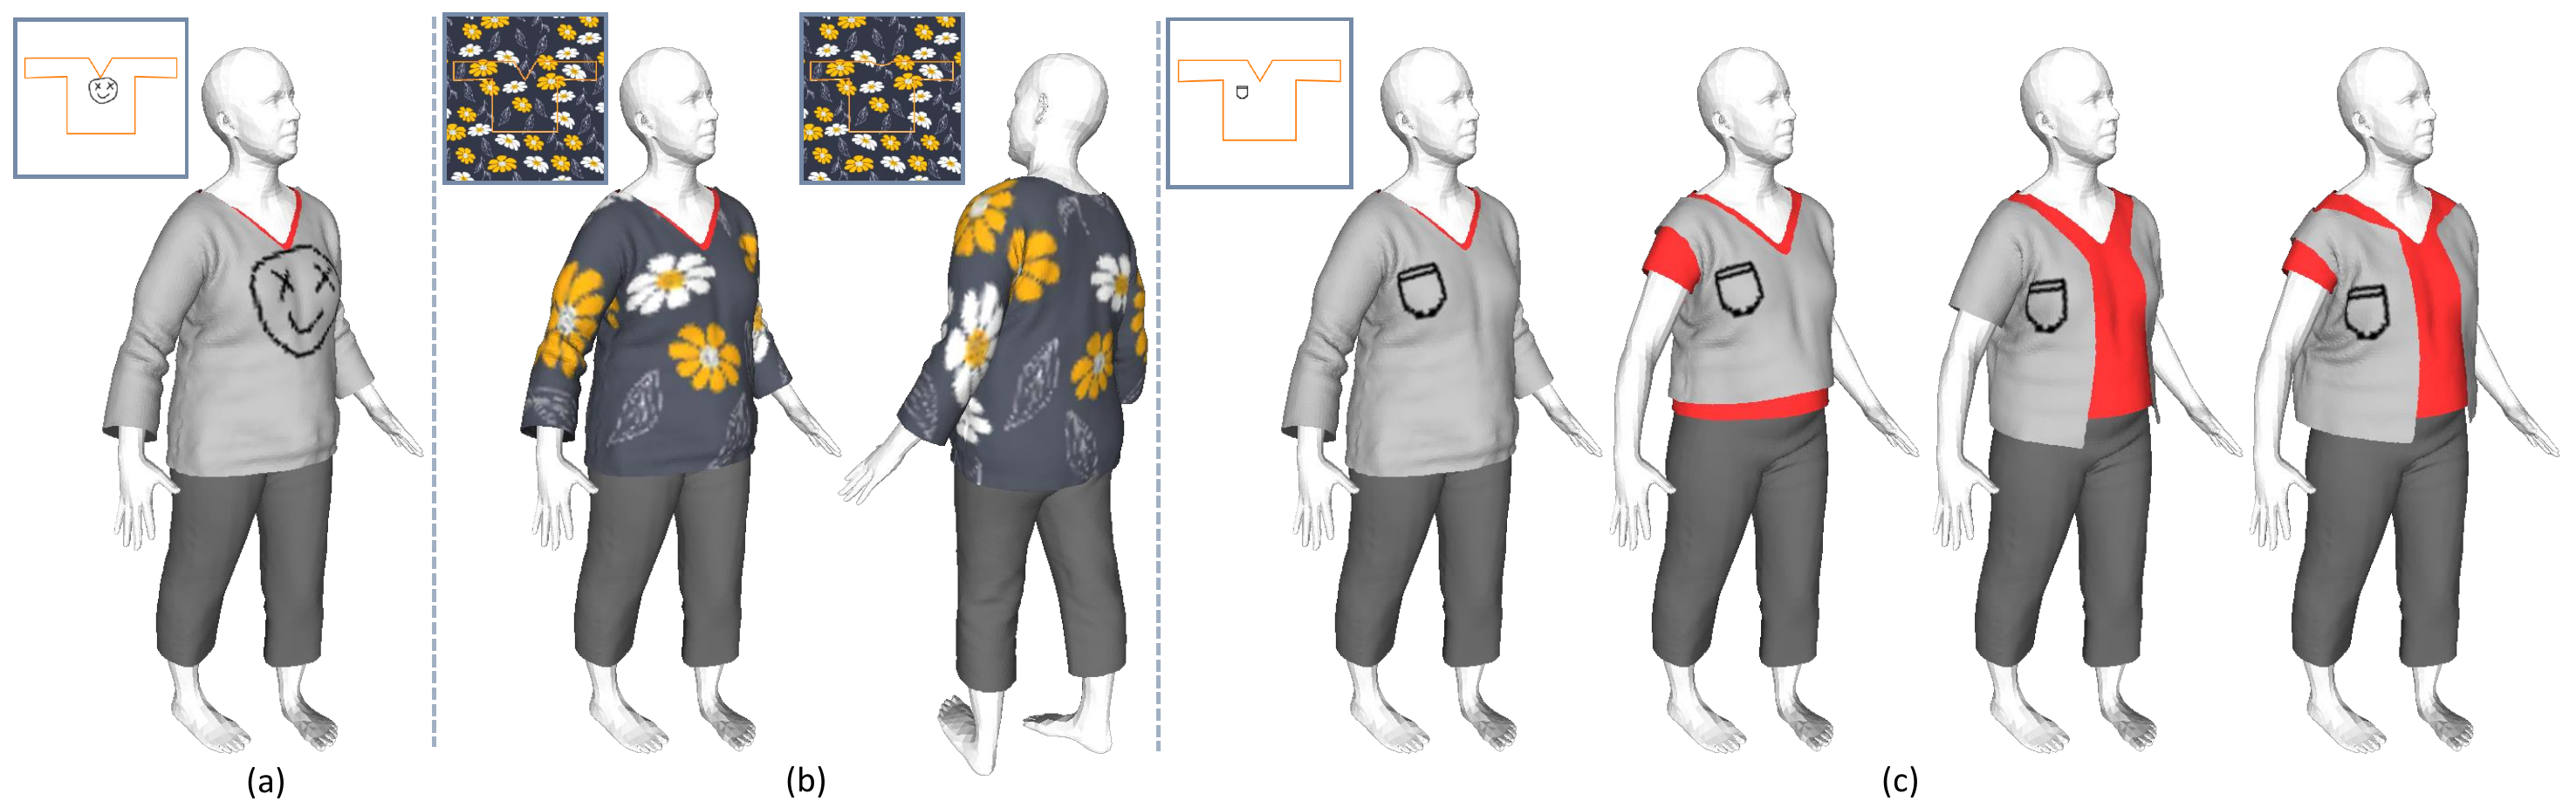}
    %\vspace{-0.35cm}
    \caption{\textbf{Texture editing.}
    \textbf{(a)} A smiling face drawn on the front panel.
    \textbf{(b)} A flower pattern painted on both the front and the back panels.  
    \textbf{(c)} A pocket drawn for the left shirt can be transferred to different garments.}
    \label{fig:texture}
    %\vspace{-0.45cm}
\end{figure} 
As illustrated in Fig.~\ref{fig:texture}, with our ISP, the texture of the garment can be easily edited by drawing on the UV panels. The figures drawn on the panel of one garment can be directly transferred to others as shown by Fig.~\ref{fig:texture}(c), since panels are defined on the same UV space.

\subsection{Garment Reconstruction}
\label{supp:garment_reconstruction}

\subsubsection{Evaluation Results}
% !TEX root = ../top.tex
% !TEX spellcheck = en-US

%\begin{table}
%    \begin{center}
%      \scalebox{1.}{
%            \begin{tabular}{c | c | c | c}
%            \toprule
%             Skirt & CHD ($\times 10^{-4}$, $\downarrow$) & NC (\%, $\uparrow$) & Time (ms, $\downarrow$) \\
%             \midrule
%             UDF - 128  & 0.714 & 98.53 & 690 \\
%             UDF - 256  & 0.408 & 98.93 & 2784 \\
%             UDF - 512  & 0.331 & 98.43 & 17362 \\
%             \midrule
%             Ours - 128  & 0.538 & 98.80 & \textbf{25} \\
%             Ours - 256  & 0.321 & 99.08 & 75 \\
%             Ours - 512  & \textbf{0.267} & \textbf{99.14} & 262 \\
%            \bottomrule
%            \end{tabular}
%            }
%      \end{center}
      %\vspace{-0.5cm}
%      \caption{Comparison of our method to UDF \cite{DeLuigi23} on skirts under the resolutions of 128, 256 and 512.
%      }
%      \label{tab:recon_skirt}
      %\vspace{-6mm}
      %\vspace{-0.5cm}
%  \end{table}
  
\begin{table}[h!]
  \begin{center}
  \scalebox{0.75}{
    \begin{tabular}{c | c | c | c}
      \toprule
       Train & CHD ($\times 10^{-4}$, $\downarrow$) & NC (\%, $\uparrow$) & Time (ms, $\downarrow$) \\
       \midrule
       UDF - 128  & 0.714 & 98.53 & 690 \\
       UDF - 256  & 0.408 & 98.93 & 2784 \\
       UDF - 512  & 0.331 & 98.43 & 17362 \\
       \midrule
       Ours - 128  & 0.538 & 98.80 & \textbf{25} \\
       Ours - 256  & 0.321 & 99.08 & 75 \\
       Ours - 512  & \textbf{0.267} & \textbf{99.14} & 262 \\
      \bottomrule
      \end{tabular}}
      ~~
  \scalebox{0.75}{
    \begin{tabular}{c | c | c}
      \toprule
       Test & CHD ($\times 10^{-4}$, $\downarrow$) & NC (\%, $\uparrow$) \\
       \midrule
       UDF - 128  & 0.734 & 97.79 \\
       UDF - 256  & 0.403 & 98.64 \\
       UDF - 512  & 0.324 & 98.27 \\
       \midrule
       Ours - 128  & 0.583 & 98.62 \\
       Ours - 256  & 0.362 & 98.85 \\
       Ours - 512   & \textbf{0.304} & \textbf{98.89} \\
      \bottomrule
      \end{tabular}
    }
  \end{center}
  \vspace{-1mm}
  \caption{Comparison of our method to UDF on skirts under the resolutions of 128, 256 and 512.}
  \vspace{-4.5mm}
  \label{tab:recon_skirts}
\end{table}

% !TEX root = ../top.tex
% !TEX spellcheck = en-US

%\begin{table}
%    \begin{center}
%      \scalebox{1.}{
%            \begin{tabular}{c | c | c}
%            \toprule
%             Skirt & CHD ($\times 10^{-4}$, $\downarrow$) & NC (\%, $\uparrow$) \\
%             \midrule
%             UDF  & 0.403 & 98.64 \\
%             \midrule
%             Ours  & \textbf{0.362} & \textbf{98.85} \\
%            \bottomrule
%            \end{tabular}
%            }
%      \end{center}
%      %\vspace{-0.5cm}
%      \caption{Comparison of our method to UDF \cite{DeLuigi23} on unseen skirts in resolution 256.
%      }
%      \label{tab:recon_unseen_skirt}
%      %\vspace{-6mm}
%      %\vspace{-0.5cm}
%  \end{table}
\begin{table}[h!]
  \begin{center}
  \scalebox{0.75}{
    \begin{tabular}{c | c | c | c}
      \toprule
       Train & CHD ($\times 10^{-4}$, $\downarrow$) & NC (\%, $\uparrow$) & Time (ms, $\downarrow$) \\
       \midrule
       UDF - 128  & 0.758 & 98.22 & 661 \\
       UDF - 256  & 0.430 & 98.56 & 2650 \\
       UDF - 512  & 0.342 & 98.33 & 17141 \\
       \midrule
       Ours - 128  & 0.545 & 98.28 & \textbf{25} \\
       Ours - 256  & 0.363 & 98.59 & 82 \\
       Ours - 512  & \textbf{0.317} & \textbf{98.62} & 269 \\
      \bottomrule
      \end{tabular}}
      ~~
  \scalebox{0.75}{
    \begin{tabular}{c | c | c}
      \toprule
       Test & CHD ($\times 10^{-4}$, $\downarrow$) & NC (\%, $\uparrow$) \\
       \midrule
       UDF - 128   & 0.752 & 97.41 \\
       UDF - 256   & 0.425 & 98.09 \\
       UDF - 512   & 0.350 & 97.63 \\
       \midrule
       Ours - 128   & 0.529 & 98.03 \\
       Ours - 256   & 0.346 & 98.31 \\
       Ours - 512   & \textbf{0.300} & \textbf{98.32} \\
      \bottomrule
      \end{tabular}
    }
  \end{center}
  \vspace{-1mm}
  \caption{Comparison of our method to UDF on trousers under the resolutions of 128, 256 and 512.}
  \label{tab:recon_pants}
\end{table}
\begin{figure}
    \centering
    \includegraphics[width=0.99\textwidth]{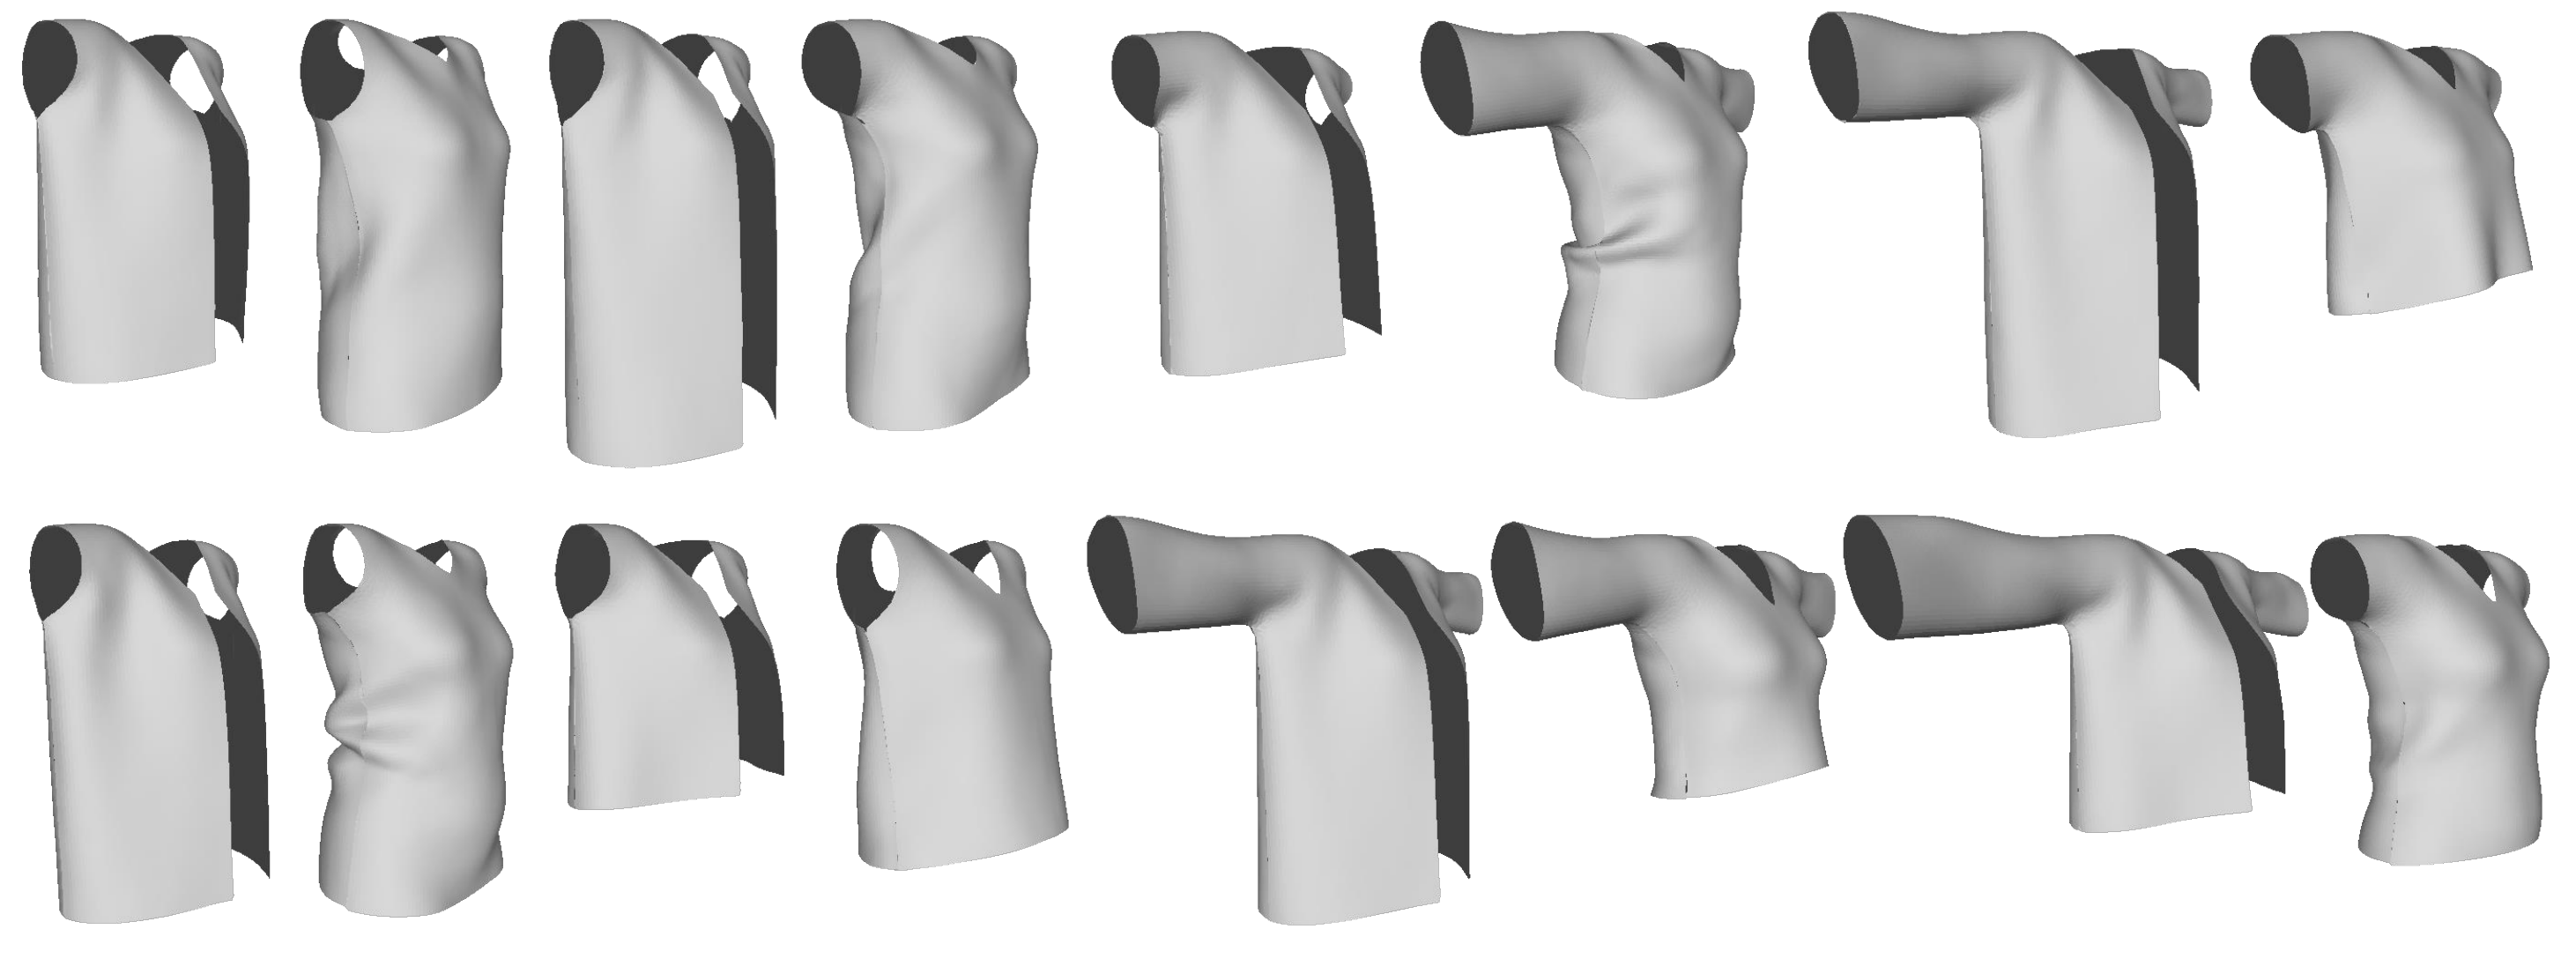}
    %\vspace{-0.35cm}
    \caption{Reconstruction samples of shirts.}
    \label{fig:supp_recon_shirt}
    %\vspace{-0.45cm}
\end{figure} 
\begin{figure}
    \centering
    \includegraphics[width=0.99\textwidth]{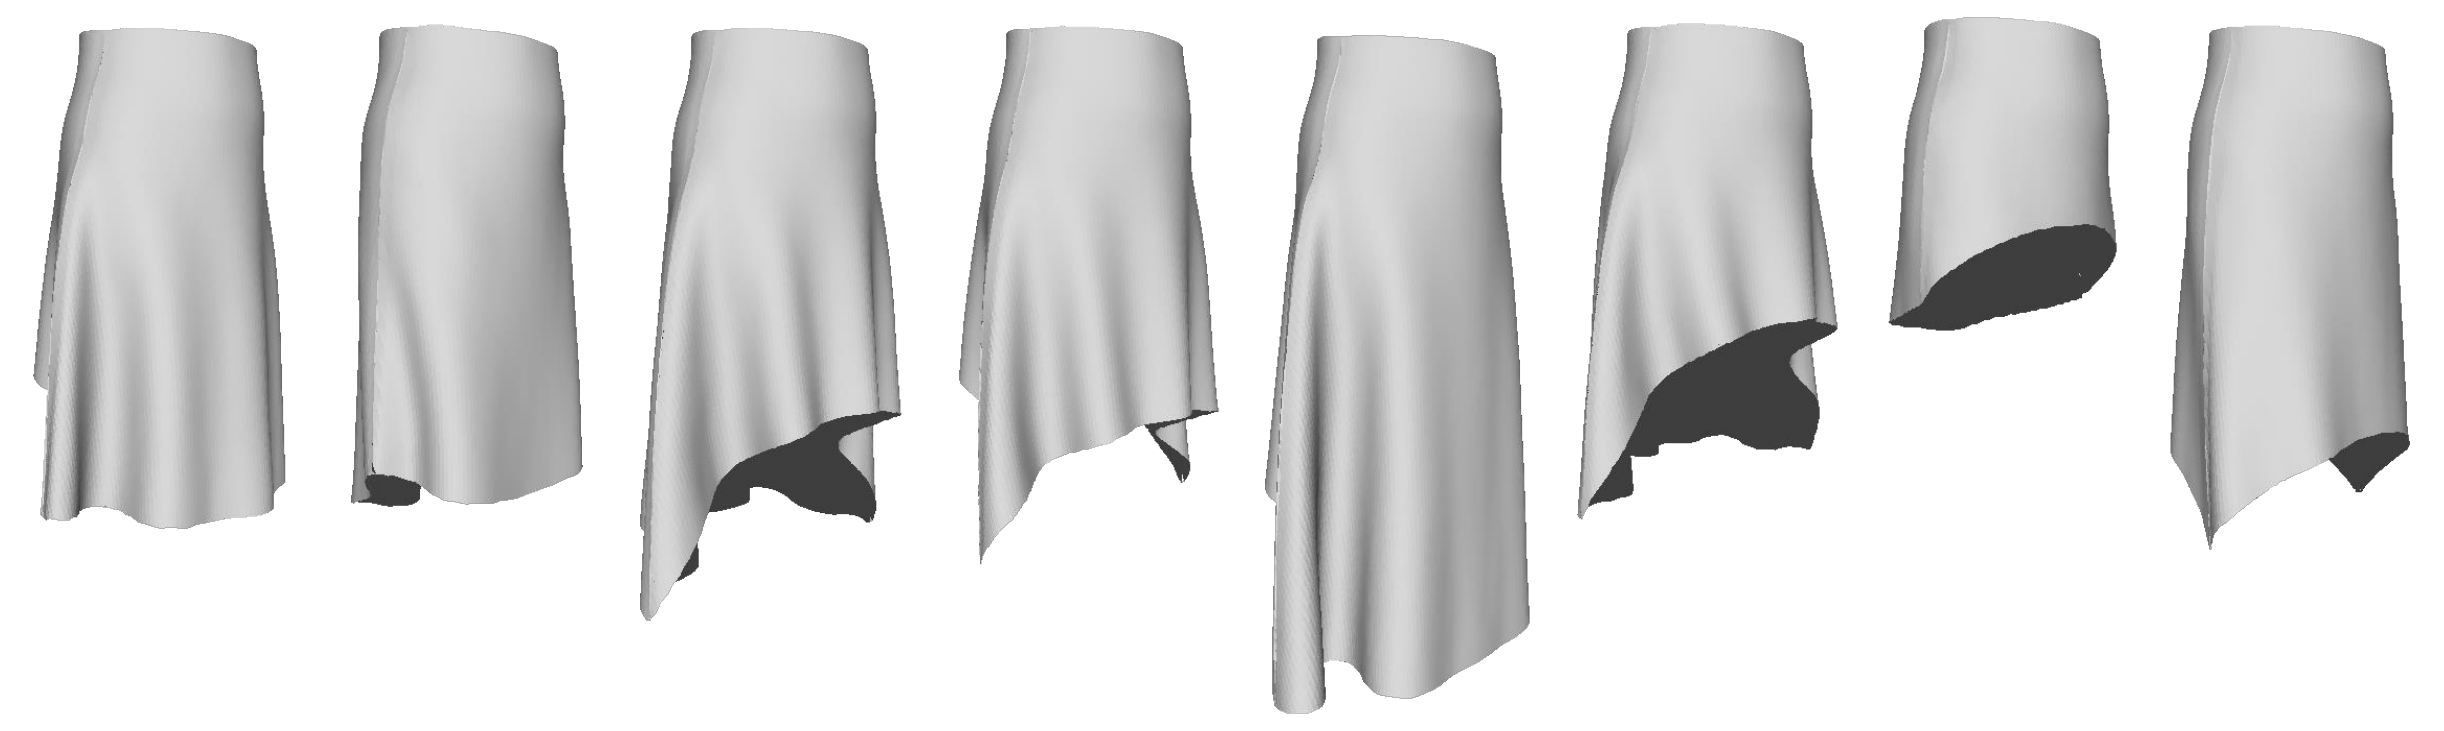}
    %\vspace{-0.35cm}
    \caption{Reconstruction samples of skirts.}
    \label{fig:supp_recon_skirt}
    %\vspace{-0.45cm}
\end{figure} 
\begin{figure}
    \centering
    \includegraphics[width=0.99\textwidth]{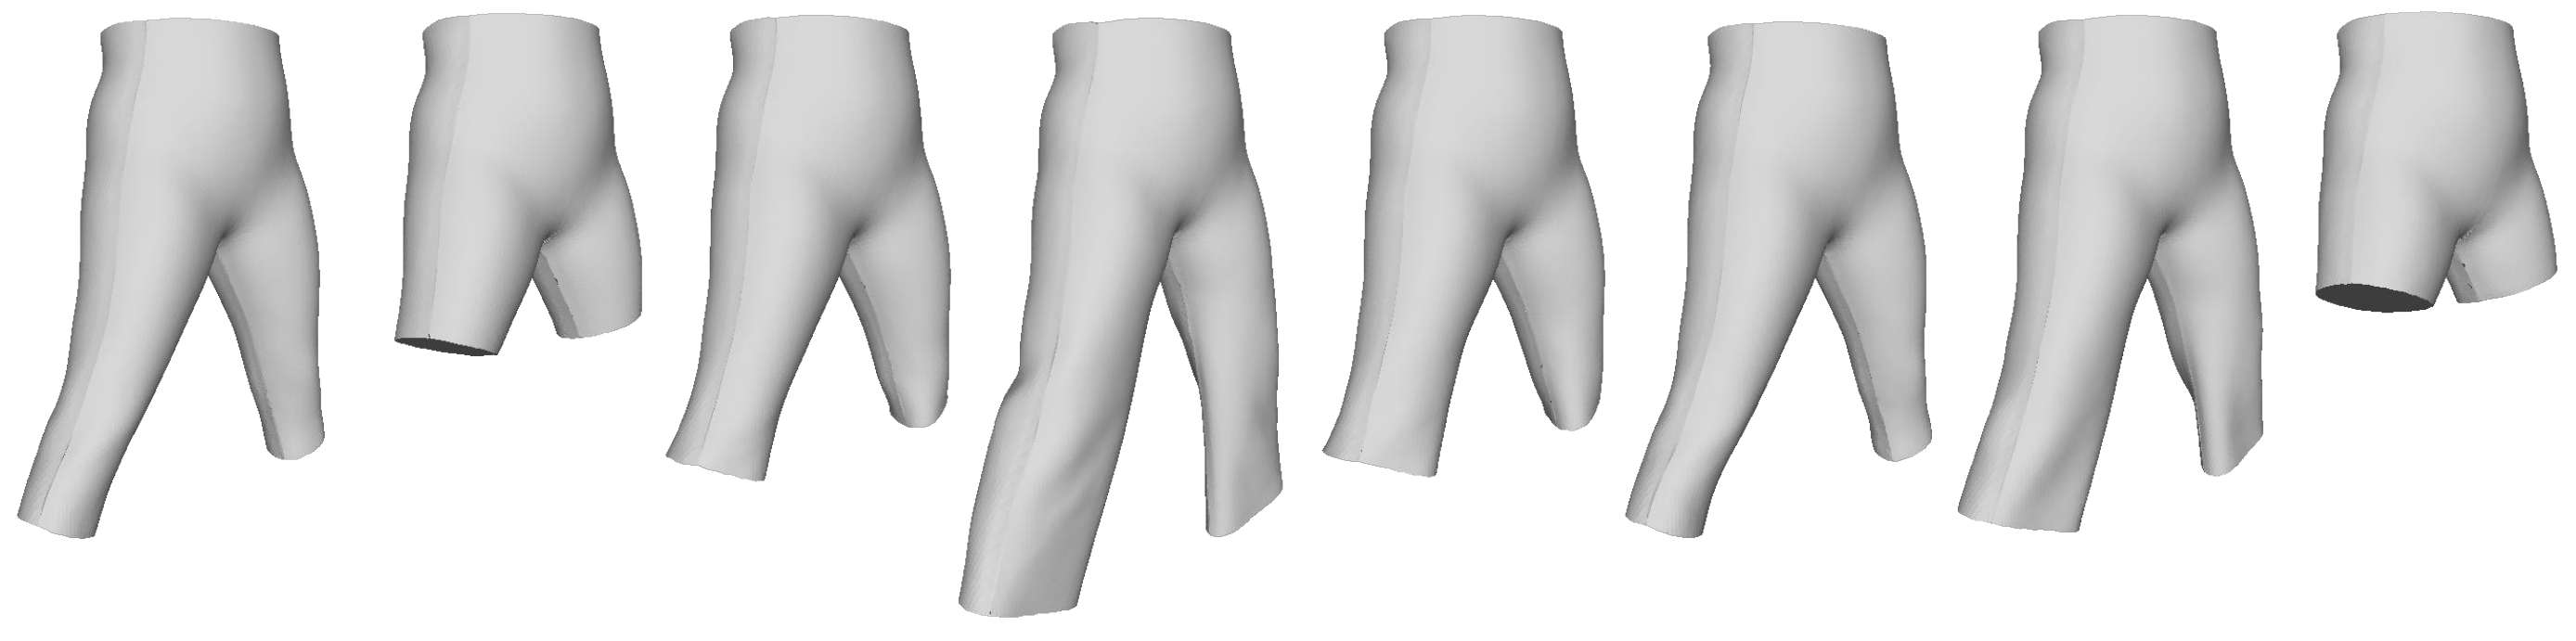}
    %\vspace{-0.35cm}
    \caption{Reconstruction samples of trousers.}
    \label{fig:supp_recon_pants}
    %\vspace{-0.45cm}
\end{figure} 
In \Cref{tab:recon_skirts,tab:recon_pants} we report the reconstruction results for skirts and trousers on the training and the test set. Similar to the results on shirts shown in the main paper, our method achieves better reconstruction quality than UDF~\cite{DeLuigi23} with lower CHD and higher NC at all resolutions, and needs less time to reconstruct a single mesh. \Cref{fig:supp_recon_shirt,fig:supp_recon_skirt,fig:supp_recon_pants} show the qualitative results reconstructed by our method for shirts, skirts and trousers respectively. 

\subsubsection{Latent Space Interpolation}
% !TEX root = ../top.tex
% !TEX spellcheck = en-US

\begin{figure}
    \centering
    \includegraphics[width=0.99\textwidth]{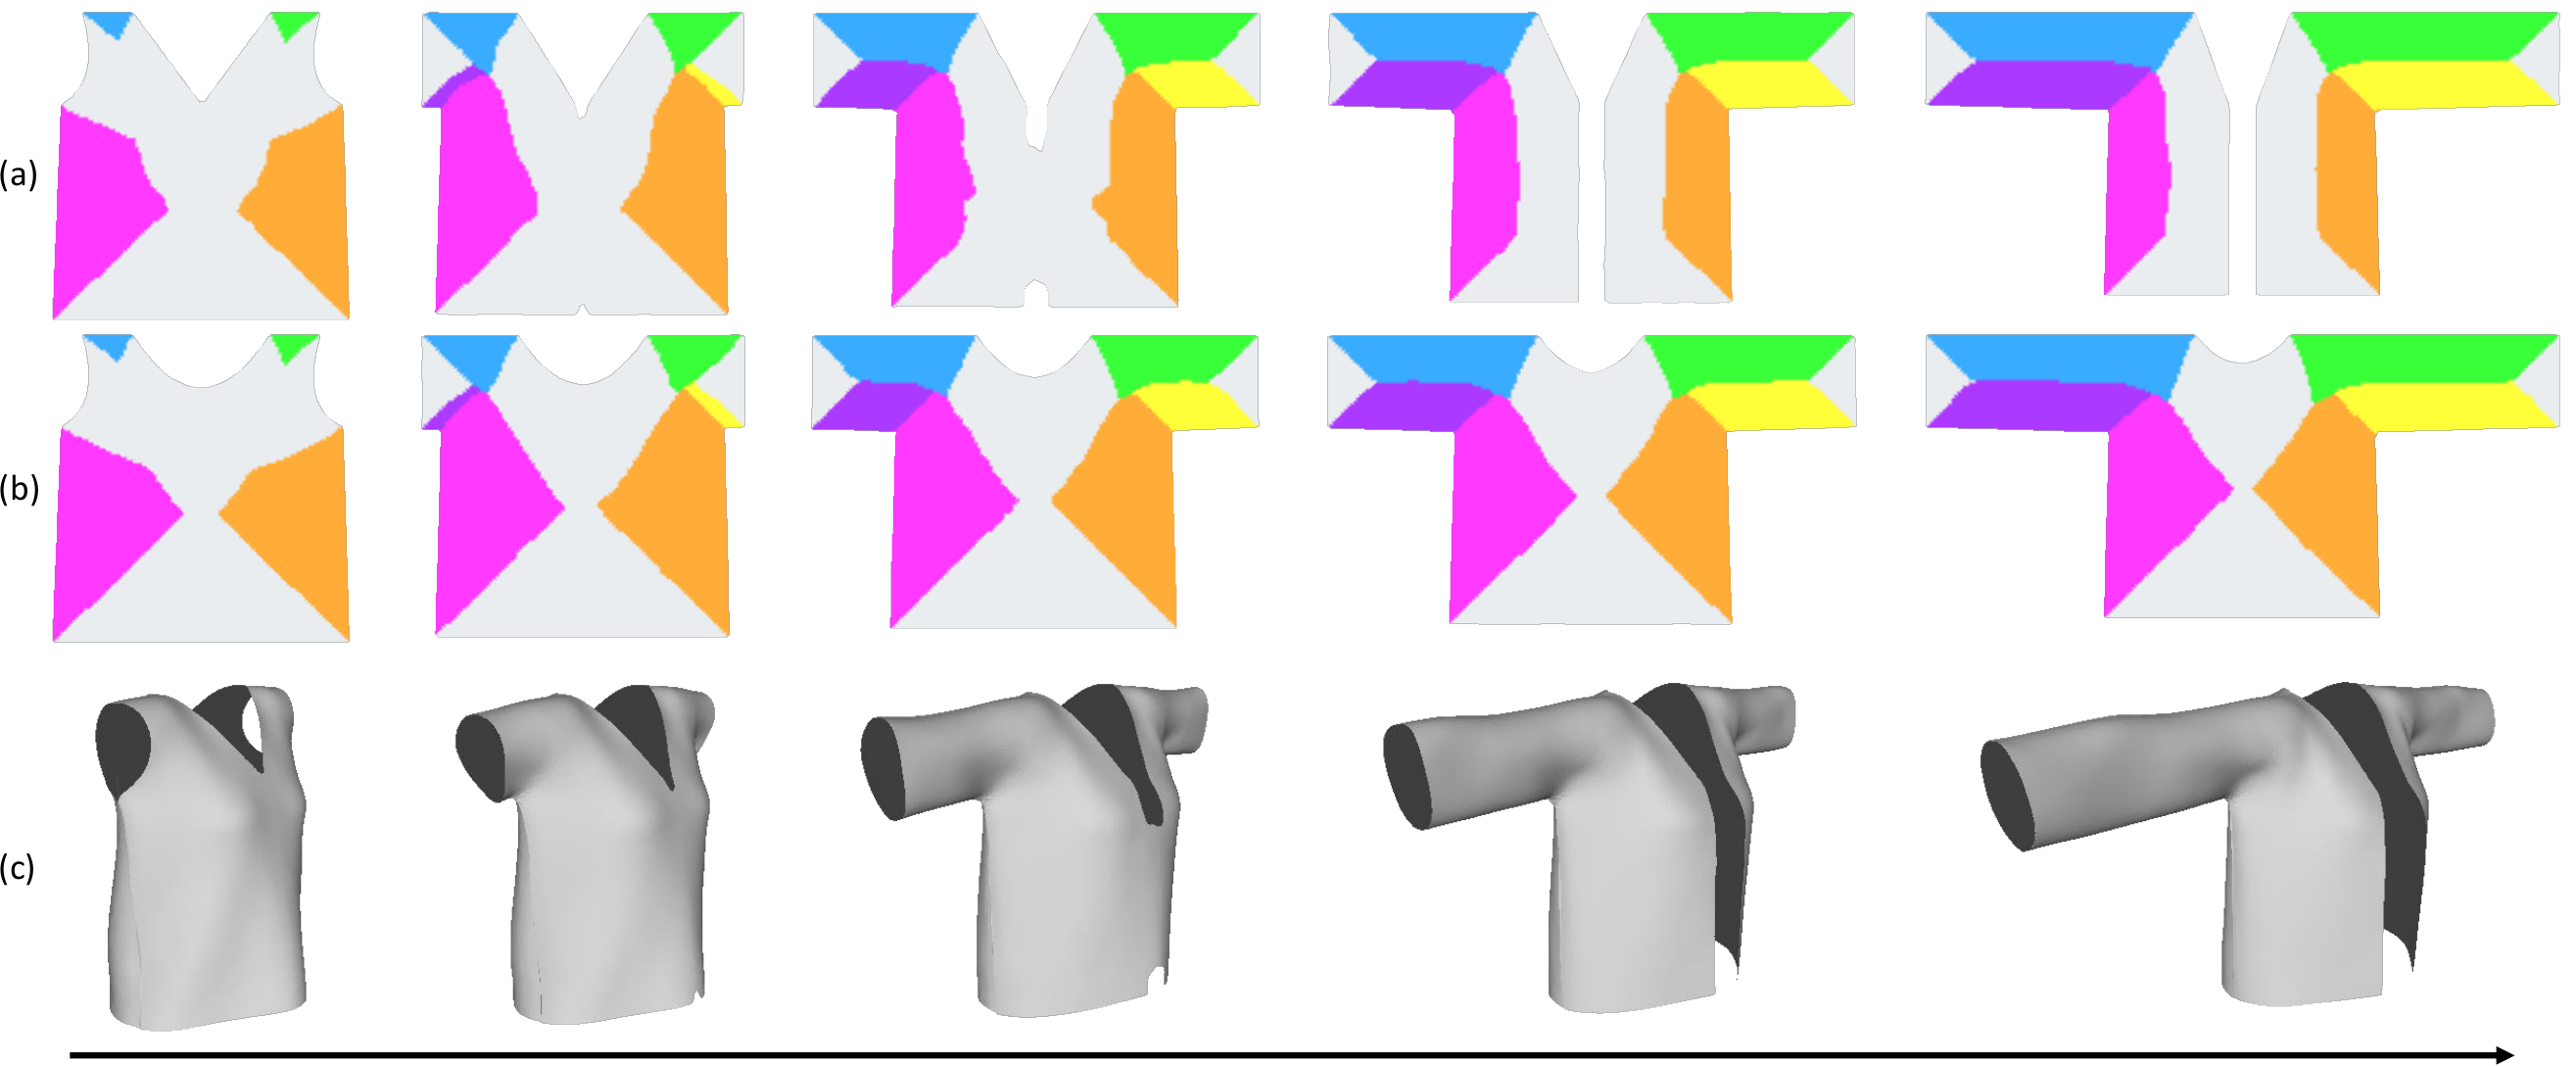}
    %\vspace{-0.35cm}
    \caption{\textbf{Interpolation}. We interpolate the latent code from a sleeveless shirt to a long-sleeve jacket. (a) and (b) show the reconstructed front and back panels, where the colors on them denote the edge label fields. (c) shows the reconstructed mesh.}
    \label{fig:interp}
    %\vspace{-0.45cm}
\end{figure} 
% !TEX root = ../top.tex
% !TEX spellcheck = en-US

\begin{figure}
    \centering
    \includegraphics[width=0.99\textwidth]{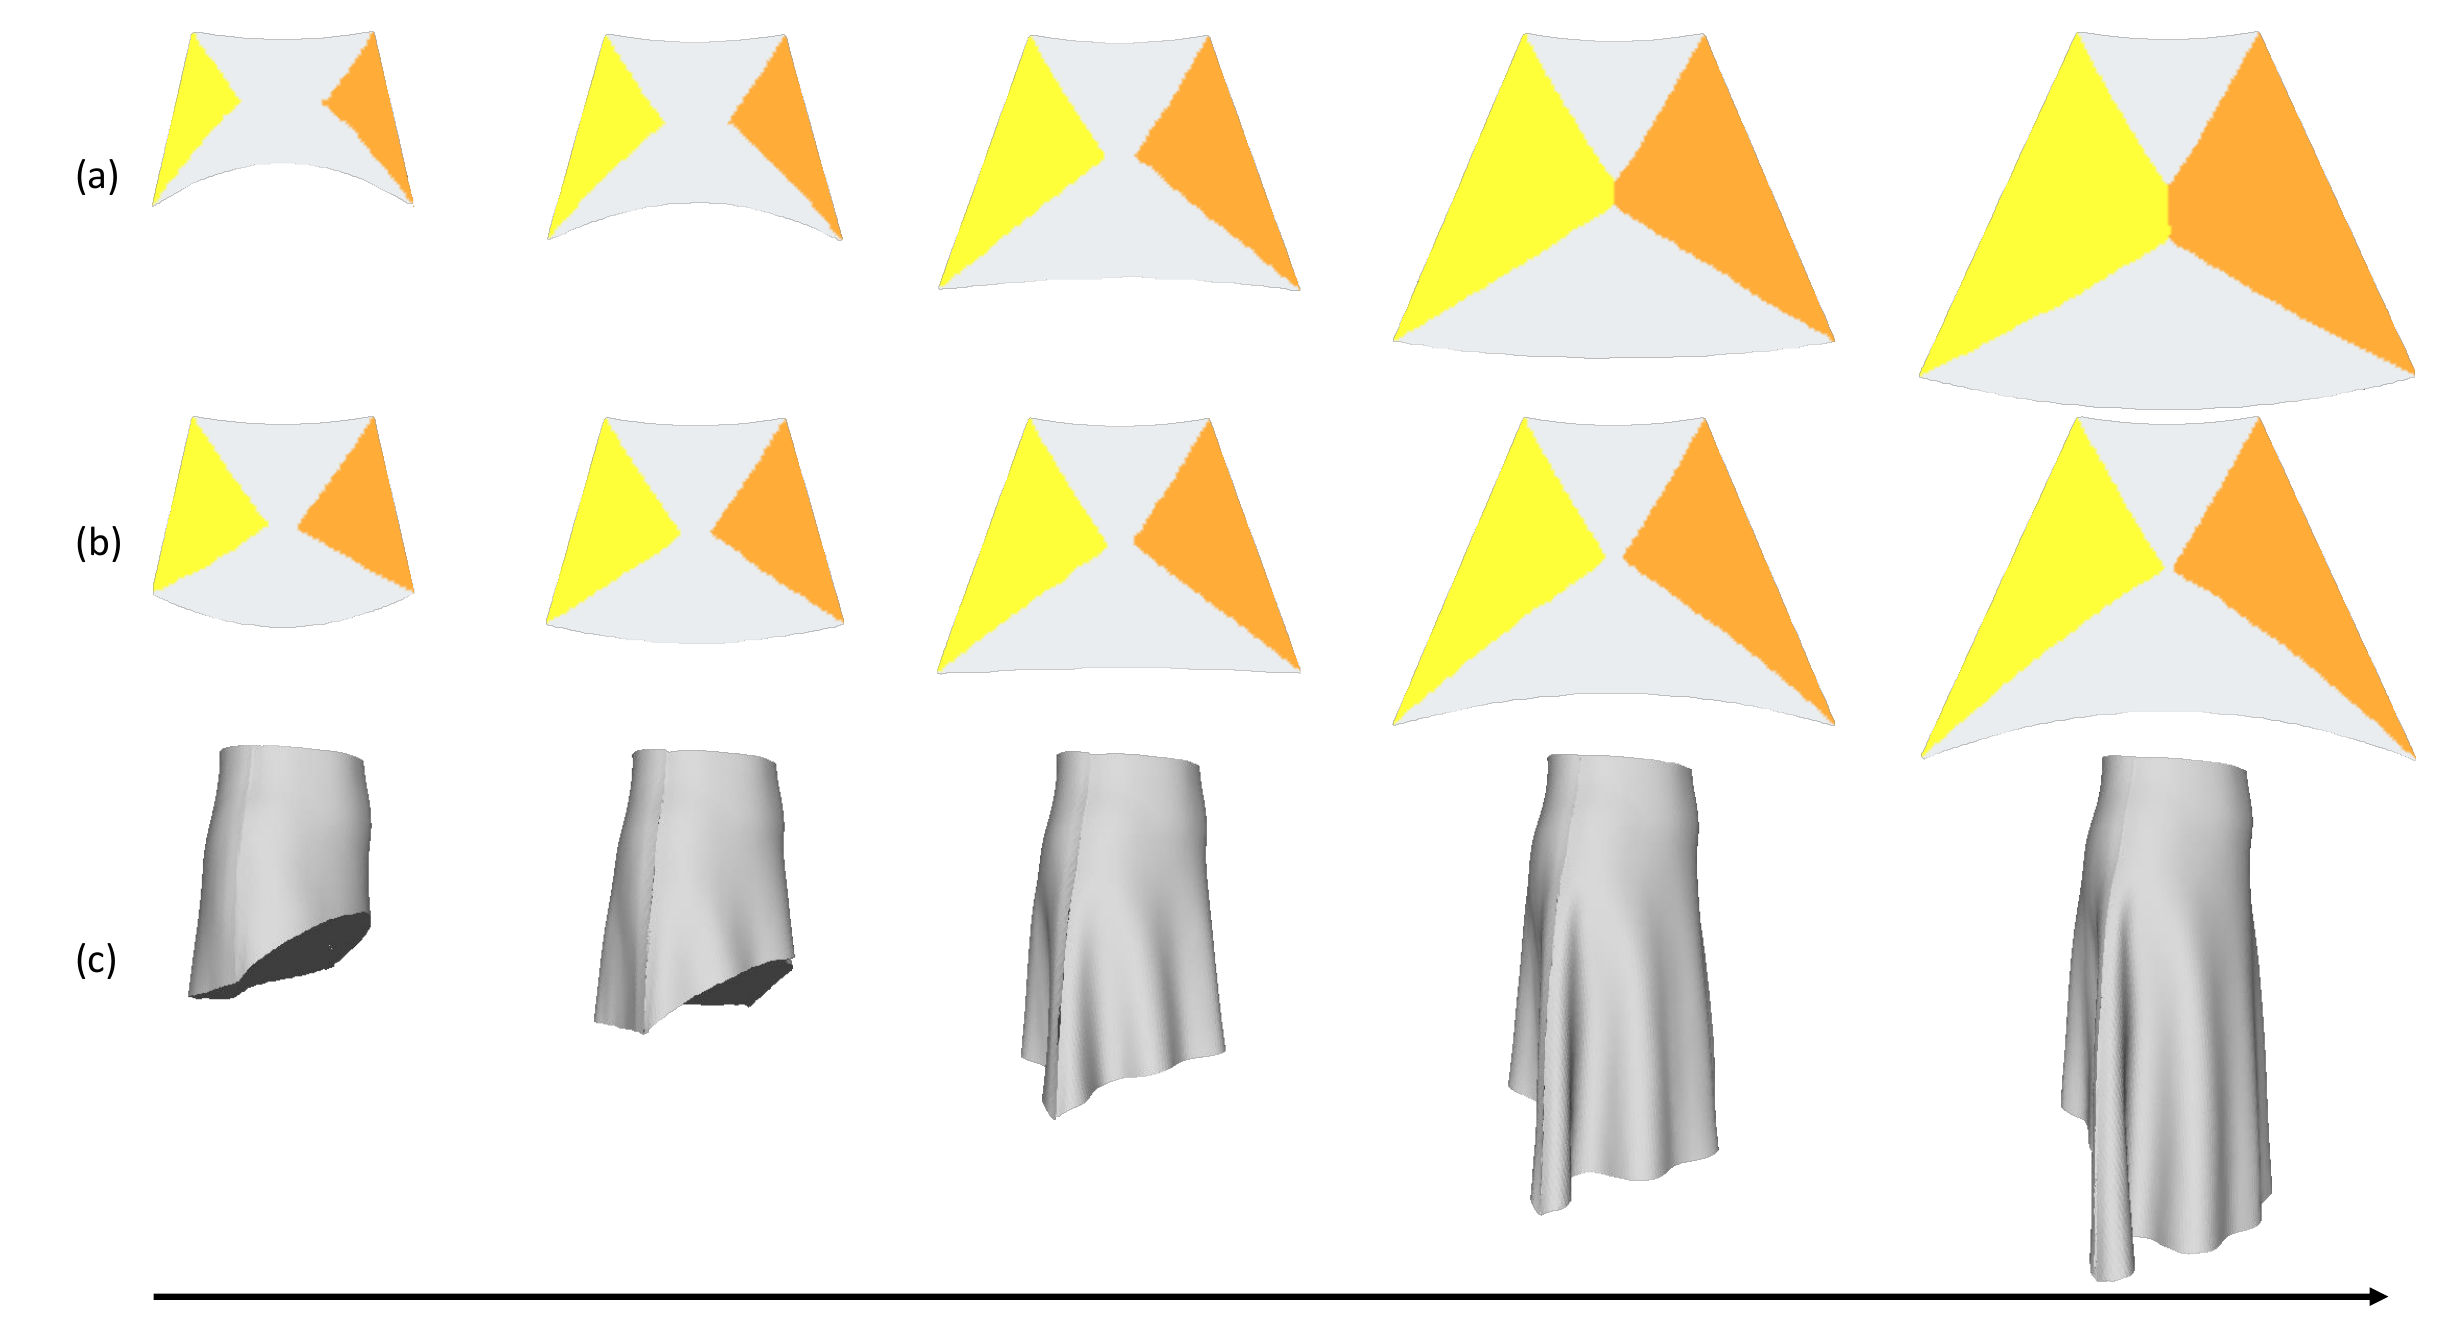}
    %\vspace{-0.35cm}
    \caption{\textbf{Interpolation}. We interpolate the latent code from a short tight skirt to a long loose skirt. (a) and (b) show the reconstructed front and back panels, where the colors on them denote the edge label fields. (c) shows the reconstructed mesh.}
    \label{fig:supp_interp_skirt}
    %\vspace{-0.45cm}
\end{figure} 
% !TEX root = ../top.tex
% !TEX spellcheck = en-US

\begin{figure}
    \centering
    \includegraphics[width=0.99\textwidth]{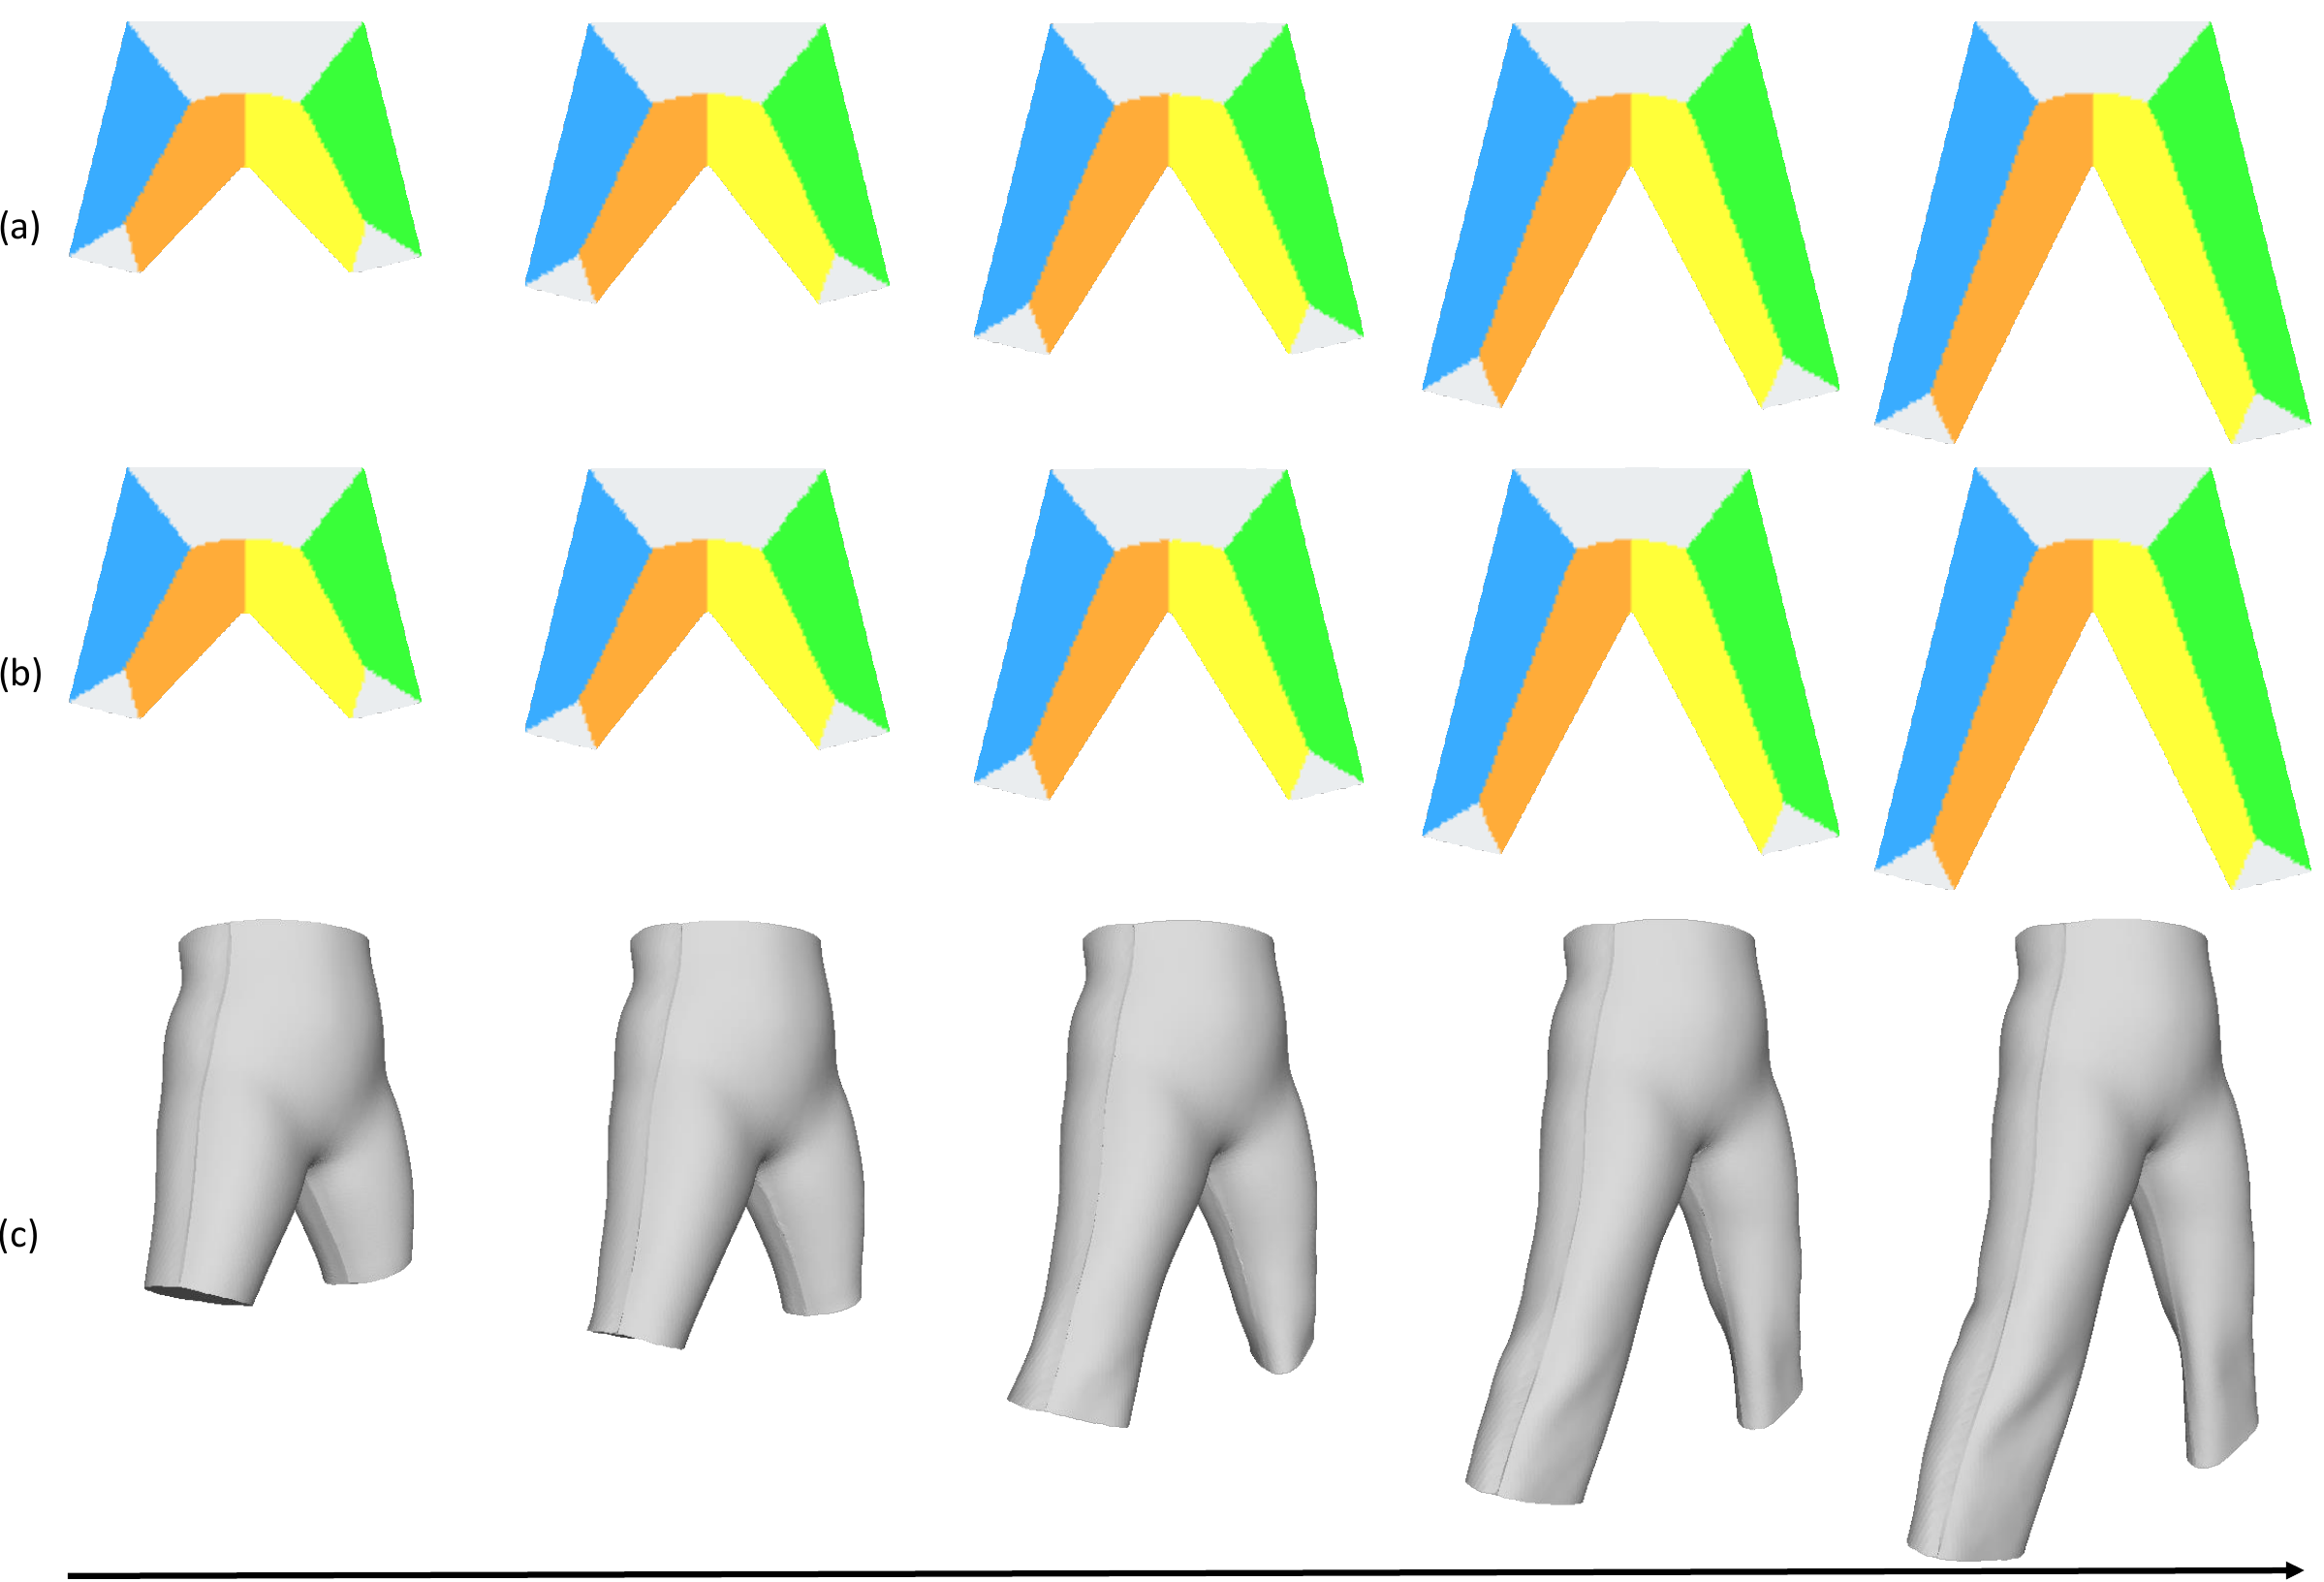}
    %\vspace{-0.35cm}
    \caption{\textbf{Interpolation}. We interpolate the latent code from a pair of short trousers to a pair of long trousers. (a) and (b) show the reconstructed front and back panels, where the colors on them denote the edge label fields. (c) shows the reconstructed mesh.}
    \label{fig:supp_interp_pants}
    %\vspace{-0.45cm}
\end{figure} 
In \Cref{fig:interp,fig:supp_interp_skirt,fig:supp_interp_pants}, we display the results of interpolation in the latent space of shirts, skirts and trousers respectively. We observe a smooth transformation in both the reconstructed sewing patterns and the garment meshes, despite the different topology and geometry of the given garments.

\subsubsection{Comparison with AtlasNet}
% !TEX root = ../top.tex
% !TEX spellcheck = en-US

\begin{figure}
    \centering
    \includegraphics[width=0.99\textwidth]{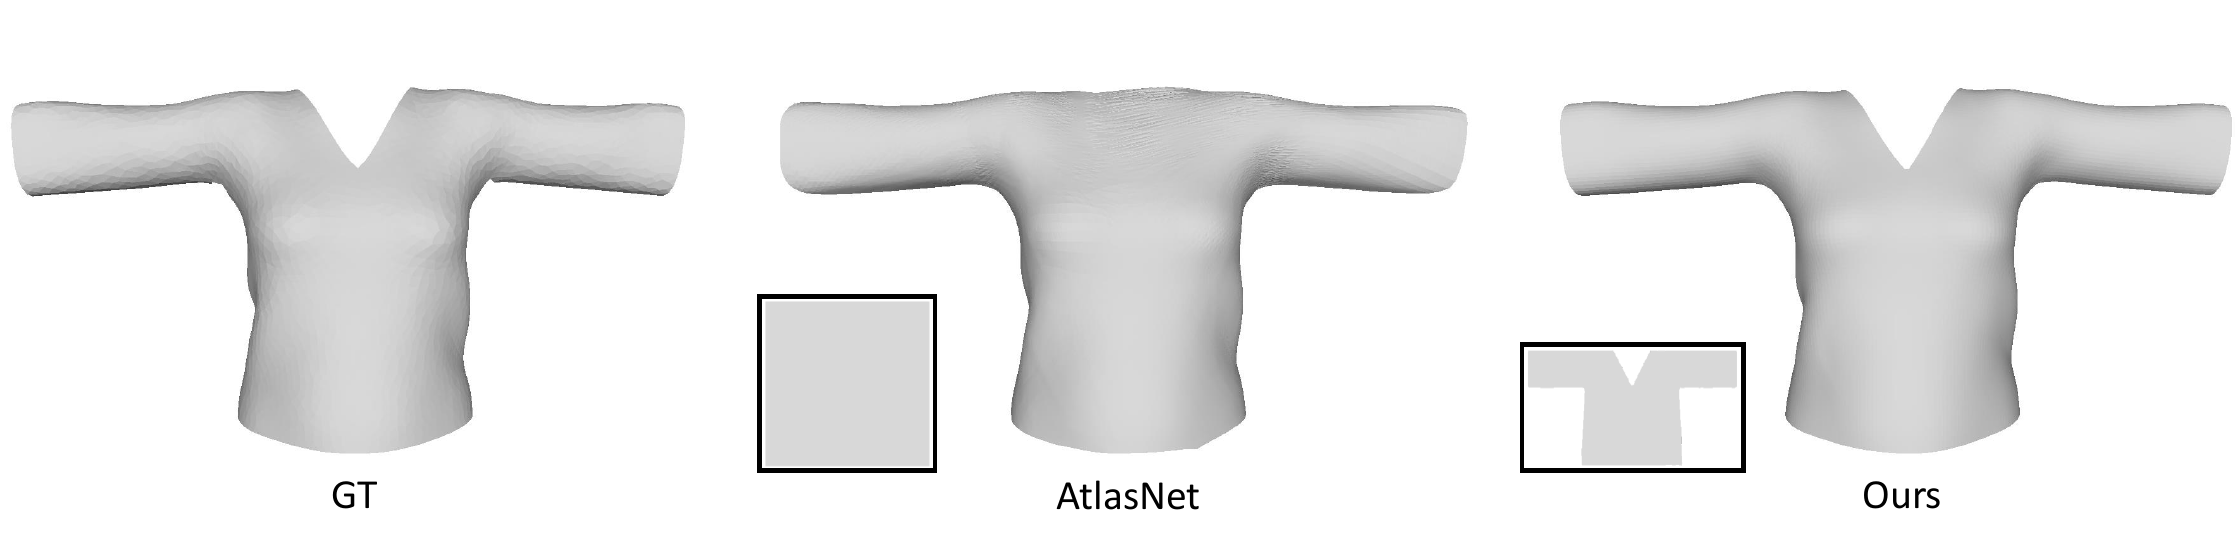}
    %\vspace{-0.35cm}
    \caption{\textbf{Comparison with AtlasNet}. The meshes in black boxes are the source patches where the mapping function is applied: a square patch for AtlastNet, a garment panel for our method.}
    \label{fig:supp_atlas}
    %\vspace{-0.45cm}
\end{figure} 
In Fig.~\ref{fig:supp_atlas}, we compare our method with AtlasNet~\cite{Groueix18a} which learns to deform a square patch. AtlasNet struggles to learn a mapping function capable of accurately deforming the square patch to produce a surface that matches the ground truth, especially in the collar region. In contrast, our method leverages the pattern parameterization network $\mathcal{I}_{\Theta}$ to simplify the training of our mapping function $\mathcal{A}_{\Phi}$. Specifically, our approach only requires learning the mapping for points within the panels, resulting in a reconstruction that is more faithful to the ground truth.

\subsubsection{Ablation Study} 
\begin{figure}[t]
	\centering
		\begin{minipage}{.4\textwidth}
				\centering
		% \vspace{1mm}
		\includegraphics[width=.99\textwidth]{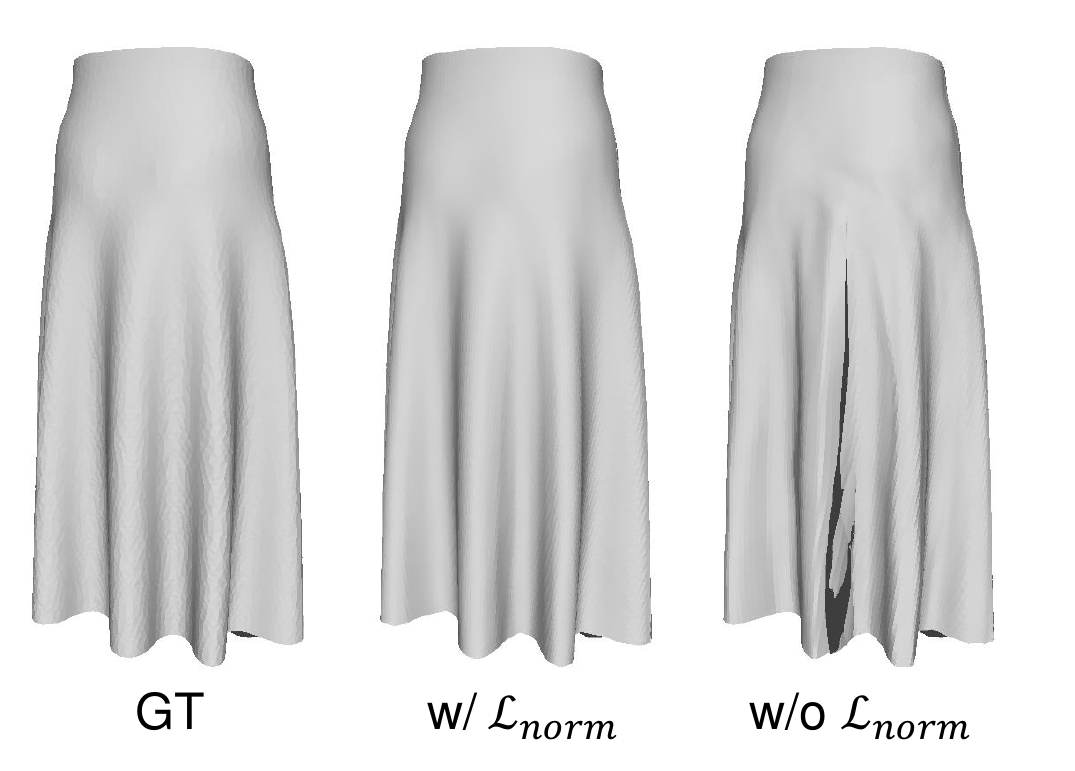}
		% \vspace{-7mm}
		\captionof{figure}{\textbf{Ablation on $\mathcal{L}_{normal}$}. Training without it yields flipped triangle faces (shown in dark grey).}
		\label{fig:normal}
	\end{minipage}
	% \hspace{0mm}
	\begin{minipage}{.57\textwidth}
		\centering
		\includegraphics[width=.99\textwidth]{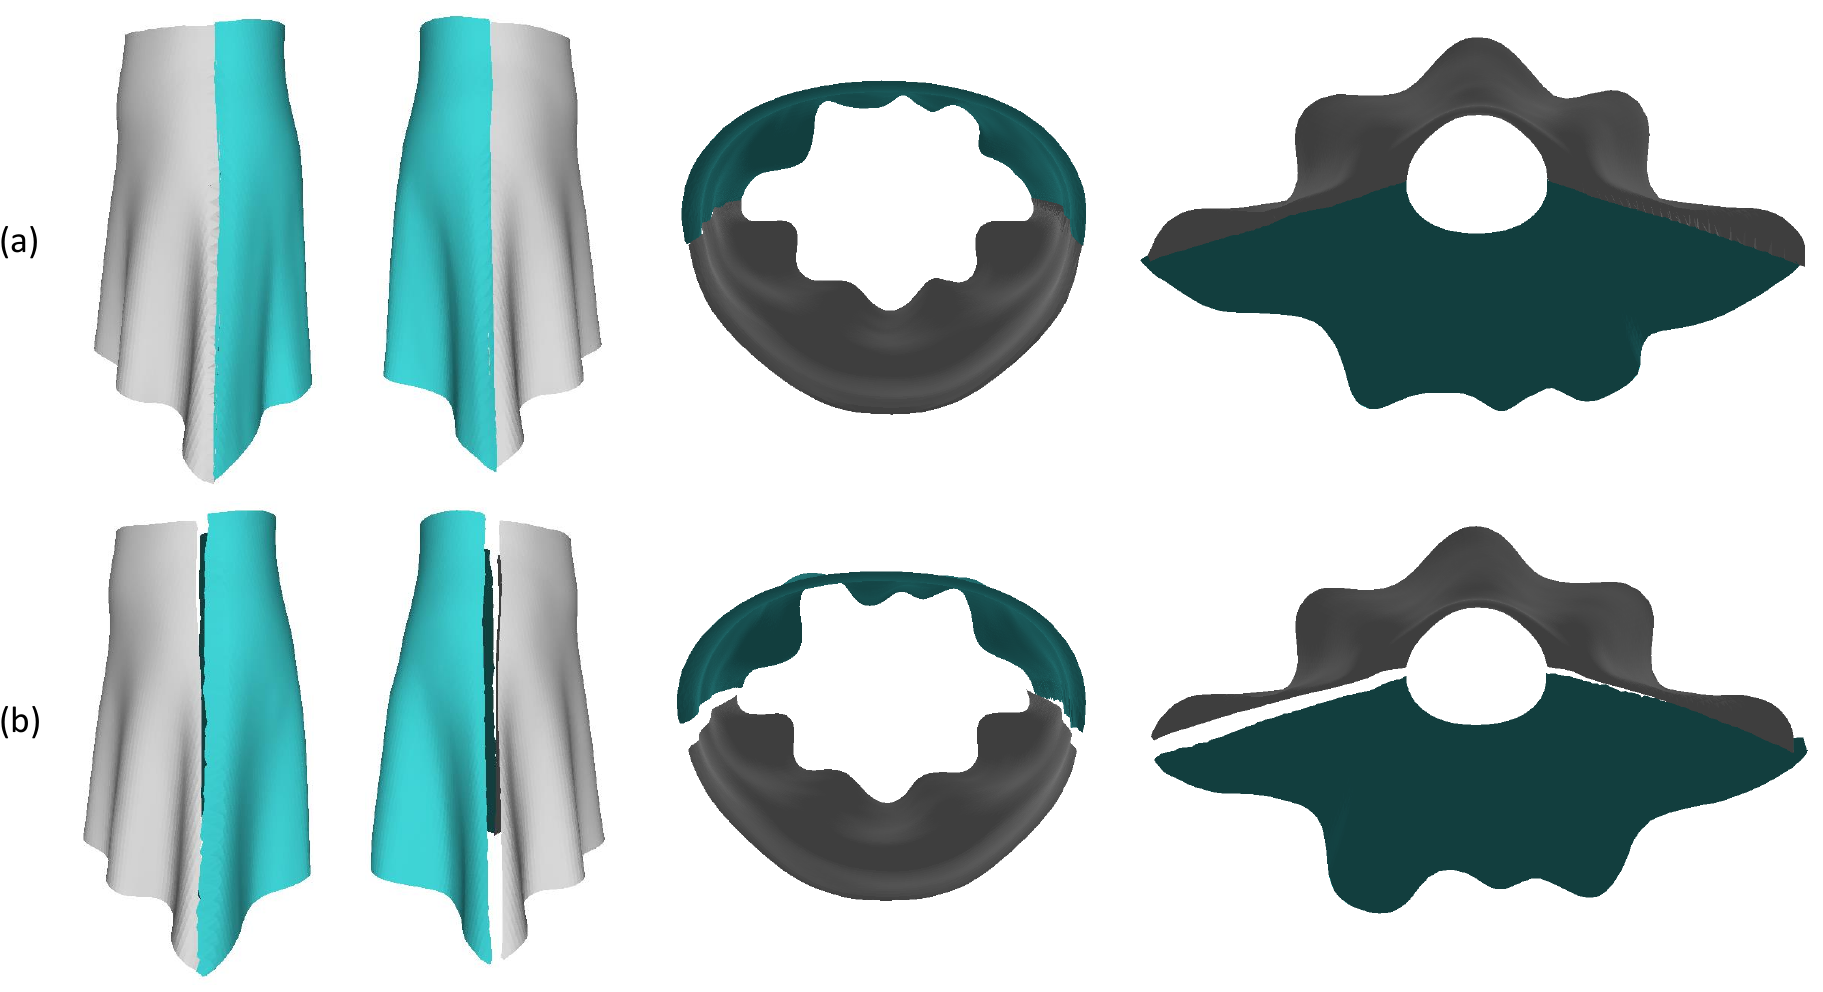}
		% \vspace{-10pt}
		\captionof{figure}{\textbf{Ablation on $\mathcal{L}_{consist}$}. The skirts reconstructed by the models trained (a) with $\mathcal{L}_{consist}$ and (b) without $\mathcal{L}_{consist}$. The latter has a gap between its front and back panels.}
		\label{fig:consist}
	\end{minipage}%
	% \vspace{-6mm}
\end{figure}
% !TEX root = ../top.tex
% !TEX spellcheck = en-US

\begin{table}
  \begin{center}
    \scalebox{1.}{
          \begin{tabular}{c | c | c }
          \toprule
             & CHD ($\times 10^{-4}$, $\downarrow$) & NC (\%, $\uparrow$)\\
           \midrule
           w/o $\mathcal{L}_{normal}$  & 0.324 & 98.69  \\
           w/ $\mathcal{L}_{normal}$  & 0.321 & 99.08  \\
          \bottomrule
          \end{tabular}
          }
    \end{center}
    %\vspace{-0.5cm}
    \caption{Comparison of the results reconstructed by the models trained w/o and w/ $\mathcal{L}_{normal}$.
    }
    \label{tab:normal}
    %\vspace{-6mm}
\end{table}

To investigate the impact of the loss terms of Eq.~(4) in the main paper on reconstruction quality, we performed an ablation study. We report the results of reconstructing 300 skirts using models trained with and without $\mathcal{L}_{normal}$ in \Cref{tab:normal}. We observe that training with $\mathcal{L}_{normal}$ reduces the CHD and increases the NC, thus improving the reconstruction accuracy. In contrast, without $\mathcal{L}_{normal}$, the model fails to learn the correct parameterization for the garment, resulting in a mesh with inverted faces as illustrated in \Cref{fig:normal}.
\Cref{fig:consist} shows a comparison of the results obtained by training models without and with $\mathcal{L}_{consist}$ to help stitch the front and back panels. We can notice that without $\mathcal{L}_{consist}$, a spatial gap exists between the front (in gray) and back (in cyan) surfaces.

\subsubsection{Vizualization of the Chamfer Distance}
% !TEX root = ../top.tex
% !TEX spellcheck = en-US

\begin{figure}
    \centering
    \includegraphics[width=0.95\textwidth]{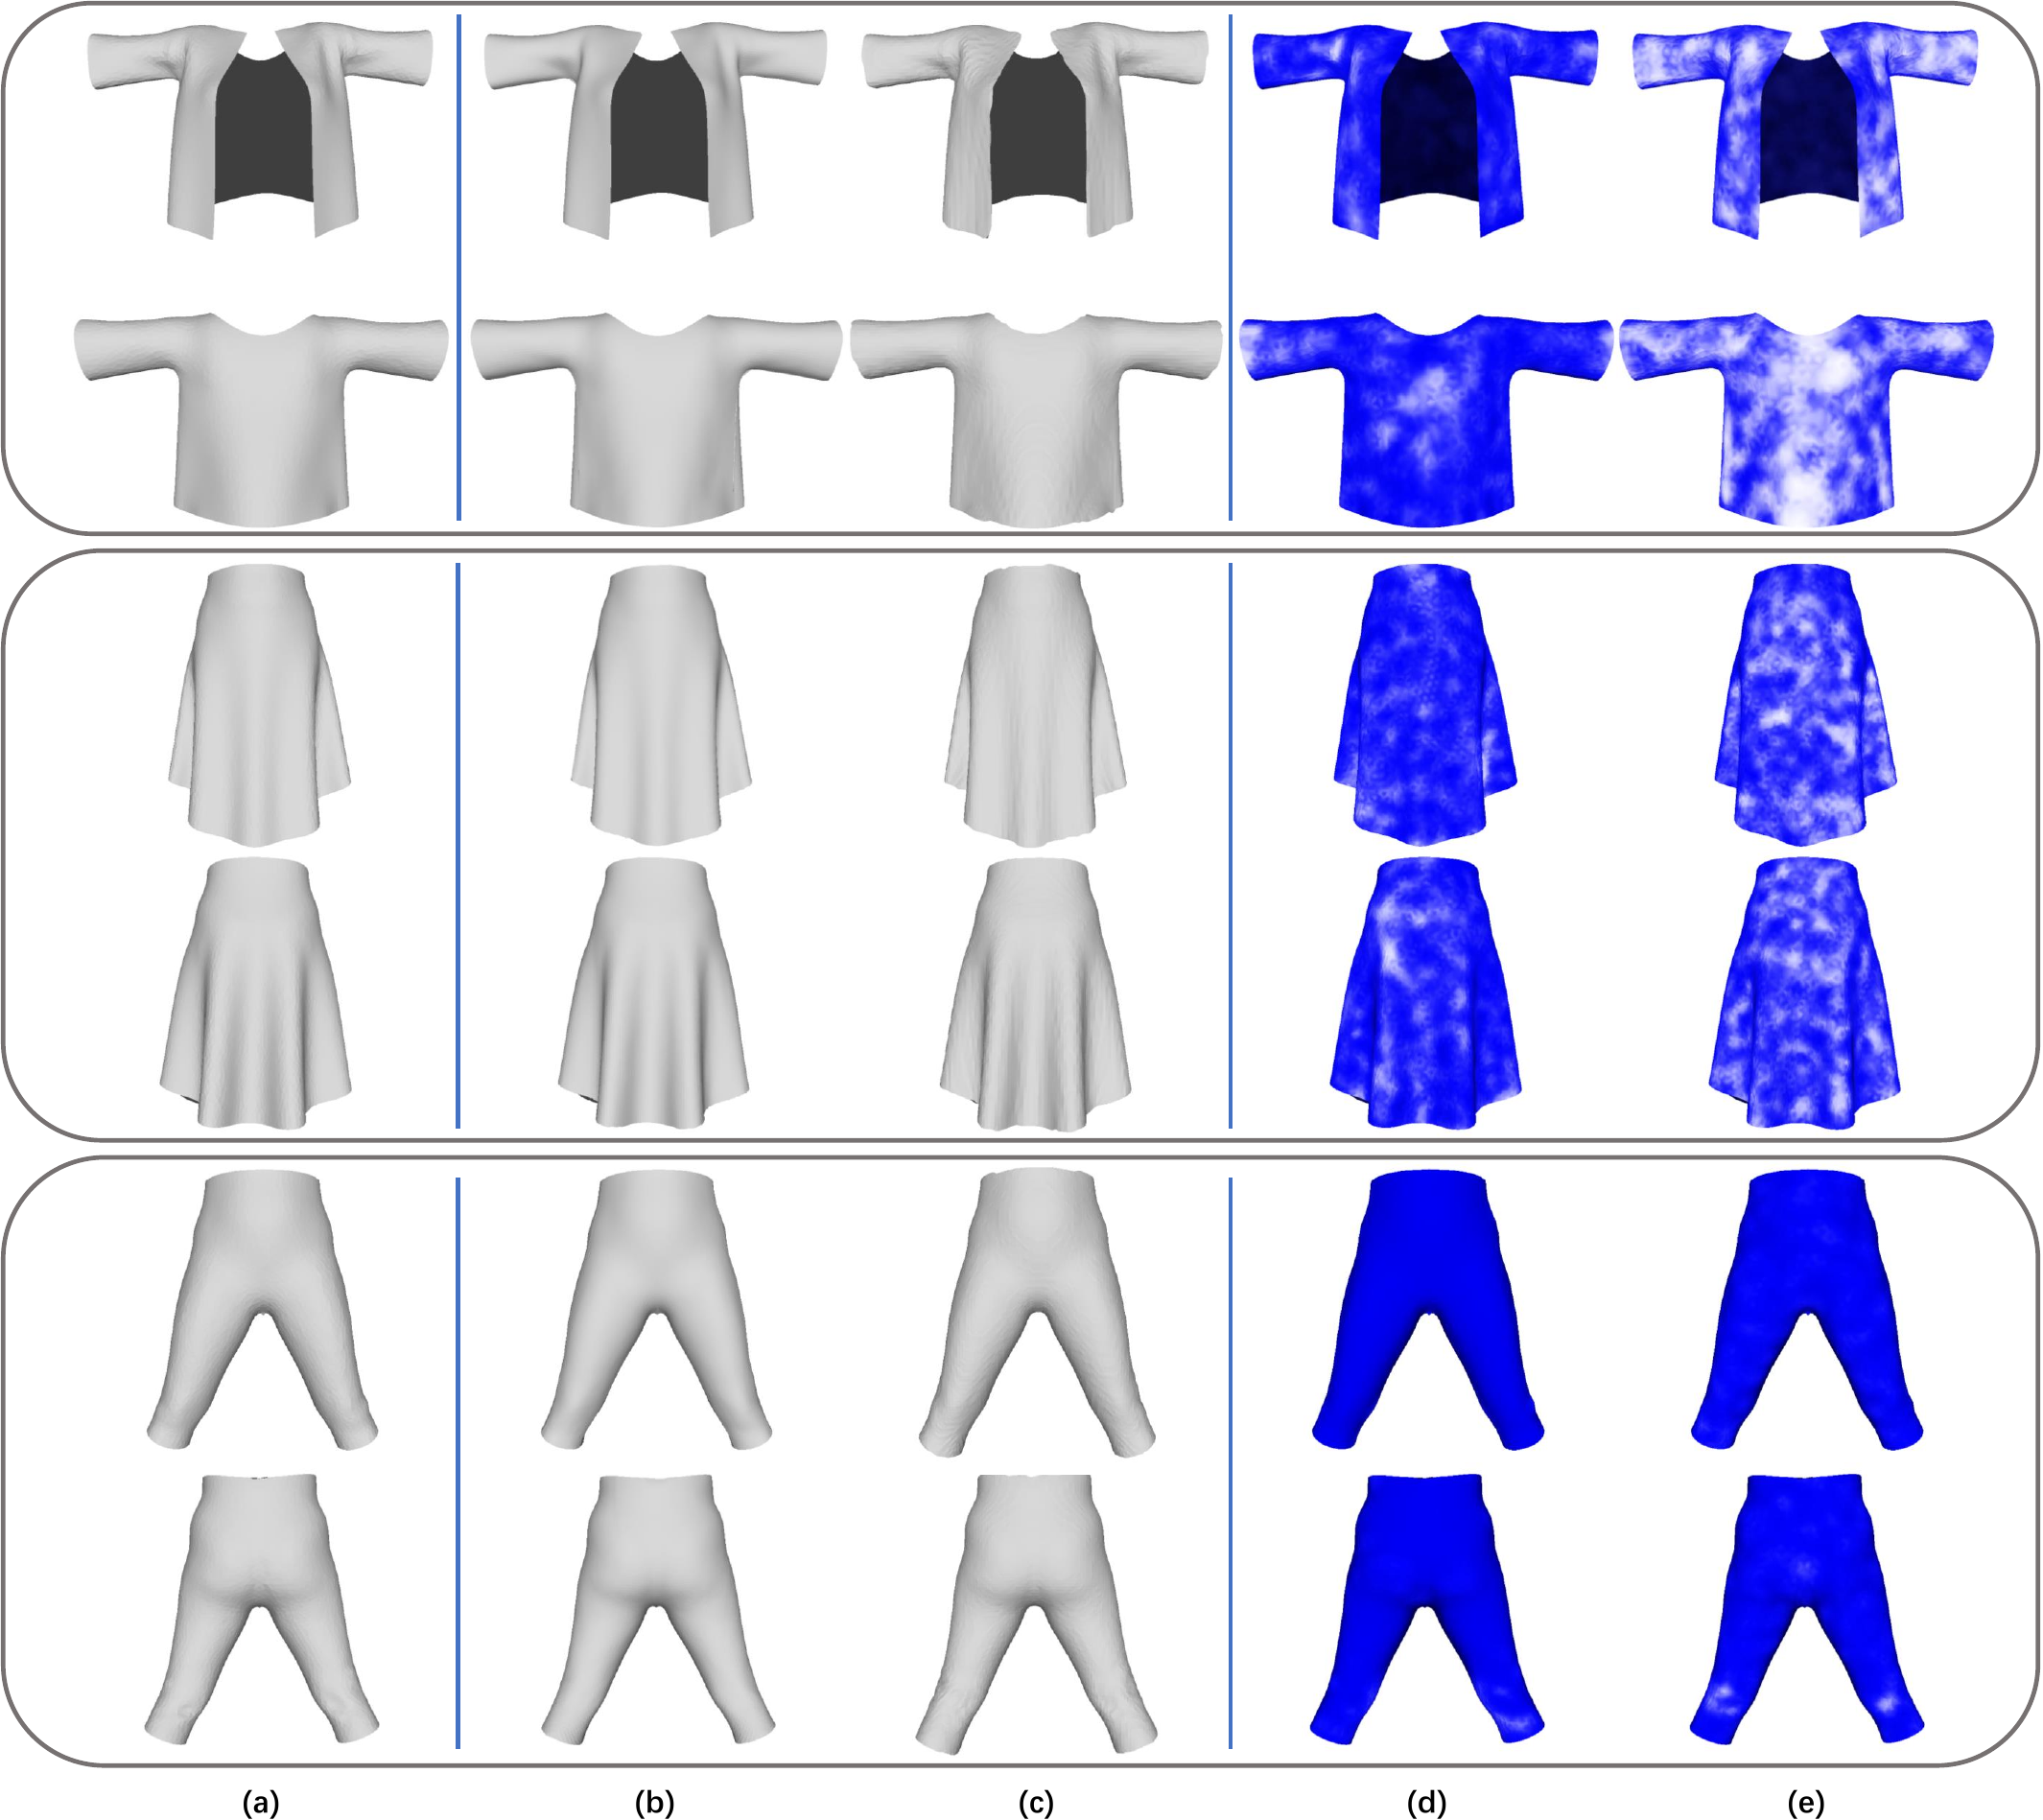}
    \caption{\textbf{Comparative analysis of mesh reconstruction and spatial error distribution for shirt, skirt and trousers}. (a) represents the ground truth mesh. (b) and (d) illustrate the mesh reconstruction and corresponding spatial error distribution for our proposed method. (c) and (e) display the same for UDFs. Each row provides both front (upper half) and back (lower half) views. In (d) and (e), error magnitude is indicated by color gradation, with white representing large errors and blue small errors.}
    \label{fig:supp_heatmap}
\end{figure} 

A visualization of the spatial error distribution can be found in \Cref{fig:supp_heatmap}. In this figure, we compare the error distribution between our reconstructions and those produced by UDFs. Our reconstructions exhibit lower error across the entire surface compared to UDFs.

\subsection{Garment Draping}
\label{supp:garment_draping_results}
% !TEX root = ../top.tex
% !TEX spellcheck = en-US

\begin{figure}[ht!]
    \centering
    \includegraphics[width=0.99\textwidth]{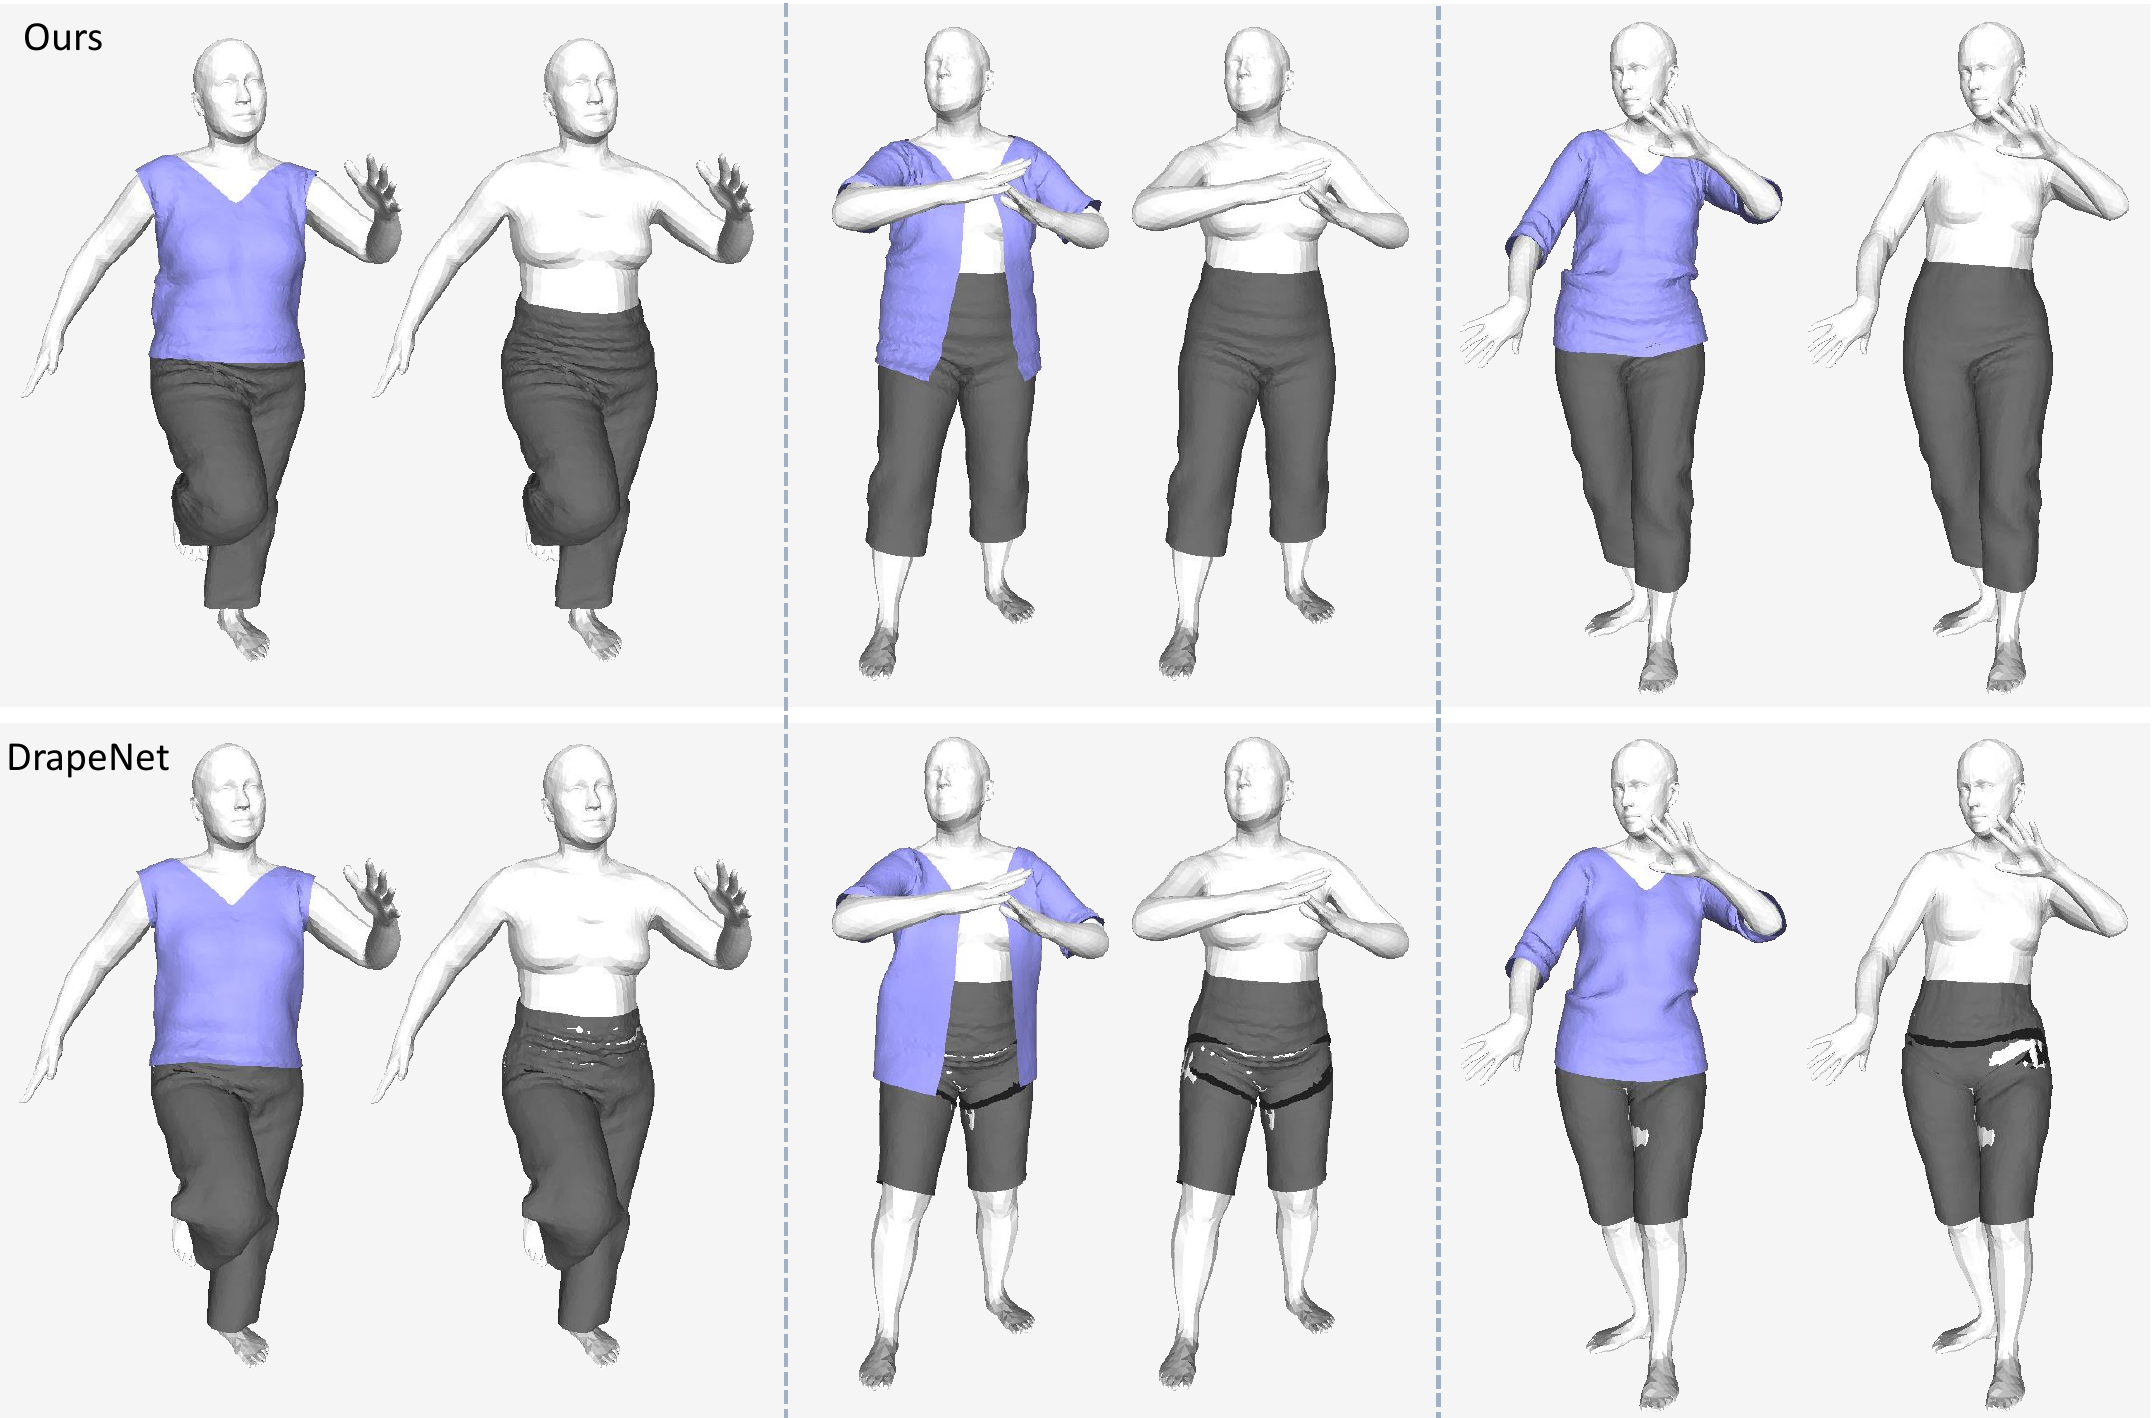}
    %\vspace{-0.35cm}
    \caption{The comparison of draping results of our method and DrapeNet.}
    \label{fig:supp_drapenet_ours}
    %\vspace{-0.45cm}
\end{figure} 
% !TEX root = ../top.tex
% !TEX spellcheck = en-US

\begin{figure}[ht!]
    \centering
    \includegraphics[width=0.99\textwidth]{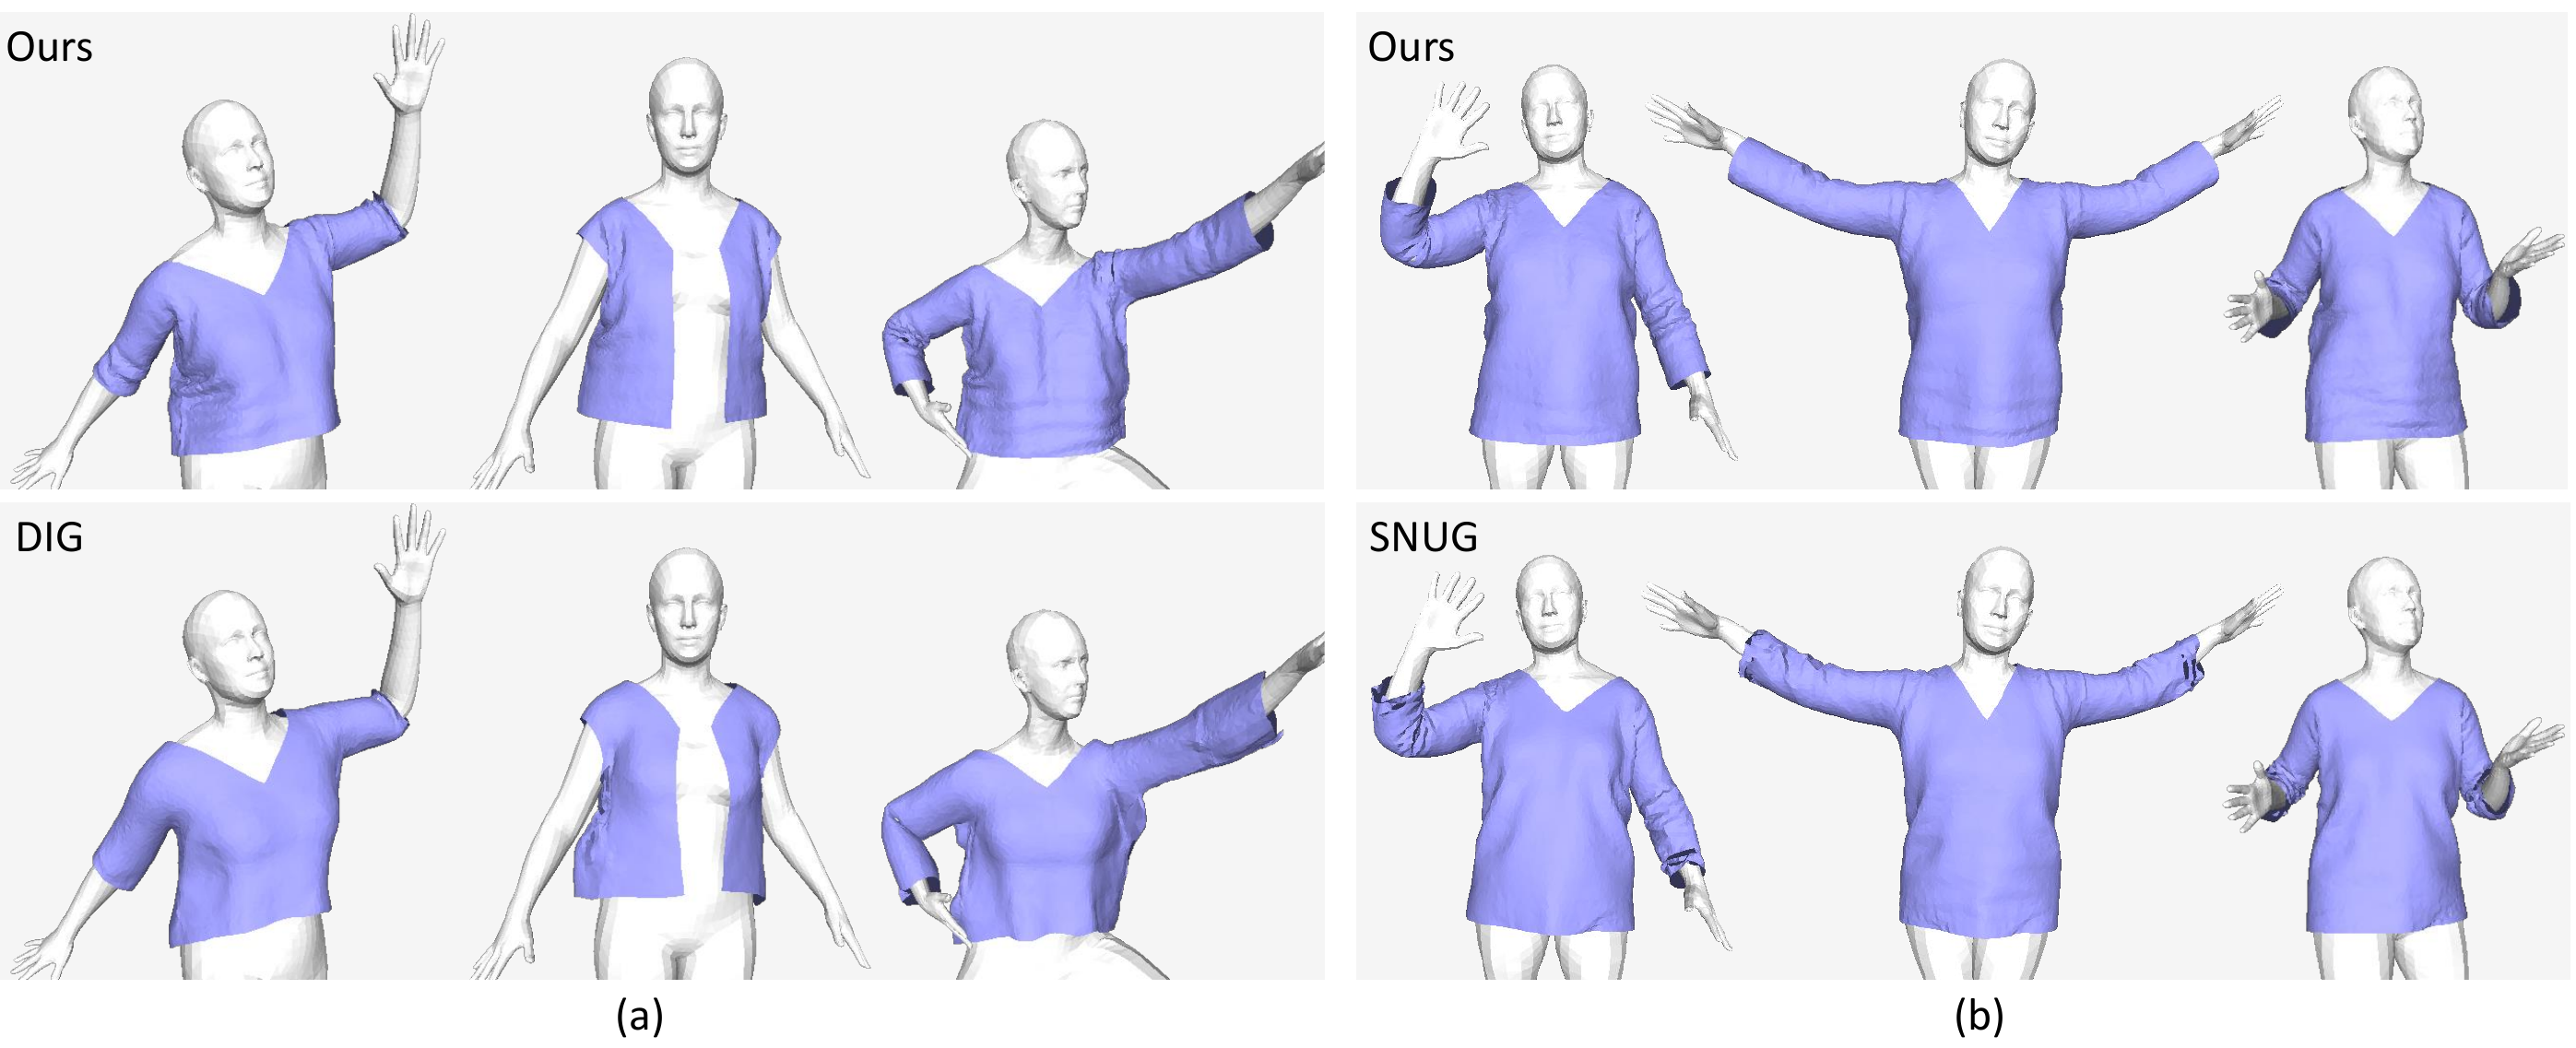}
    %\vspace{-0.35cm}
    \caption{The comparison of draping results for (a) our method vs. DIG, and (b) our method vs. SNUG.}
    \label{fig:supp_dig_snug_ours}
    %\vspace{-0.45cm}
\end{figure} 
Fig.~\ref{fig:supp_drapenet_ours} and Fig.~\ref{fig:supp_dig_snug_ours}(a) present additional comparisons of draping results for our method, DIG~\cite{Li22c} and DrapeNet~\cite{DeLuigi23}. Our results show higher fidelity and fewer artifacts compared to the other methods. We also compare our method with SNUG~\cite{Santesteban22}, a self-supervised method that relies on mesh templates for garment representation and trains one network for each clothing item. In Fig.~\ref{fig:supp_dig_snug_ours}(b), we show the qualitative results on the same shirt. Our results are either comparative or visually superior to those of SNUG, despite using a single draping network for a whole garment category.

\subsection{Multi-Layer Draping}
\label{supp:multilayer_draping_results}
To assess the effectiveness of our multi-layering model, we conducted an experiment to measure the intersection ratio between different layers of garments, and between the garments and the body. We used the 673 unseen poses from the test set of AMASS dataset \cite{Mahmood19} and 673 shape parameters uniformly sampled from the continuous space of $[-2, 2]^{10}$ to generate 673 unique unseen bodies. For each body, we randomly generated five unseen garments (one skirt or one pair of trousers, with four shirts) by interpolating the garment latent codes and draped them on the body. The first layer contained the skirt or trousers, while the shirts were on the following layers. 

The corresponding results are shown in \Cref{tab:collisions_skirt,tab:collisions_trousers}, where the diagonal values represent the intersection ratio between the body and the $i$-th ($i=1,2,3,4,5$) layer, and the other values represent the intersection between different layers of garments. It is important to note that we cannot fairly compare these numbers to any other method, as they do not support layering. The left and right sides of the tables correspond to the results obtained with and without the layering procedure, respectively. As shown in the tables, the significantly lower intersection ratios on the left side demonstrate the effectiveness of our model in handling intersections with the body and between different garments. Another noteworthy observation is that the intersections tend to increase as we layer more garments. This behavior is explained in \Cref{supp:garment_draping}, where we clarify that our multi-layer draping model $\mathcal{D}_m$ is trained solely on garments obtained through single-layer draping, which are relatively close to the body. However, it is worth mentioning that even after five layers, the intersections still remain at a low level ($\sim$2\%).

% !TEX root = ../top.tex
% !TEX spellcheck = en-US

\begin{table}[h!]
  \begin{center}
  \scalebox{0.8}{
    \begin{tabular}{c | c | c | c | c | c}
      \toprule
       w/ $\mathcal{D}_m$ & 1 & 2 & 3 & 4 & 5 \\
       \midrule
       1  & 0.000 & 0.067 & 0.001 & 0.000 & 0.000 \\
       2  & - & 0.003 & 0.633 & 0.608 & 0.636 \\
       3  & - & - & 0.028 & 1.224 & 1.158 \\
       4  & - & - & - & 0.019 & 2.449\\
       5  & - & - & - & - & 0.035 \\
      \bottomrule
      \end{tabular}}
      ~~
  \scalebox{0.8}{
    \begin{tabular}{c | c | c | c | c | c}
      \toprule
       w/o $\mathcal{D}_m$ & 1 & 2 & 3 & 4 & 5 \\
       \midrule
       1  & 0.000 & 0.456 & 0.340 & 0.357 & 0.233 \\
       2  & - & 0.004 & 28.033 & 26.378 & 26.246 \\
       3  & - & - & 0.046 & 24.729 & 24.679 \\
       4  & - & - & - & 0.073 & 27.821\\
       5  & - & - & - & - & 0.052 \\
      \bottomrule
      \end{tabular}}
  \end{center}
  \caption{Evaluation of intersections with the underlying body and between garments on different layers (the 1st layer is a \textbf{skirt}). Left and right are the results of draping with and without the multi-layering network $\mathcal{D}_m$, respectively. The unit is \%.}
  \label{tab:collisions_skirt}
\end{table}

\begin{table}[h!]
  \begin{center}
  \scalebox{0.8}{
    \begin{tabular}{c | c | c | c | c | c}
      \toprule
       w/ $\mathcal{D}_m$ & 1 & 2 & 3 & 4 & 5 \\
       \midrule
       1  & 0.185 & 0.048 & 0.000 & 0.000 & 0.000 \\
       2  & - & 0.003 & 0.631 & 0.588 & 0.637 \\
       3  & - & - & 0.030 & 1.227 & 1.161 \\
       4  & - & - & - & 0.020 & 2.426\\
       5  & - & - & - & - & 0.028 \\
      \bottomrule
      \end{tabular}}
      ~~
  \scalebox{0.8}{
    \begin{tabular}{c | c | c | c | c | c}
      \toprule
       w/o $\mathcal{D}_m$ & 1 & 2 & 3 & 4 & 5 \\
       \midrule
       1  & 0.185 & 0.225 & 0.259 & 0.223 & 0.134 \\
       2  & - & 0.004 & 28.033 & 26.378 & 26.246 \\
       3  & - & - & 0.046 & 24.729 & 24.679 \\
       4  & - & - & - & 0.073 & 27.821\\
       5  & - & - & - & - & 0.052 \\
      \bottomrule
      \end{tabular}}
  \end{center}
  \caption{Evaluation of intersections with the underlying body and between garments on different layers (the 1st layer is a pair of \textbf{trousers}). Left and right are the results of draping with and without the multi-layering network $\mathcal{D}_m$, respectively. The unit is \%.}
  \label{tab:collisions_trousers}
\end{table}

\section{Technical Details}
\label{supp:technical_details}

\subsection{Sewing Patterns for Trousers and Skirts}
\label{supp:sewing_patters}
% !TEX root = ../top.tex
% !TEX spellcheck = en-US

\begin{figure}[ht!]
    \centering
    \includegraphics[width=0.99\textwidth]{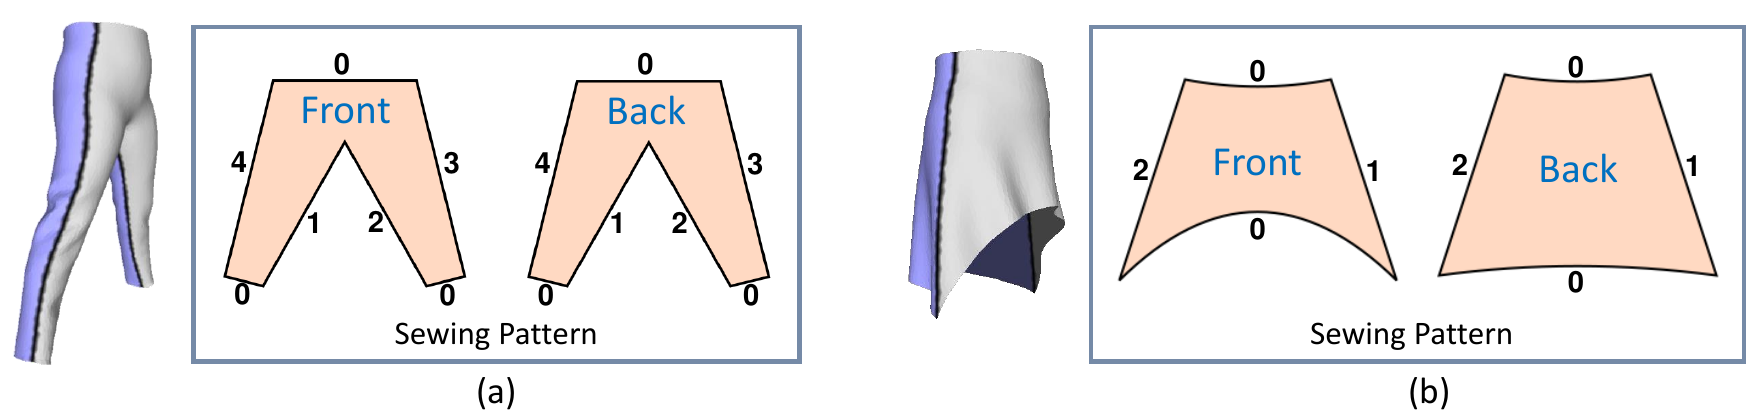}
    %\vspace{-0.35cm}
    \caption{The sewing patterns for (a) trousers and (b) skirts. The front mesh surfaces are in gray and the back ones in blue.}
    \label{fig:supp_pattern}
    %\vspace{-0.45cm}
  \end{figure} 
In Fig. \ref{fig:supp_pattern}, we show the sewing patterns used in our experiments for trousers and skirts.

\subsection{Mesh Triangulation}
\label{supp:mesh_triangulation}
% !TEX root = ../top.tex
% !TEX spellcheck = en-US

\begin{figure}[ht!]
    \centering
    \includegraphics[width=0.99\textwidth]{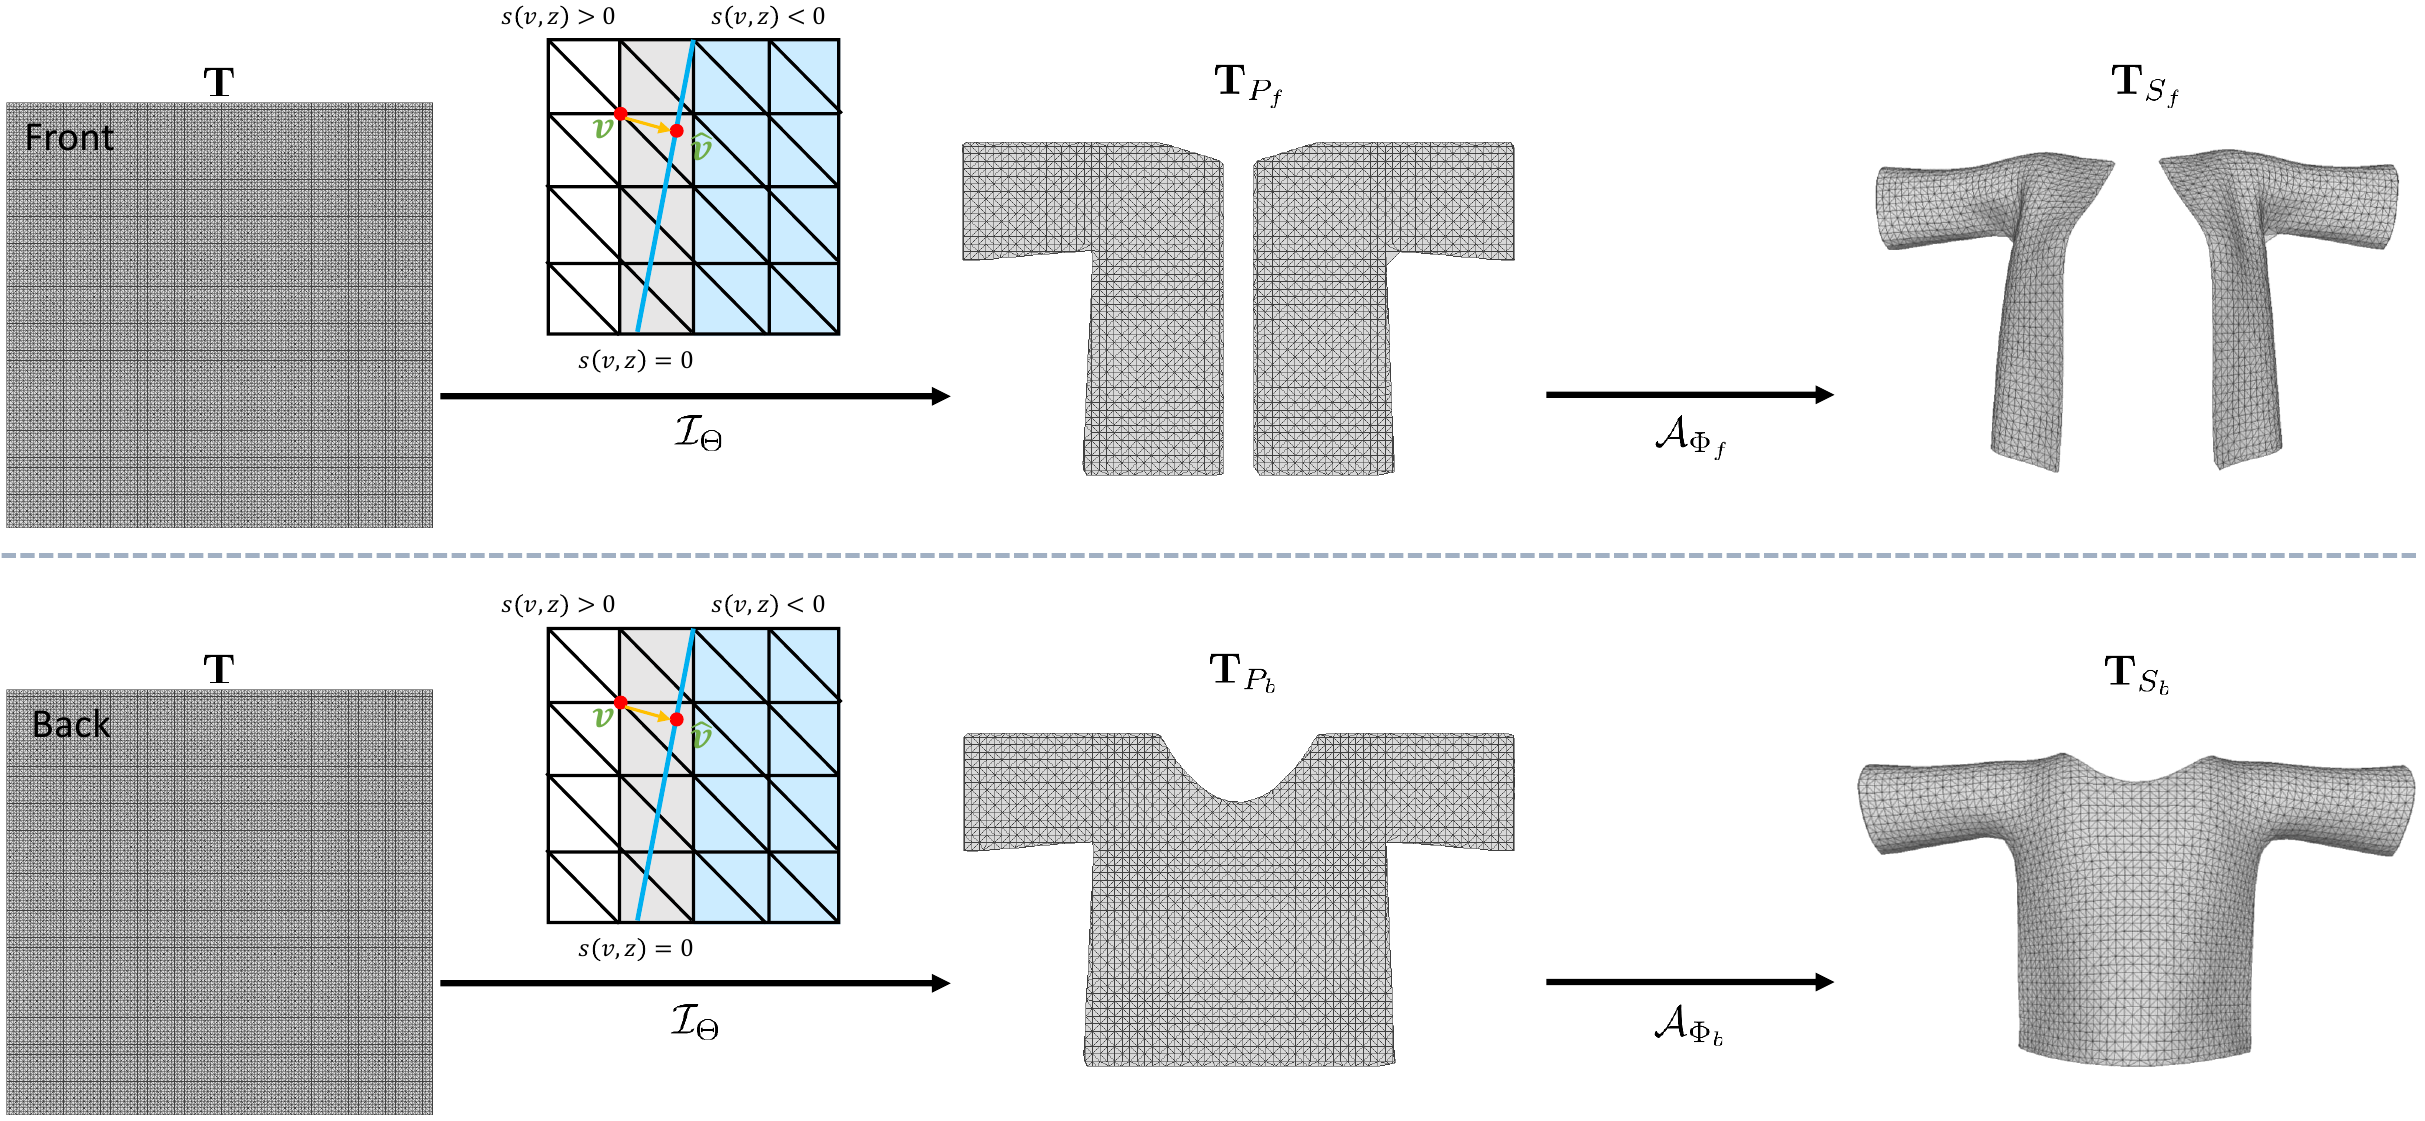}
    %\vspace{-0.35cm}
    \caption{\textbf{Meshing Process.} Starting with a square 2D mesh $\mathbf{T}$, we first extract the front and back panel meshes $\mathbf{T}_{P_f}$ and $\mathbf{T}_{P_b}$ using the implicit function $\mathcal{I}_{\Theta}$. Then we lift $\mathbf{T}_{P_f}$ and $\mathbf{T}_{P_b}$ to 3D to get the surface meshes $\mathbf{T}_{S_f}$ and $\mathbf{T}_{S_b}$ by querying $\mathcal{A}_{\Phi_f}$ and $\mathcal{A}_{\Phi_b}$ on their vertices respectively.}
    \label{fig:supp_mesh}
    %\vspace{-0.45cm}
\end{figure} 
% !TEX root = ../top.tex
% !TEX spellcheck = en-US

\begin{figure}[ht!]
  \centering
  \includegraphics[width=0.9\textwidth]{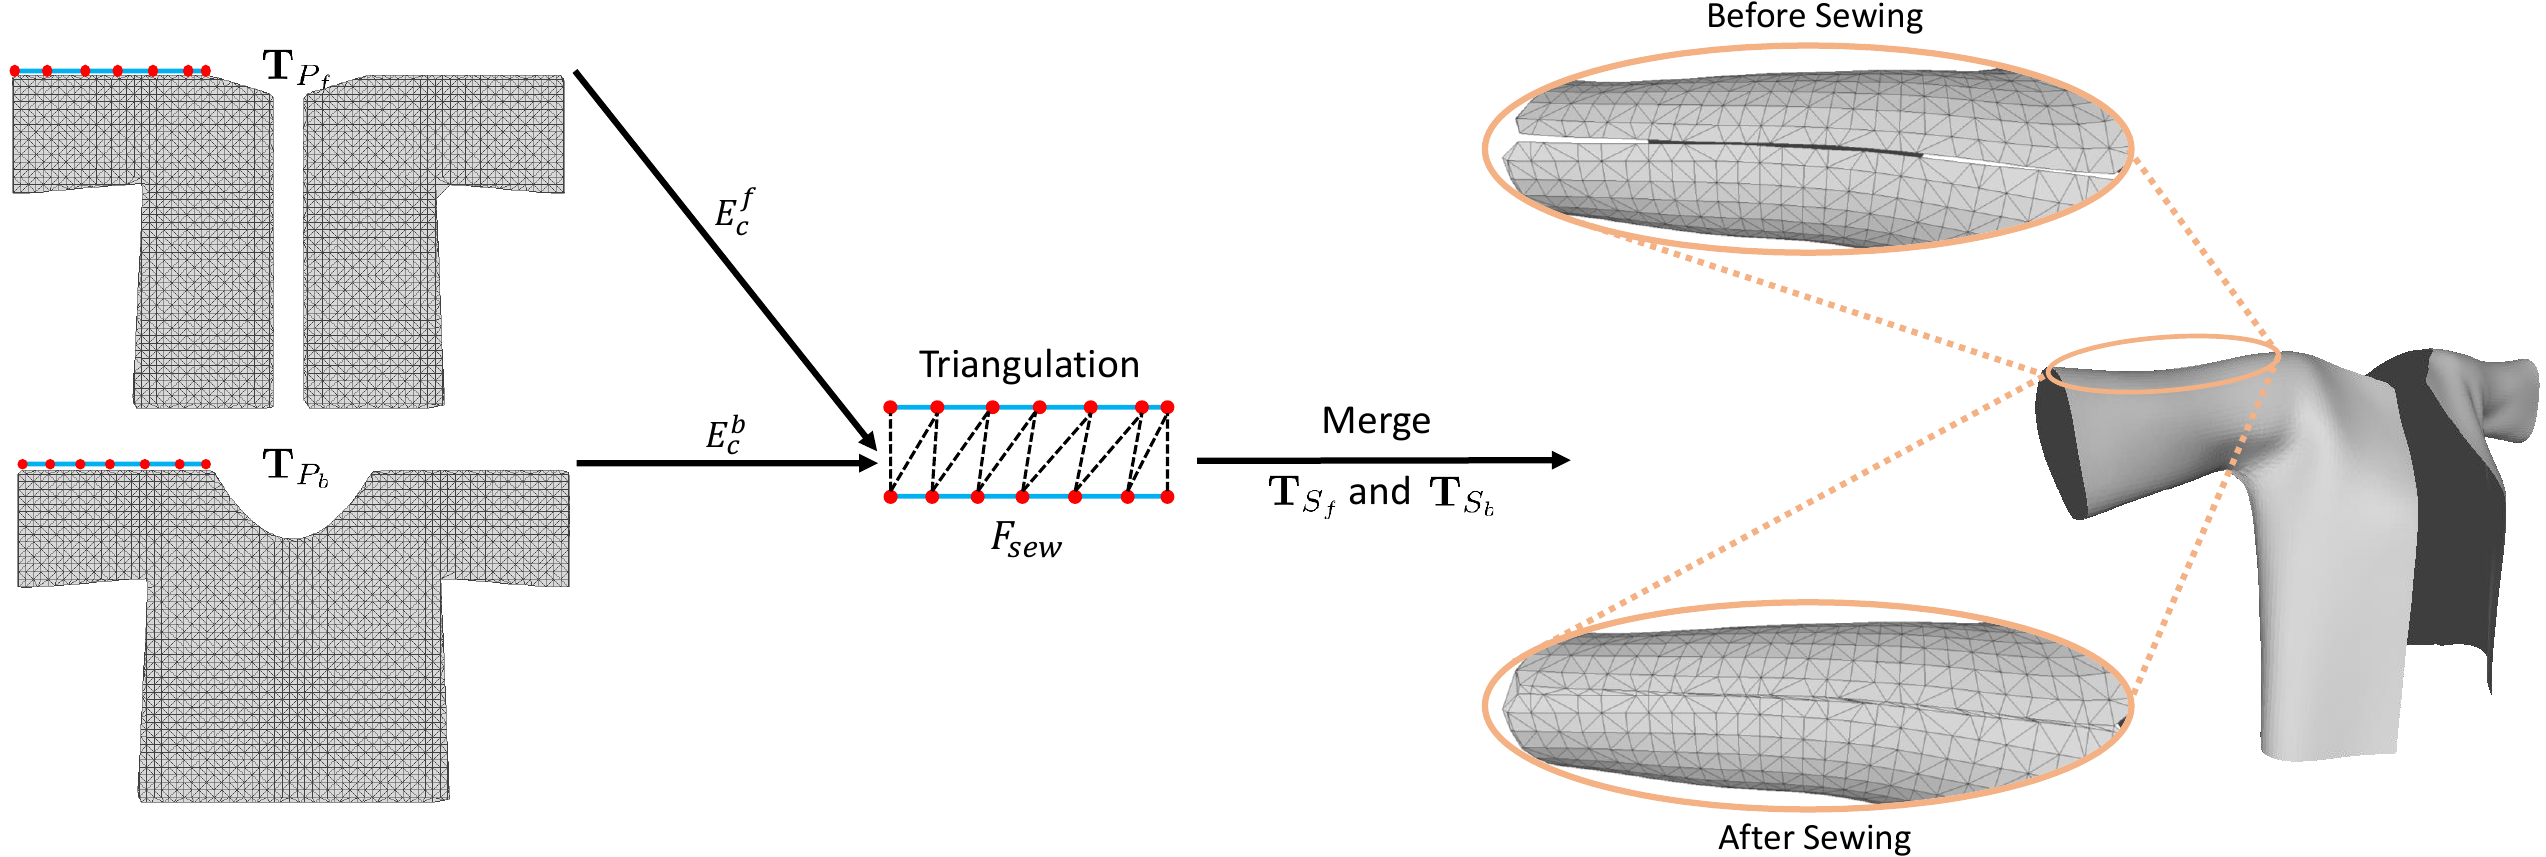}
  %\vspace{-0.35cm}
  \caption{\textbf{Sewing process.} Left: the boundary vertices belonging to the sewing edges $E_c^f$ and $E_c^b$ are marked in red. Middle: The triangulation is performed between $E_c^f$ and $E_c^b$ to create new faces $F_{sew}$. Right: The mesh generated by merging the front and back surfaces $\mathbf{T}_{S_f}$ and $\mathbf{T}_{S_b}$ with $F_{sew}$.}
  \label{fig:supp_sew}
  %\vspace{-0.45cm}
\end{figure} 

In this section, we detail the meshing process of ISP. We first create a square 2D mesh $\mathbf{T}$ for $\Omega$ as shown on the left of Fig.~\ref{fig:supp_mesh}. Given the latent code $\bz$ of a specific garment, for each vertex $v\in V_{\Omega}$, we compute its signed distance value $s$ and edge label $c$ with $(s,c)=\mathcal{I}_{\Theta}(v,\mathbf{z})$.
The 2D front and back panel meshes $\mathbf{T}_{P_f}$ and $\mathbf{T}_{P_b}$ are constructed by keeping vertices of $\mathbf{T}$ with negative signed distance (the blue region of the colored gird in Fig.~\ref{fig:supp_mesh}) and those that have positive signed distance but belong to the edges crossing the 0 iso-level (the gray region of the colored gird in Fig.~\ref{fig:supp_mesh}). For the later ones, we adjust their positions from $v$ to $\hat{v}=v-s(v,\bz)\nabla s(v,\bz)$ to project them to the zero level set (the blue line).
Finally, we query $\mathcal{A}_{\Phi_f}$ and $\mathcal{A}_{\Phi_b}$ on each vertex of $\mathbf{T}_{P_f}$ and $\mathbf{T}_{P_b}$ respectively to lift them to 3D, giving us the front and back surfaces $\mathbf{T}_{S_f}$ and $\mathbf{T}_{S_b}$ as shown on the right of Fig.~\ref{fig:supp_mesh}.

To sew the lifted front and back surfaces $\mathbf{T}_{S_f}$ and $\mathbf{T}_{S_b}$, we perform triangulation with the help of panel meshes $\mathbf{T}_{P_f}$ and $\mathbf{T}_{P_b}$. As illustrated in Fig. \ref{fig:supp_sew}, we group the boundary vertices of $\mathbf{T}_{P_f}$ and $\mathbf{T}_{P_b}$ whose predicted labels are the same ($c$, with $c>0$) to form the sewing edges $E_c^f$ and $E_c^b$ for the front and back panels separately. Then we create faces $F_{sew}$ between the vertices of $E_c^f$ and $E_c^b$, and use $F_{sew}$ to merge the meshes of $\mathbf{T}_{S_f}$ and $\mathbf{T}_{S_b}$, which gives us the final assembled garment mesh.

\subsection{Proof of the Differentiability of ISP}
\label{supp:proof}
According to the \textit{Theorem 1} of \cite{Remelli20b}, for an SDF $s$ and the point $\bx_0$ lying on the 0 iso-level $l=\{\bq|s(\bq,\bz)=0, \bq \in \Omega\}$, we have
\begin{equation}\label{eq:theorem}
    \frac{\partial \bx_0}{\partial s} = -\nabla s(\bx_0,\bz). \;
\end{equation}

For point $\bx$ lying on the $\alpha$ iso-level, we can have $s(\bx,\bz)=\alpha$, where $\alpha$ is a constant. Let $s_\alpha=s-\alpha$, then $\bx$ lies on the 0 iso-level of $s_\alpha$. Based on Eq. \ref{eq:theorem}, we can have
\begin{equation}\label{eq:alpha}
    \frac{\partial \bx}{\partial s_\alpha} = -\nabla s_\alpha(\bx,\bz) = -\nabla s(\bx,\bz). \;
\end{equation}

Assume $v$ is a vertex of the mesh $\mathbf{T}_G$ reconstructed by ISP and $\bx$ is the point on the UV space that satisfies $v=\mathcal{A}_{\Phi}(\bx,\bz)$, then it holds that
\begin{align}
    \frac{\partial v}{\partial\bz} &= \frac{\partial\mathcal{A}_{\Phi}}{\partial \bz}(\bx,\bz) + \frac{\partial\mathcal{A}_{\Phi}}{\partial \bx} \frac{\partial \bx}{\partial \bz}(\bx,\bz), \; \\
    &= \frac{\partial\mathcal{A}_{\Phi}}{\partial \bz}(\bx,\bz) + \frac{\partial\mathcal{A}_{\Phi}}{\partial \bx} \frac{\partial \bx}{\partial s_\alpha} \frac{\partial s_\alpha}{\partial s} \frac{\partial s}{\partial \bz}(\bx,\bz). \; \label{eq:derive}
\end{align}
Since $\frac{\partial s_\alpha}{\partial s}=1$, we can substitute Eq. \ref{eq:alpha} into Eq. \ref{eq:derive} to derive that
\begin{equation}
    \frac{\partial v}{\partial\bz} = \frac{\partial\mathcal{A}_{\Phi}}{\partial \bz}(\bx,\bz) - \frac{\partial\mathcal{A}_{\Phi}}{\partial \bx} \nabla s(\bx,\bz) \frac{\partial s}{\partial \bz}(\bx,\bz). \;
\end{equation}

\subsection{Garment Draping}
\label{supp:garment_draping}
% !TEX root = ../top.tex
% !TEX spellcheck = en-US

\begin{figure}[ht!]
	\centering
		\begin{minipage}{.40\textwidth}
				\centering
		% \vspace{1mm}
		\includegraphics[width=0.99\textwidth]{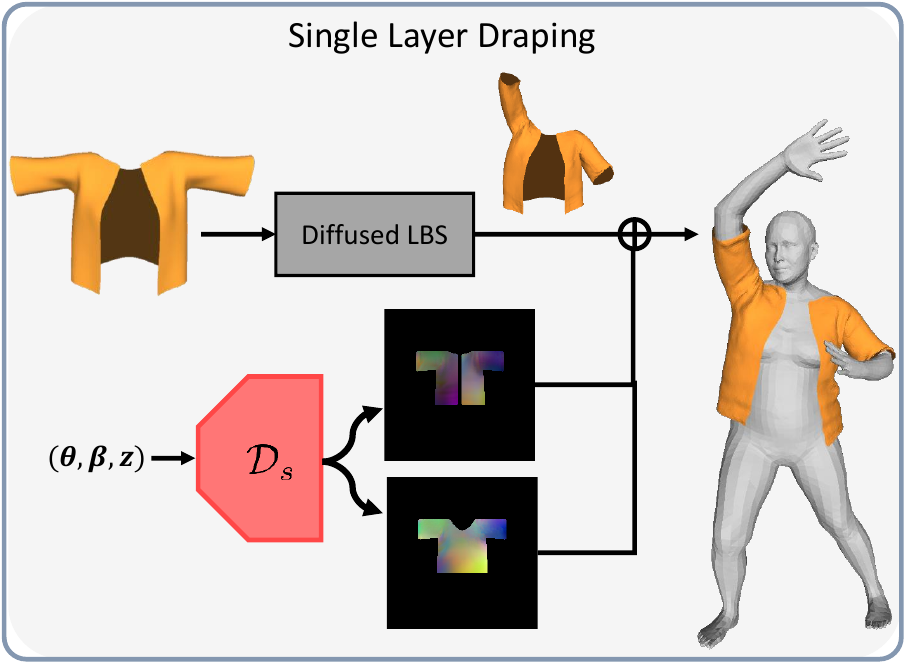}
		% \vspace{-7mm}
		\captionof{figure}{\textbf{Single layer draping.} The rest-state garment is first deformed by the diffused LBS to get the initial shape, and then refined by the displacement maps predicted by $\mathcal{D}_s$. }
		\label{fig:supp_pipD}
	\end{minipage}
	% \hspace{0mm}
    ~
	\begin{minipage}{.58\textwidth}
		\centering
		\includegraphics[width=.99\textwidth]{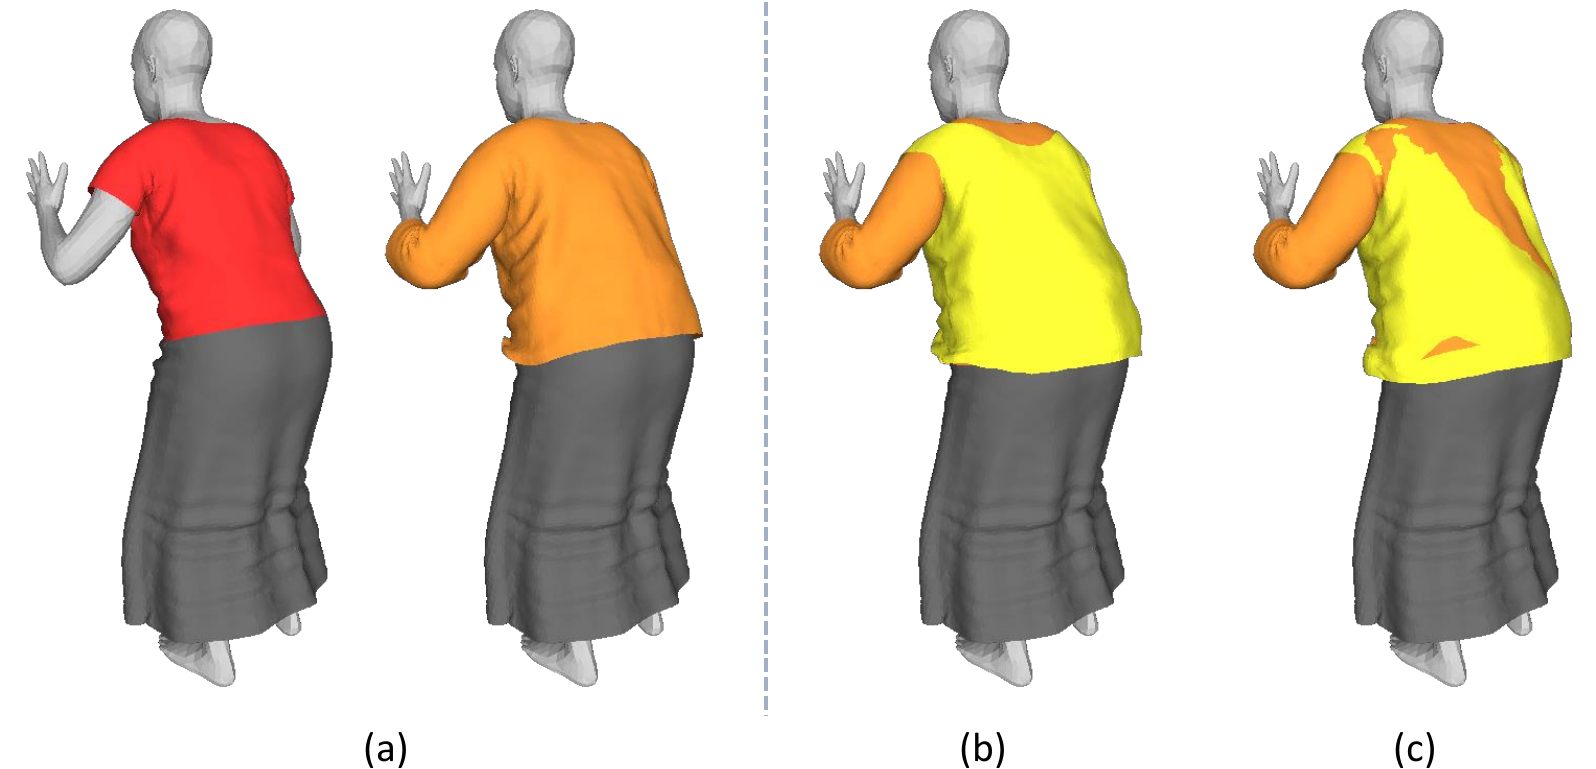}
		% \vspace{-10pt}
		\captionof{figure}{\textbf{Layering.} (a) We drape a red and an orange shirts on the body. A third one (yellow) is draped by (b) Algorithm \ref{alg:mld} and (c) by naively applying $\mathcal{D}_m$ to it.}
		\label{fig:supp_layer}
	\end{minipage}%
    \vspace{-0.45cm}
\end{figure}

\iffalse
\begin{figure}
    \centering
    \includegraphics[width=0.99\textwidth]{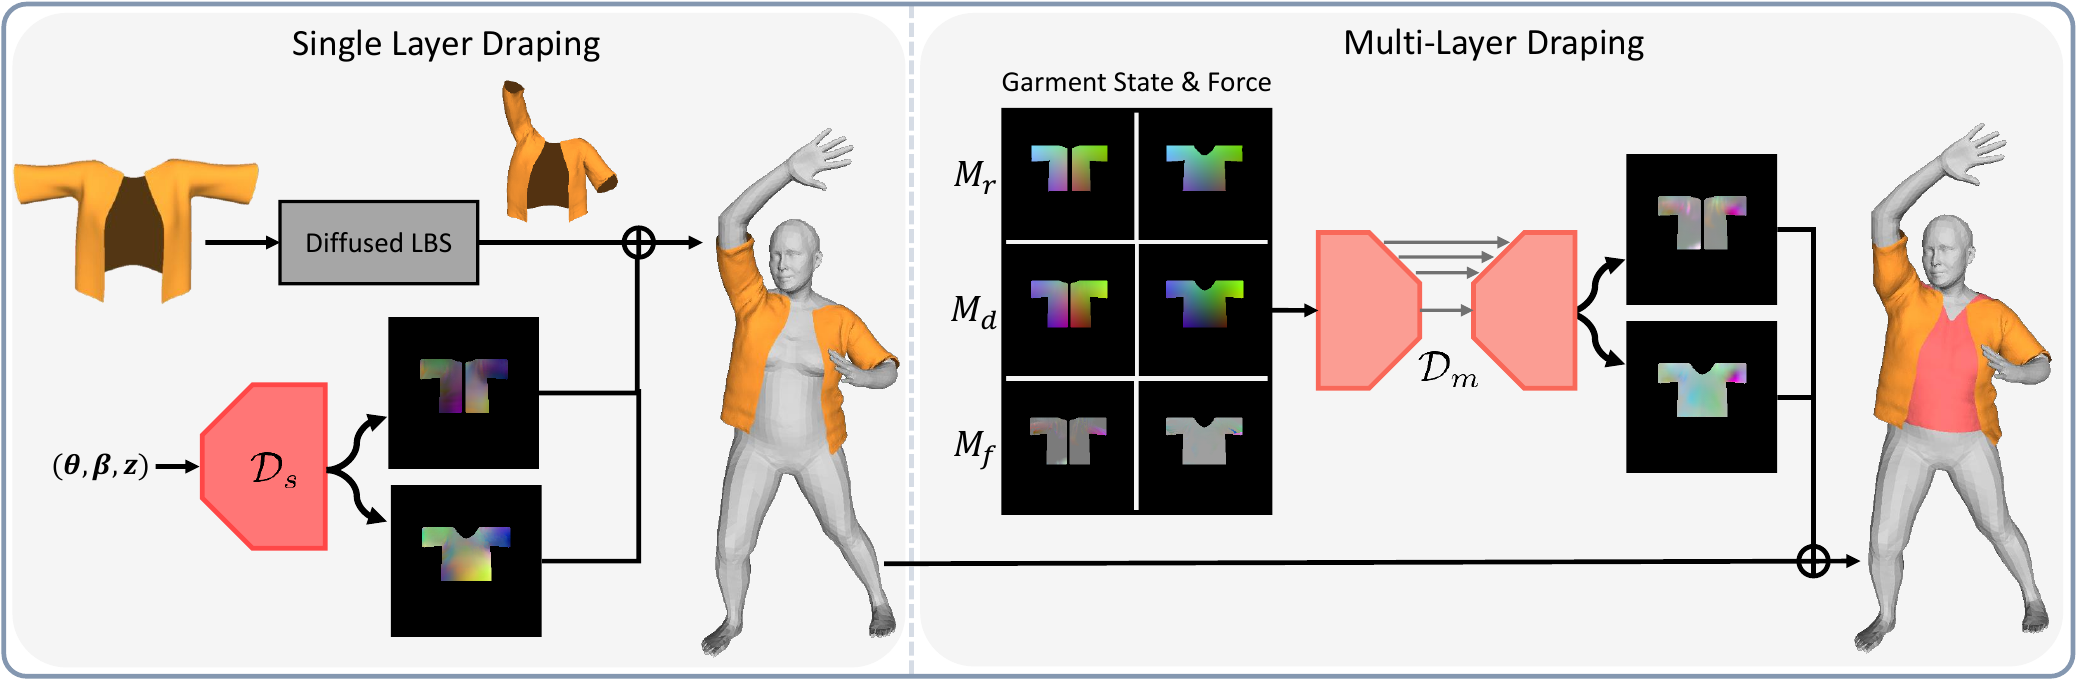}
    %\vspace{-0.35cm}
    \caption{\textbf{The pipeline of garment draping}. We first apply the network $\mathcal{D}_s$ to drape single garments. By utilizing the garment geometry and forces encoded in the input UV maps, we then rely on the network $\mathcal{D}_m$ to resolve garment intersections for multi-layered draping.}
    \label{fig:supp_pipD}
    %\vspace{-0.45cm}
\end{figure} 
\fi
%\input{figs/supp_layer}
\paragraph{Single Layer Draping.}
In Fig. \ref{fig:supp_pipD}, we illustrate the pipeline for the single layer draping, which relies on the diffused LBS of SMPL \cite{Loper15} to get the initial rough estimate of the garment shape and the displacement map output by $\mathcal{D}_s$ to refine it. 

\paragraph{Multi-Layer Draping.}
\label{supp:multilayer_draping}
Our layering network $\mathcal{D}_m$ can be applied to multiple garments iteratively to resolve collisions between them. More specifically, consider $K$ garments $[G_1, G_2,...,G_K]$ that are already draped individually by single layer draping network $\mathcal{D}_s$. Their subscripts denote their draping order, with smaller ones being closer to the body. We can obtain their rest state maps $[M_r^1, M_r^2,...,M_r^K]$ as described in Sec.~3.2 of the main paper, and apply Algorithm \ref{alg:mld} for layering them by iterating on garments following their draping order. 
%For each one, it solves intersections with all subsequent garments. 
\begin{algorithm}
    \SetKwFunction{ForceMap}{ForceMap}
    %\SetKwFunction{RestStateMap}{RestStateMap}
    \SetKwFunction{PositionMap}{PositionMap}
    \SetKwInOut{Input}{Input}\SetKwInOut{Output}{Output}\SetKwInOut{Require}{Require}
    \Require{Function \ForceMap{$a$, $b$} that computes the force map for $a$ by taking $b$ as the underlying layer; Function \PositionMap{$a$} that computes the 2D position map of $a$; Layering network $\mathcal{D}_m$.}
    \Input{An ordered set of garments $[G_1, G_2,...,G_K]$; Rest state maps for each garemnts $[M_r^1, M_r^2,...,M_r^K]$.}
    \Output{Layered garments $\{\tilde{G_1}, \tilde{G_2},...,\tilde{G_K}\}$ without intersections.}
    \BlankLine
    \For{$i\leftarrow 1$ \KwTo $K$}{
        $\tilde{G_i} \leftarrow G_i$\;
        \For{$j\leftarrow i+1$ \KwTo $K$}{
            $M_f^j$ $\leftarrow$ \ForceMap{$G_j$, $\tilde{G_i}$} \tcc*[r]{Eq.~(9) in the main paper}
            $M_d^j$ $\leftarrow$ \PositionMap{$G_j$}\;
            Update vertex positions of $G_j$ by $\mathcal{D}_{m}(M_r^j, M_d^j, M_f^j)$ \;
    }
    }
    \caption{Multi-layer Draping}\label{alg:mld}
\end{algorithm}

Note that we only train $\mathcal{D}_{m}$ on \textit{one} pair of garments individually draped by $\mathcal{D}_{s}$. Therefore, it can only resolve the intersections happening at the same layer, which leads to an extra inner loop in Algorithm \ref{alg:mld} that moves all the subsequent garments to the same $j$-th layer. Otherwise, intersections cannot be completely resolved when applying $\mathcal{D}_{m}$ to two garments lying on the different layers as illustrated in Fig.~\ref{fig:supp_layer}(c).

\subsection{Recovering Multi-Layered Garments from Images}
\label{supp:recovering_multilayered}
\begin{figure}[ht!]
    \centering
    \includegraphics[width=0.99\textwidth]{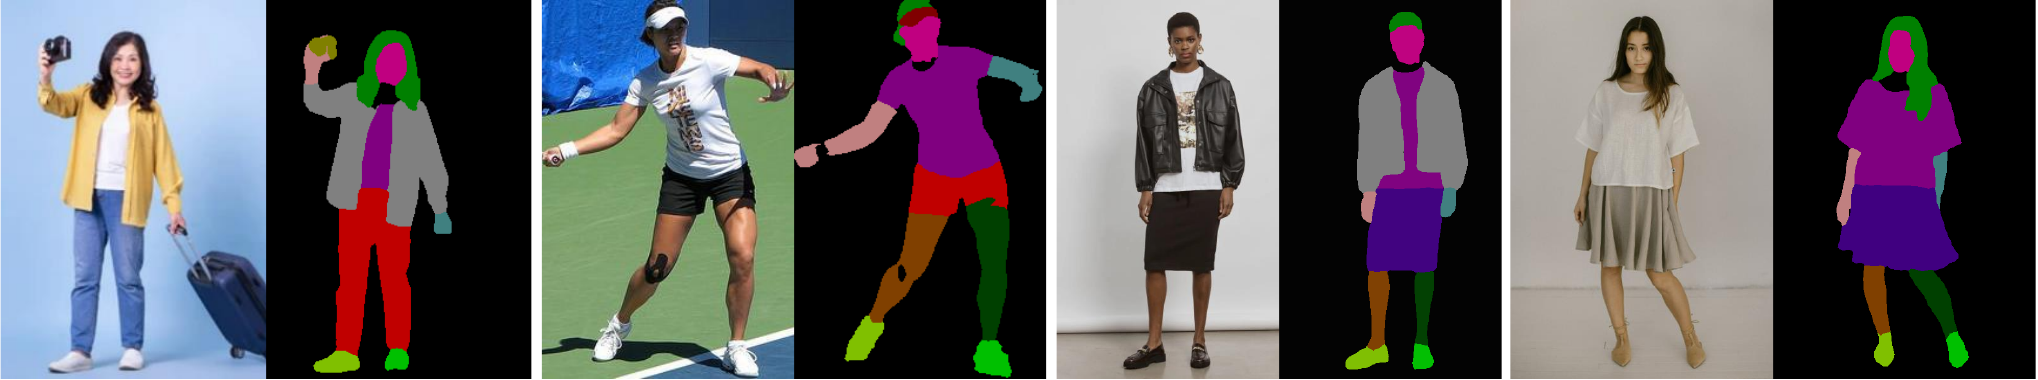}
    %\vspace{-0.35cm}
    \caption{Segmentation masks obtained from \cite{Li20i}. Jackets are marked in gray, shirts in purple, skirts in dark purple, trousers in red, and body parts in other colors.}
    \label{fig:supp_seg}
    %\vspace{-0.45cm}
\end{figure} 
In Fig. \ref{fig:supp_seg}, we show the segmentation masks used for the optimization in Eq.~(11) in the main paper. The optimization is performed from the outer garment to the inner one, i.e., jacket (if detected) $\rightarrow$ shirt $\rightarrow$ trousers (or skirt). More specifically, for the first example shown in Fig. \ref{fig:supp_seg}, we have the detected segmentation mask $\mathbf{S}_1$, $\mathbf{S}_2$ and $\mathbf{S}_3$ for the jacket, the shirt and the trousers respectively. We first initialize a latent code $\bz_1$ for the jacket and perform the following optimization to recover its mesh 
\begin{equation}\label{eq:fit1}
    \bz^*_{1} = \arg\min_{\bz_{1}} L_{\text{IoU}}(R(\mathcal{G}(\Beta,\Teta,\bz_{1})\oplus\mathcal{M}(\Beta,\Teta)), \mathbf{S}_1) \; ,
\end{equation}
\begin{equation}
    \mathcal{G}(\Beta,\Teta,\bz_{1}) = \mathcal{D}(\Beta,\Teta,\bz_1, \bT_G(\bz_1))\; , 
\end{equation}
Note that the rendered mask is obtained by setting the colors of the jacket and the body mesh vertices to white and black respectively. Then we fix $\bz_1$ and initialize a new latent code $\bz_2$ for the shirt and perform
\begin{align}
    \bz^*_{2} &= \arg\min_{\bz_{2}} L_{\text{IoU}}(R(\mathcal{G}(\Beta,\Teta,\bz_{1:2})\oplus\mathcal{M}(\Beta,\Teta)), \mathbf{S}_2) \; , \\
    \mathcal{G}(\Beta,\Teta,\bz_{1:2}) &= \mathcal{D}(\Beta,\Teta,\bz_1, \bT_G(\bz_1))\oplus\mathcal{D}(\Beta,\Teta,\bz_2, \bT_G(\bz_2)), \;
\end{align}
to recover the mesh of the shirt. The optimization for the trousers is similar: fixing $\bz_1$ and $\bz_2$; initializing the latent code $\bz_3$ for the trousers; performing
\begin{align}
    \bz^*_{3} &= \arg\min_{\bz_{3}} L_{\text{IoU}}(R(\mathcal{G}(\Beta,\Teta,\bz_{1:3})\oplus\mathcal{M}(\Beta,\Teta)), \mathbf{S}_3) \; , \\
    \mathcal{G}(\Beta,\Teta,\bz_{1:3}) &= \mathcal{D}(\Beta,\Teta,\bz_1, \bT_G(\bz_1))\oplus\mathcal{D}(\Beta,\Teta,\bz_2, \bT_G(\bz_2))\oplus\mathcal{D}(\Beta,\Teta,\bz_3, \bT_G(\bz_3)). \;
\end{align}

\subsection{Loss Terms, Network Architectures and Training}
\label{supp:loss_terms}
\paragraph{Loss Terms.}
The Chamfer distance loss $\mathcal{L}_{CHD}$ of Eq.~(4) in the main paper  is formulated as
\begin{equation}
    \mathcal{L}_{CHD} = \sum_{\bx \in P} \min_{\bX \in \mathcal{S}} || \mathcal{A}_{\Phi}(\bx,\bz)-\bX ||_2^2 + \sum_{\bX \in \mathcal{S}} \min_{\bx \in P} || \mathcal{A}_{\Phi}(\bx,\bz),\bX ||_2^2, \;
\end{equation}
where $P$ is the panel and $\mathcal{S}$ is the ground truth surface mesh.

The normal consistency loss $\mathcal{L}_{normal}$ of Eq.~(4) in the main paper is formulated as
\begin{equation}
    \mathcal{L}_{normal} = \sum_{\bx \in Fc_P} (1 - n_f(\mathcal{A}_{\Phi}(\bx,\bz))\cdot \bn_{\bX^*}) + \sum_{\bX \in Fc_\mathcal{S}} (1 - n_f(\mathcal{A}_{\Phi}(\bx^*,\bz))\cdot \bn_{\bX}), \;
\end{equation}
\begin{equation}
    \bX^* = \argmin_{\bX \in Fc_\mathcal{S}} ||\bX-\mathcal{A}_{\Phi}(\bx,\bz)||_2, ~~ \bx^* = \argmin_{\bx \in Fc_P} ||\bX-\mathcal{A}_{\Phi}(\bx,\bz)||_2 \;
\end{equation}
where $Fc_P$ and $Fc_\mathcal{S}$ are the face centers of the panel mesh and the surface mesh, and $\bn_{\bX}$ represents the normal of $\bX$. $n_f(\cdot)$ is the function that computes the normal for the face that $\mathcal{A}_{\Phi}(\bx,\bz)$ belongs to.

\paragraph{Network Architectures.} 
For each garment category, i.e. shirts, skirts, and trousers, we train one separate set of networks $\{\mathcal{I}_{\Theta},\mathcal{A}_{\Phi},\mathcal{D}_s\}$. $\mathcal{D}_m$ is shared by all garment categories. Our models are implemented as the following.
\begin{itemize}
    \item \underline{Pattern parameterization network $\mathcal{I}_{\Theta}$:} We use two separate networks $\mathcal{I}_{\Theta_f}$ and $\mathcal{I}_{\Theta_b}$ to learn the pattern parameterization for the front and back panels. Each of them is implemented as an MLP with Softplus activations.
    \item \underline{UV parameterization network $\mathcal{A}_{\Phi}$:} We use two separate networks $\mathcal{A}_{\Phi_f}$ and $\mathcal{A}_{\Phi_b}$ to learn the UV parameterization for the front and back surfaces. Both of them have the same architecture, which is a 7-layer MLP with a skip connection from the input layer to the middle and Softplus activations.
    \item \underline{Latent code $\bz$:} The dimension is 32.
    \item \underline{Diffuse skinning weight model $w$:} A 9-layer MLP with leaky ReLU activations and an extra Softmax layer at the end to normalize
    the output.
    \item \underline{Displacement network $\mathcal{D}_s$:} A 10-layer MLP with a skip connection from the input layer to the middle and leaky ReLU activations.
    \item \underline{Layering network $\mathcal{D}_m$:} A U-Net with 4 convolution blocks and 4 deconvolution blocks.
\end{itemize}

\paragraph{Training.} 
We use the Adam \cite{Kingma15} optimizer for training our networks. The batch sizes, the learning rates and the numbers of iterations for training are summarized in Table. \ref{tab:training}. The hyperparameters of the training losses are summarized in Table. \ref{tab:parameters}. $\mathcal{I}_{\Theta}$, $\mathcal{A}_{\Phi}$, $w$ and $\mathcal{D}_m$ are trained with a TESLA V100 GPU, while $\mathcal{D}_s$ is trained with 3 GPUs. During the training of $\mathcal{D}_m$, we randomly select two garments as the outer and inner layers, and let the model learn to resolve intersections between them.
% !TEX root = ../top.tex
% !TEX spellcheck = en-US

\begin{table}
    \begin{center}
      \scalebox{1.}{
            \begin{tabular}{c | c | c | c | c | c}
            \toprule
             Network & $\mathcal{I}_{\Theta}$ & $\mathcal{A}_{\Phi}$ & $w$ & $\mathcal{D}_s$ & $\mathcal{D}_m$ \\
             \midrule
             Learning Rate  & $10^{-4}$ & $10^{-4}$ & $10^{-4}$ & $5\times 10^{-5}$ & $10^{-4}$ \\
             Batch Size  & 50 & 50 & 6000 & 30 & 6\\
             Iterations  & 70000 & 70000 & 2000 & 20000 & 30000 \\
            \bottomrule
            \end{tabular}
            }
      \end{center}
      %\vspace{-0.5cm}
      \caption{Training hyperparameters.}
      \label{tab:training}
      %\vspace{-6mm}
      %\vspace{-0.5cm}
  \end{table}
  
% !TEX root = ../top.tex
% !TEX spellcheck = en-US
  
\begin{table}
    \begin{center}
        \begin{tabular}{c|cc|cc|ccc}
        \toprule
        \multirow{2}{*}{Loss} &
            \multicolumn{2}{c|}{$\mathcal{L}_{\mathcal{I}}$} &
            \multicolumn{2}{c|}{$\mathcal{L}_{\mathcal{A}}$} &
            \multicolumn{3}{c}{$\mathcal{L}_{\mathcal{D}_m}$} \\
            & $\lambda_{CE}$ & $\lambda_{reg}$ & $\lambda_{n}$ & $\lambda_{c}$ & $\lambda_{g}$ & $\lambda_{r}$ & $\epsilon$ \\
            \midrule
        Value & 0.01 & 0.001 & 0.01 & 1 & 0.5 & 1 & 0.005 \\
        \bottomrule
        \end{tabular}
    \end{center}
    \caption{Training loss hyperparameters for $\mathcal{L}_{\mathcal{I}}$, $\mathcal{L}_{\mathcal{A}}$ and $\mathcal{L}_{\mathcal{D}_m}$.
    }
    \label{tab:parameters}
\end{table}

\section{Extension to Sewing Patterns with More Panels}
\label{supp:extension}
% !TEX root = ../top.tex
% !TEX spellcheck = en-US

\begin{figure}[ht!]
    \centering
    \includegraphics[width=0.99\textwidth]{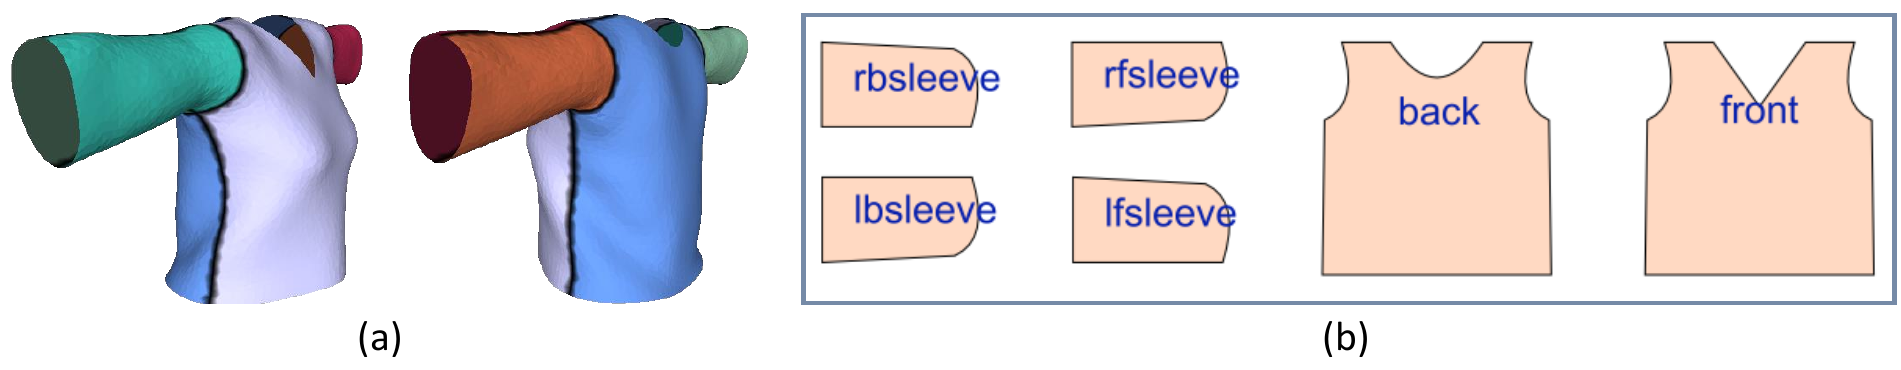}
    %\vspace{-0.35cm}
    \caption{\textbf{The 6-panel sewing pattern}. (a) The 3D mesh surface for a shirt. The corresponding surface for each panel is denoted in different colors. (b) The six 2D panels for the front, the back, the right front/back sleeves and the left front/back sleeves.}
    \label{fig:supp_6_panels}
    %\vspace{-0.45cm}
\end{figure} 
% !TEX root = ../top.tex
% !TEX spellcheck = en-US

\begin{figure}[ht!]
    \centering
    \includegraphics[width=0.99\textwidth]{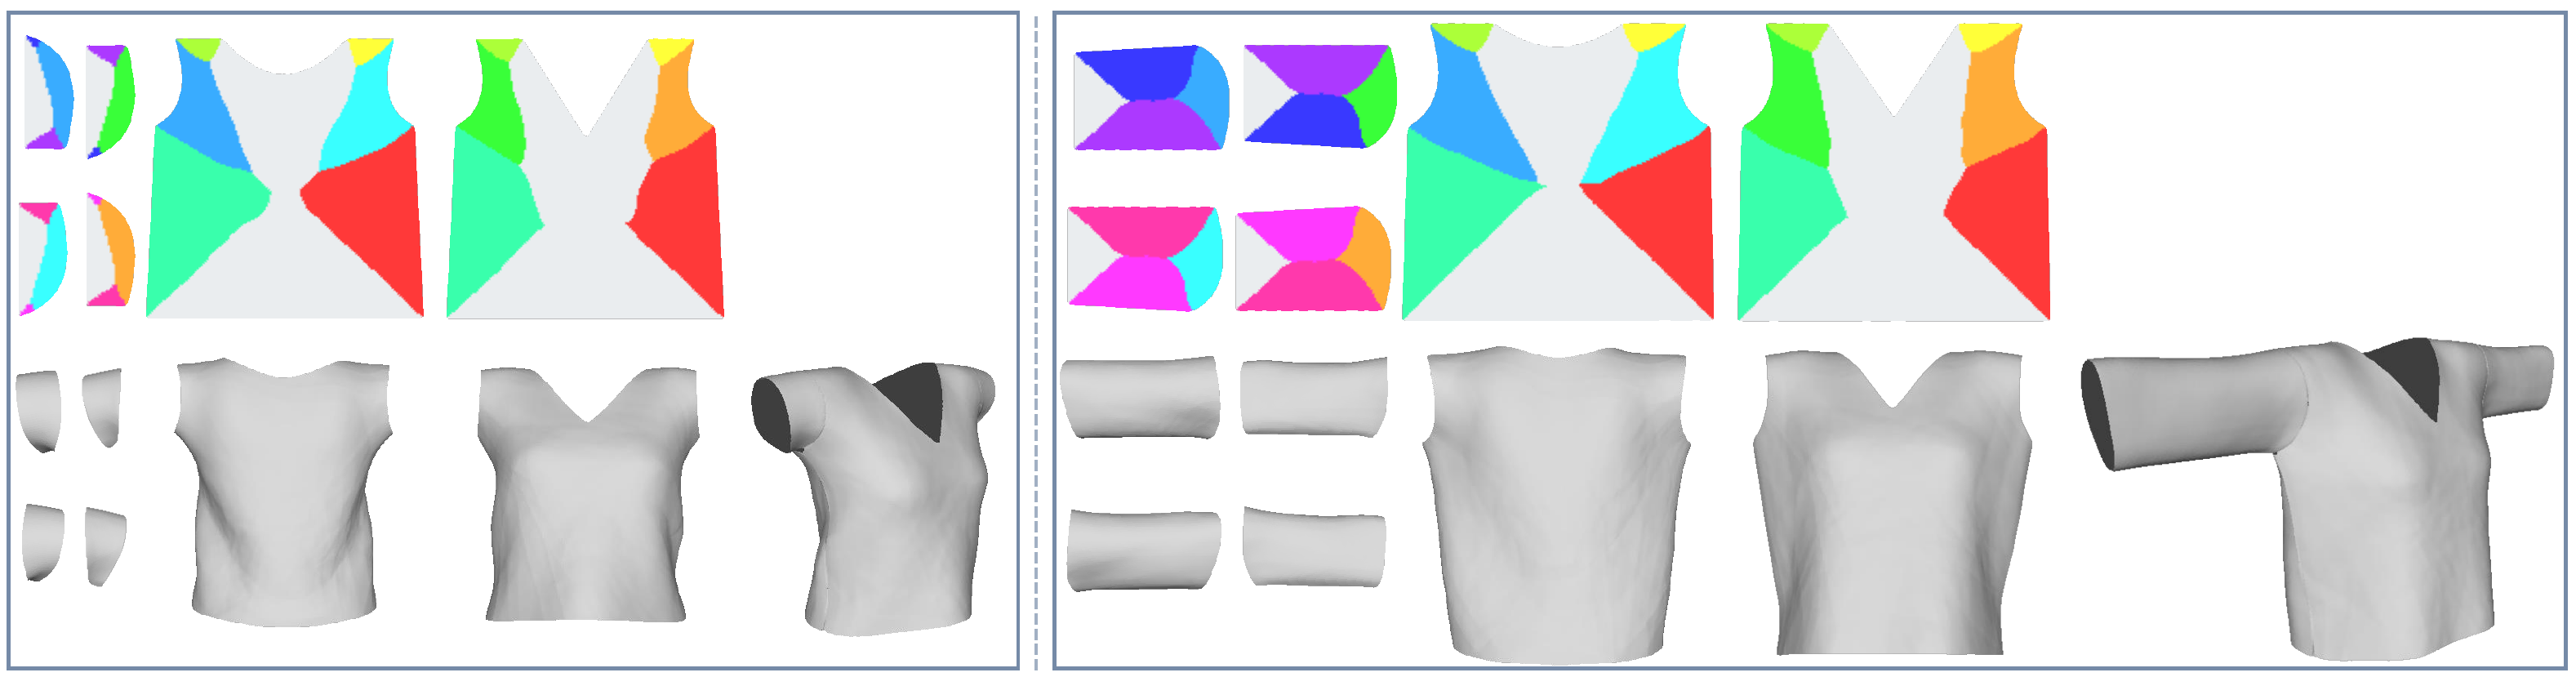}
    %\vspace{-0.35cm}
    \caption{\textbf{Reconstruction with 6 panels}. For both the left and right examples, we show the reconstructed panels on the top and the reconstructed surfaces and the sewed meshes at the bottom. Colors on panels denote edge labels predicted by $\mathcal{I}_{\Theta}$.}
    \label{fig:supp_6_panels_recon}
\end{figure} 
In our experiments, each garment's sewing pattern consists of two panels, the front and the back. However, our ISP can be extended to patterns with any number of panels. For example, we can train $\mathcal{I}_{\Theta}$ and $\mathcal{A}_{\Phi}$ on a database of sewing patterns with six panels as shown in Figure \ref{fig:supp_6_panels}, using the same training protocol described in the main paper. After training, we can use them to reconstruct the panels and surfaces and produce the sewed mesh as illustrated in Fig.~\ref{fig:supp_6_panels_recon}. Adding more panels does not result in better reconstructions. For this reason and for the sake of simplicity, we use a model with 2 panels as our default setting.

\section{Failure Cases}
\label{supp:failure_cases}
\begin{figure}[ht!]
    \centering
    \includegraphics[width=0.99\textwidth]{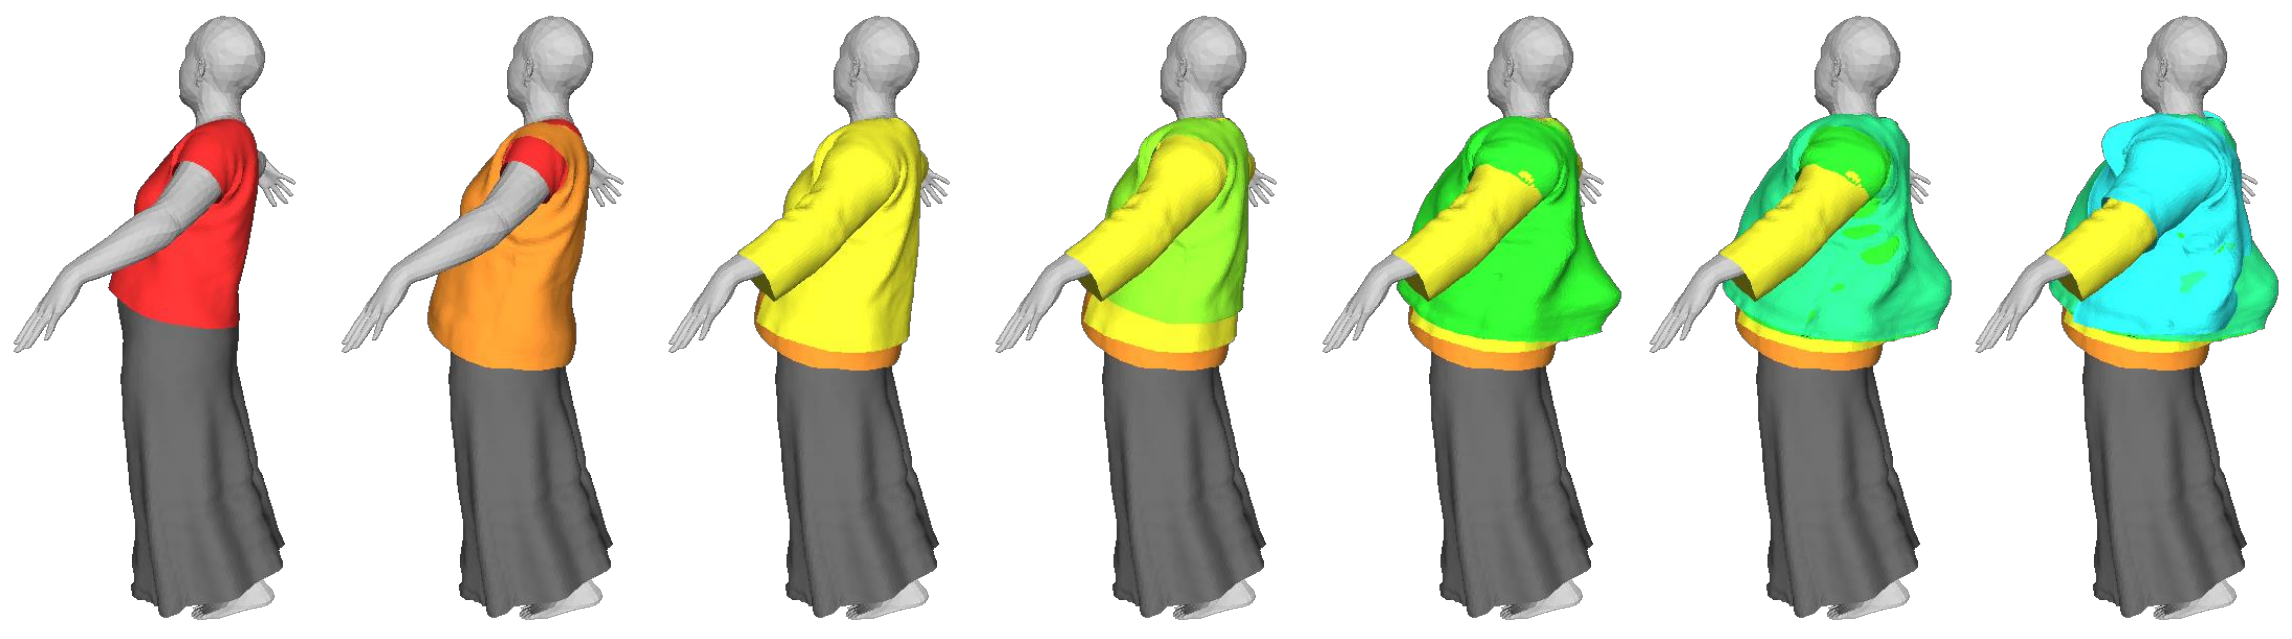}
    %\vspace{-0.35cm}
    \caption{Draping increasingly many shirts: from 1 (left) to 7 (right).}
    \label{fig:failure}
    %\vspace{-0.45cm}
\end{figure} 

Fig.~\ref{fig:failure} presents draping results as the number of shirts increases. We observe that the model produces unrealistic deformation when the number of shirts is greater than four. This behavior occurs because our multi-layer draping model $\mathcal{D}_m$ is only trained on garments obtained by single layer draping as described in Section 3.2 of the main paper. In this scenario, the garments are relatively close to the body. When applied to cases with more shirts (typically over four), the model may generate unpredictable results with the shirts moving far away from the body. However, we note that this issue can be resolved by finetuning the model progressively on layered garments. We also consider that wearing more than four shirts is not a common scenario.
