# Supplementary material for: ISP: Multi-Layered Garment Draping with Implicit Sewing Patterns
Source: arXiv:2305.14100 source file (2023-10-14)
Supplement: Supplementary file 2 [file supp_6_panels.tex]

% !TEX root = ../top.tex
% !TEX spellcheck = en-US

\begin{figure}[ht!]
    \centering
    \includegraphics[width=0.99\textwidth]{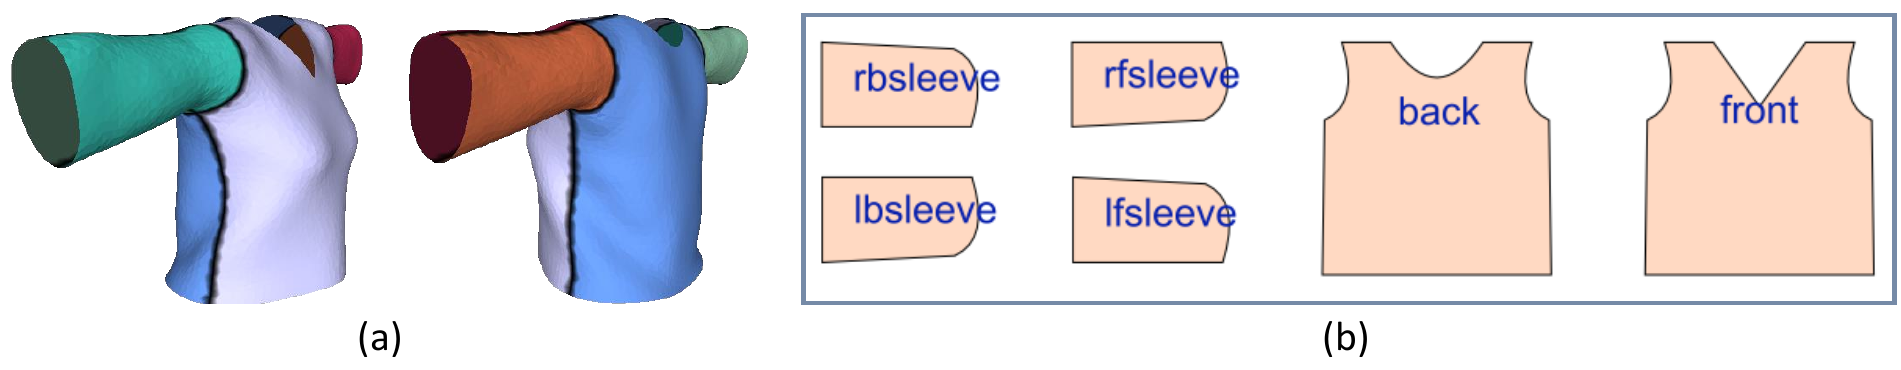}
    %\vspace{-0.35cm}
    \caption{\textbf{The 6-panel sewing pattern}. (a) The 3D mesh surface for a shirt. The corresponding surface for each panel is denoted in different colors. (b) The six 2D panels for the front, the back, the right front/back sleeves and the left front/back sleeves.}
    \label{fig:supp_6_panels}
    %\vspace{-0.45cm}
\end{figure}
