# Supplementary material for: ISP: Multi-Layered Garment Draping with Implicit Sewing Patterns
Source: arXiv:2305.14100 source file (2023-10-14)
Supplement: Supplementary file 3 [file supp_6_panels_recon.tex]

% !TEX root = ../top.tex
% !TEX spellcheck = en-US

\begin{figure}[ht!]
    \centering
    \includegraphics[width=0.99\textwidth]{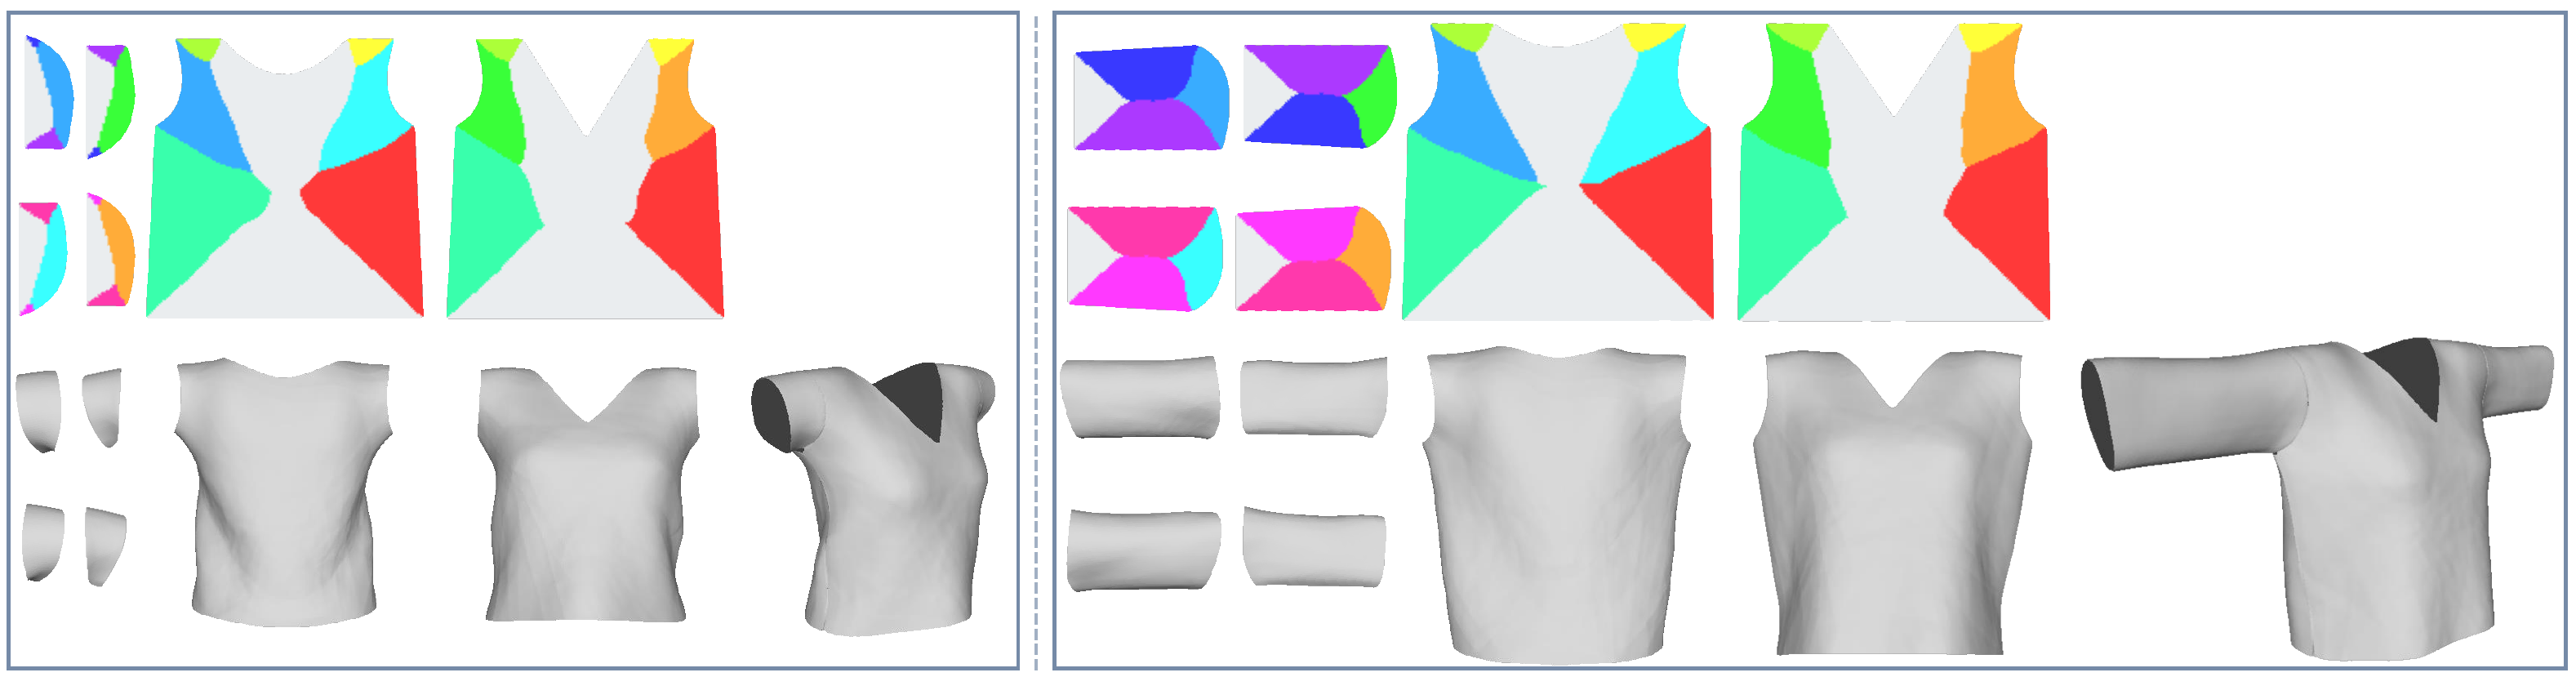}
    %\vspace{-0.35cm}
    \caption{\textbf{Reconstruction with 6 panels}. For both the left and right examples, we show the reconstructed panels on the top and the reconstructed surfaces and the sewed meshes at the bottom. Colors on panels denote edge labels predicted by $\mathcal{I}_{\Theta}$.}
    \label{fig:supp_6_panels_recon}
\end{figure}
