# Supplementary material for: ISP: Multi-Layered Garment Draping with Implicit Sewing Patterns
Source: arXiv:2305.14100 source file (2023-10-14)
Supplement: Supplementary file 5 [file supp_atlas.tex]

% !TEX root = ../top.tex
% !TEX spellcheck = en-US

\begin{figure}
    \centering
    \includegraphics[width=0.99\textwidth]{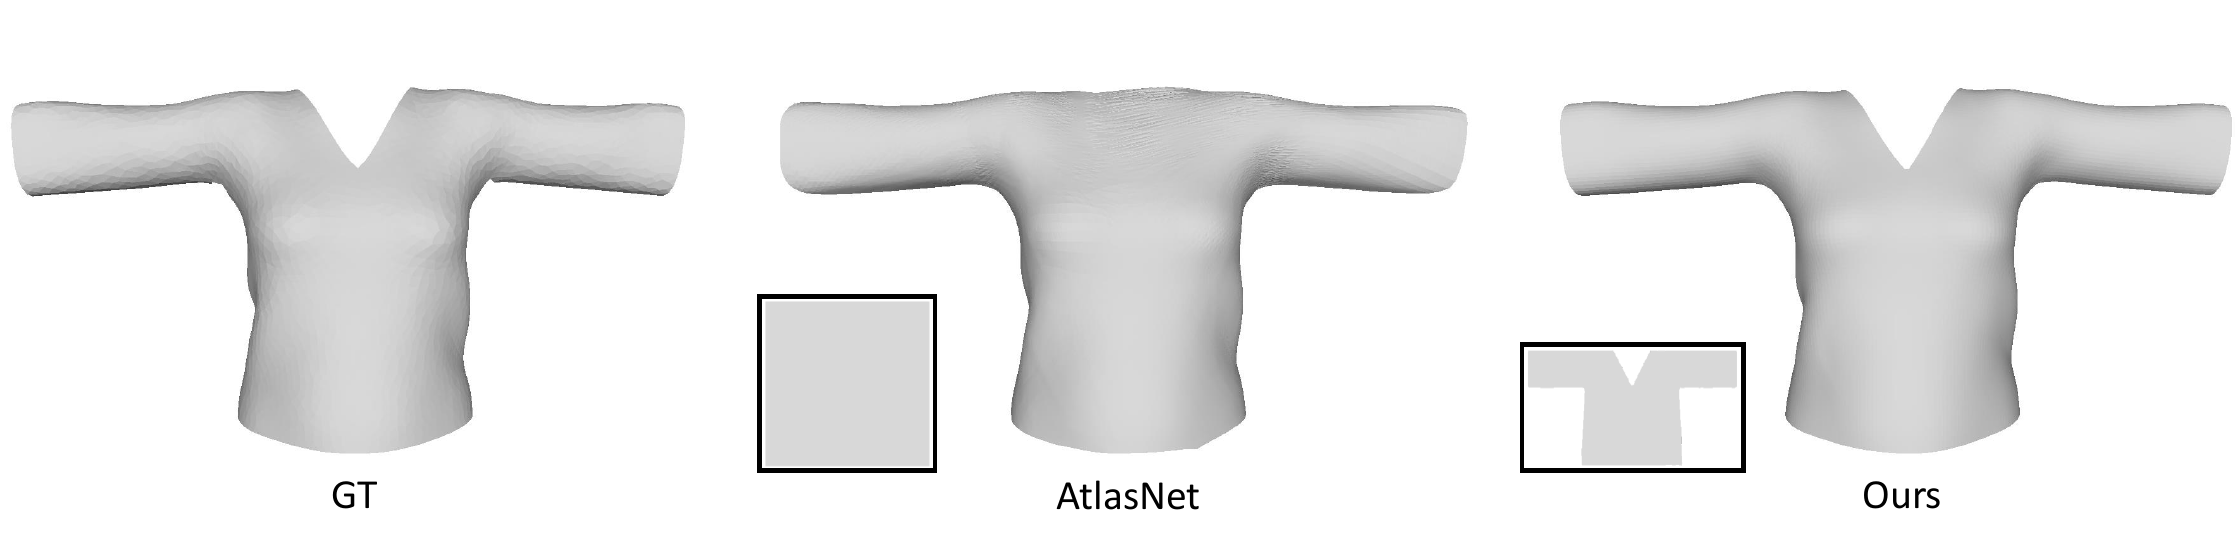}
    %\vspace{-0.35cm}
    \caption{\textbf{Comparison with AtlasNet}. The meshes in black boxes are the source patches where the mapping function is applied: a square patch for AtlastNet, a garment panel for our method.}
    \label{fig:supp_atlas}
    %\vspace{-0.45cm}
\end{figure}
