# Supplementary material for: ISP: Multi-Layered Garment Draping with Implicit Sewing Patterns
Source: arXiv:2305.14100 source file (2023-10-14)
Supplement: Supplementary file 6 [file supp_dig_snug_ours.tex]

% !TEX root = ../top.tex
% !TEX spellcheck = en-US

\begin{figure}[ht!]
    \centering
    \includegraphics[width=0.99\textwidth]{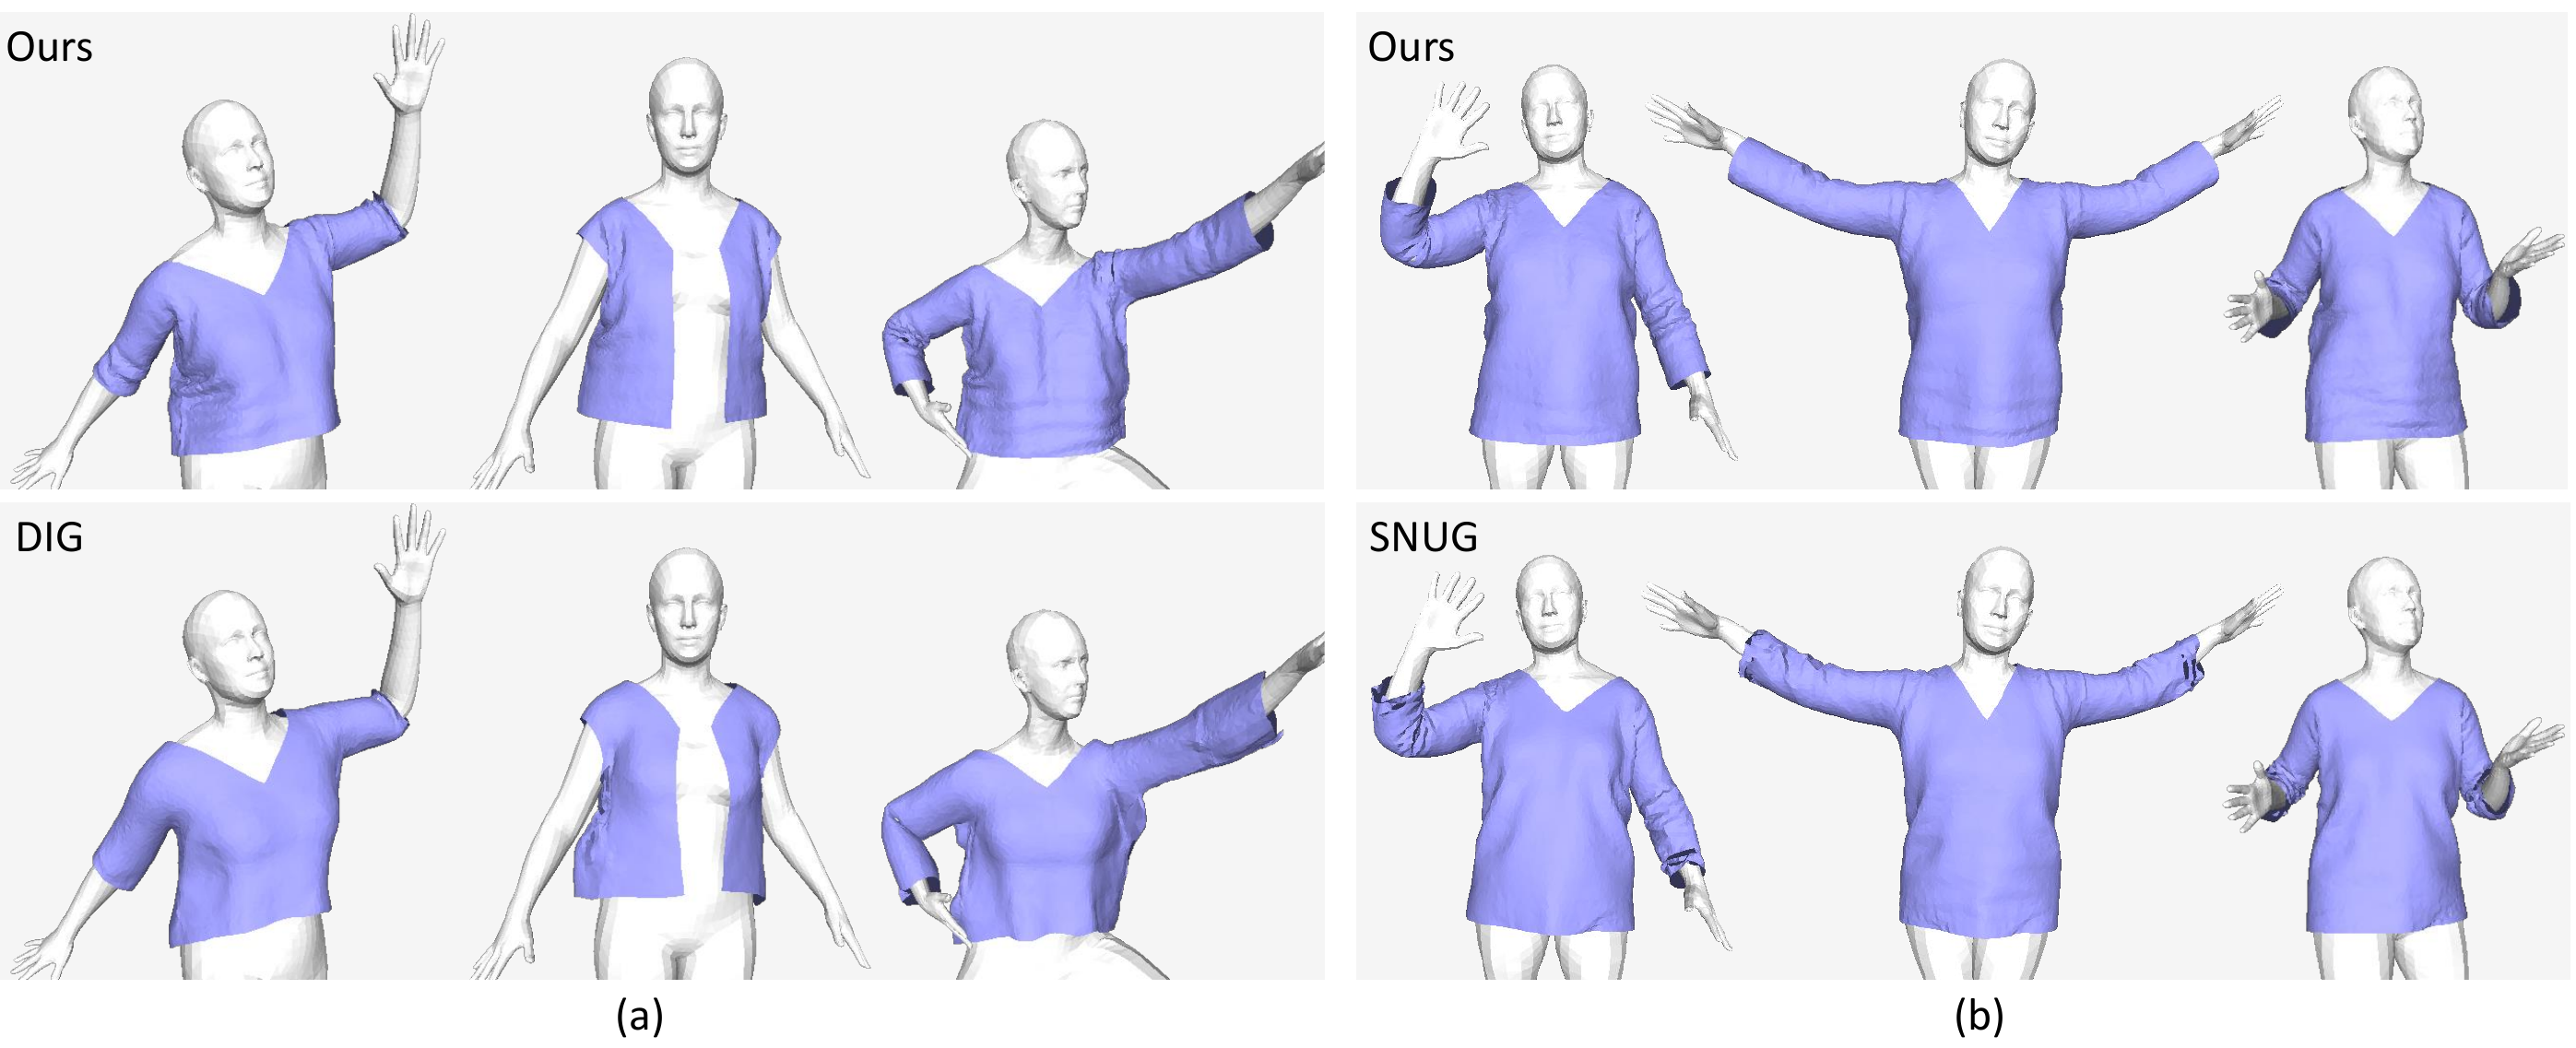}
    %\vspace{-0.35cm}
    \caption{The comparison of draping results for (a) our method vs. DIG, and (b) our method vs. SNUG.}
    \label{fig:supp_dig_snug_ours}
    %\vspace{-0.45cm}
\end{figure}
