# Supplementary material for: ISP: Multi-Layered Garment Draping with Implicit Sewing Patterns
Source: arXiv:2305.14100 source file (2023-10-14)
Supplement: Supplementary file 8 [file supp_heatmap.tex]

% !TEX root = ../top.tex
% !TEX spellcheck = en-US

\begin{figure}
    \centering
    \includegraphics[width=0.95\textwidth]{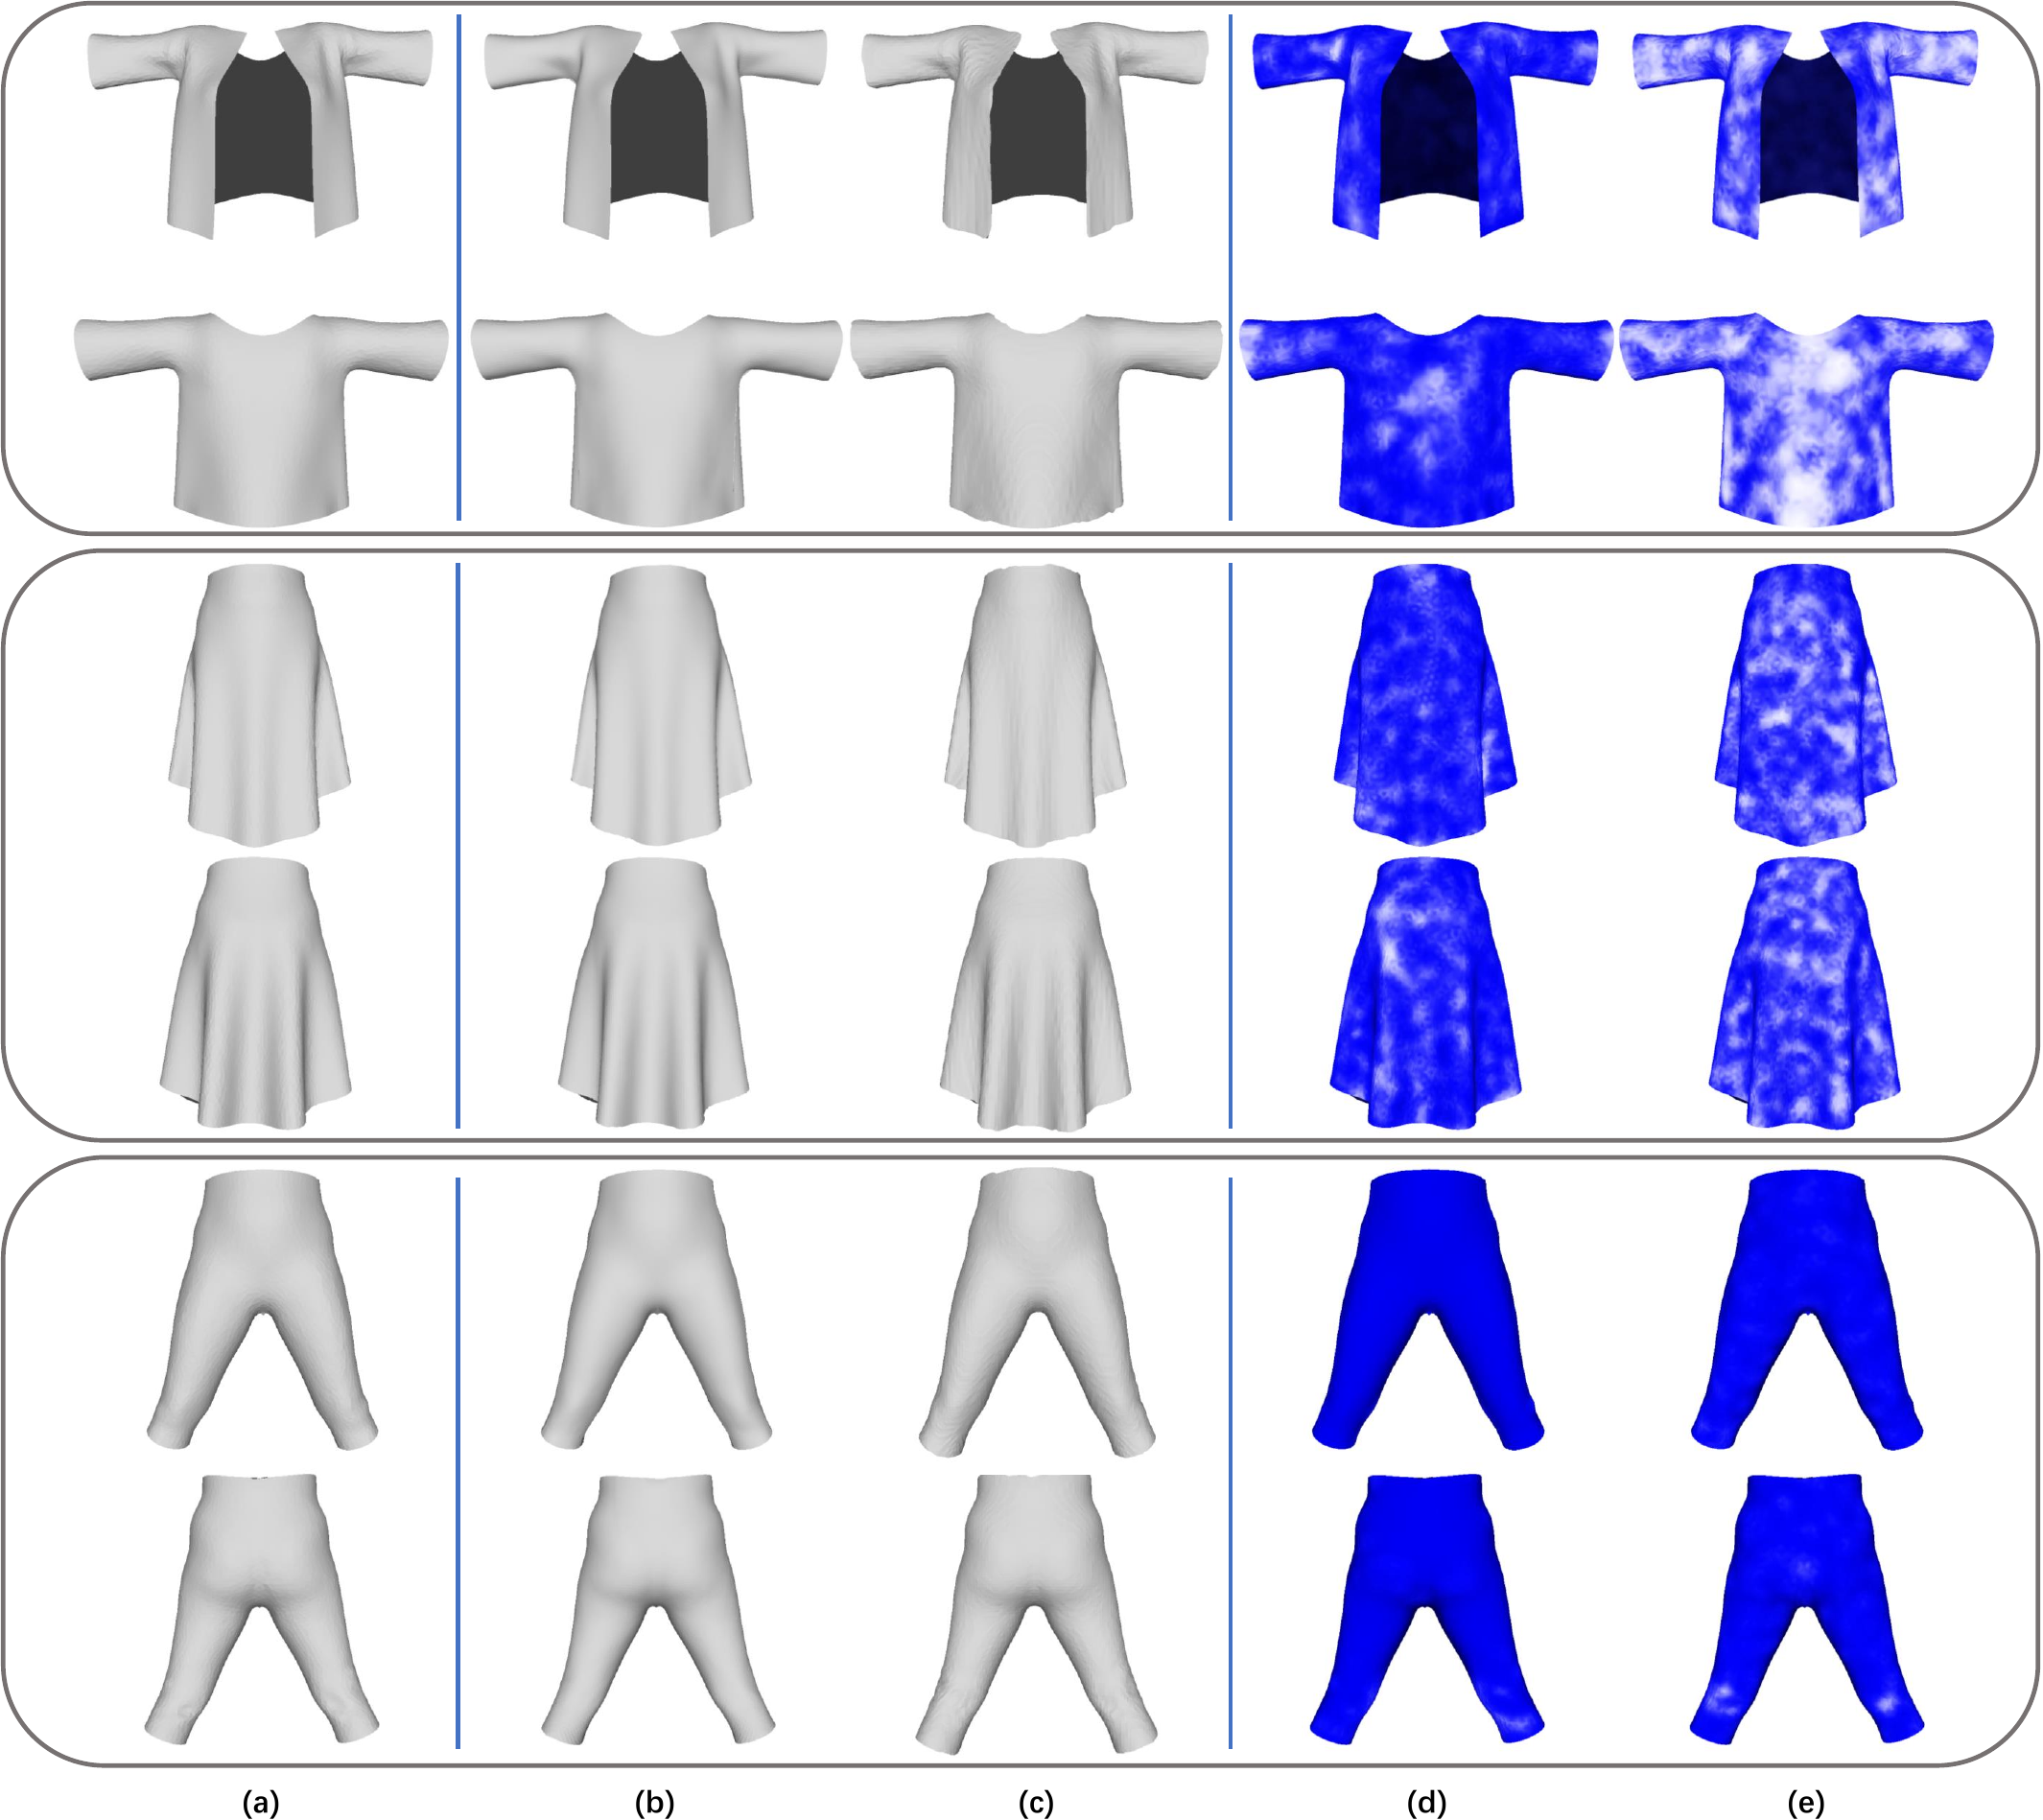}
    \caption{\textbf{Comparative analysis of mesh reconstruction and spatial error distribution for shirt, skirt and trousers}. (a) represents the ground truth mesh. (b) and (d) illustrate the mesh reconstruction and corresponding spatial error distribution for our proposed method. (c) and (e) display the same for UDFs. Each row provides both front (upper half) and back (lower half) views. In (d) and (e), error magnitude is indicated by color gradation, with white representing large errors and blue small errors.}
    \label{fig:supp_heatmap}
\end{figure}
