# Supplementary material for: ISP: Multi-Layered Garment Draping with Implicit Sewing Patterns
Source: arXiv:2305.14100 source file (2023-10-14)
Supplement: Supplementary file 9 [file supp_interp_pants.tex]

% !TEX root = ../top.tex
% !TEX spellcheck = en-US

\begin{figure}
    \centering
    \includegraphics[width=0.99\textwidth]{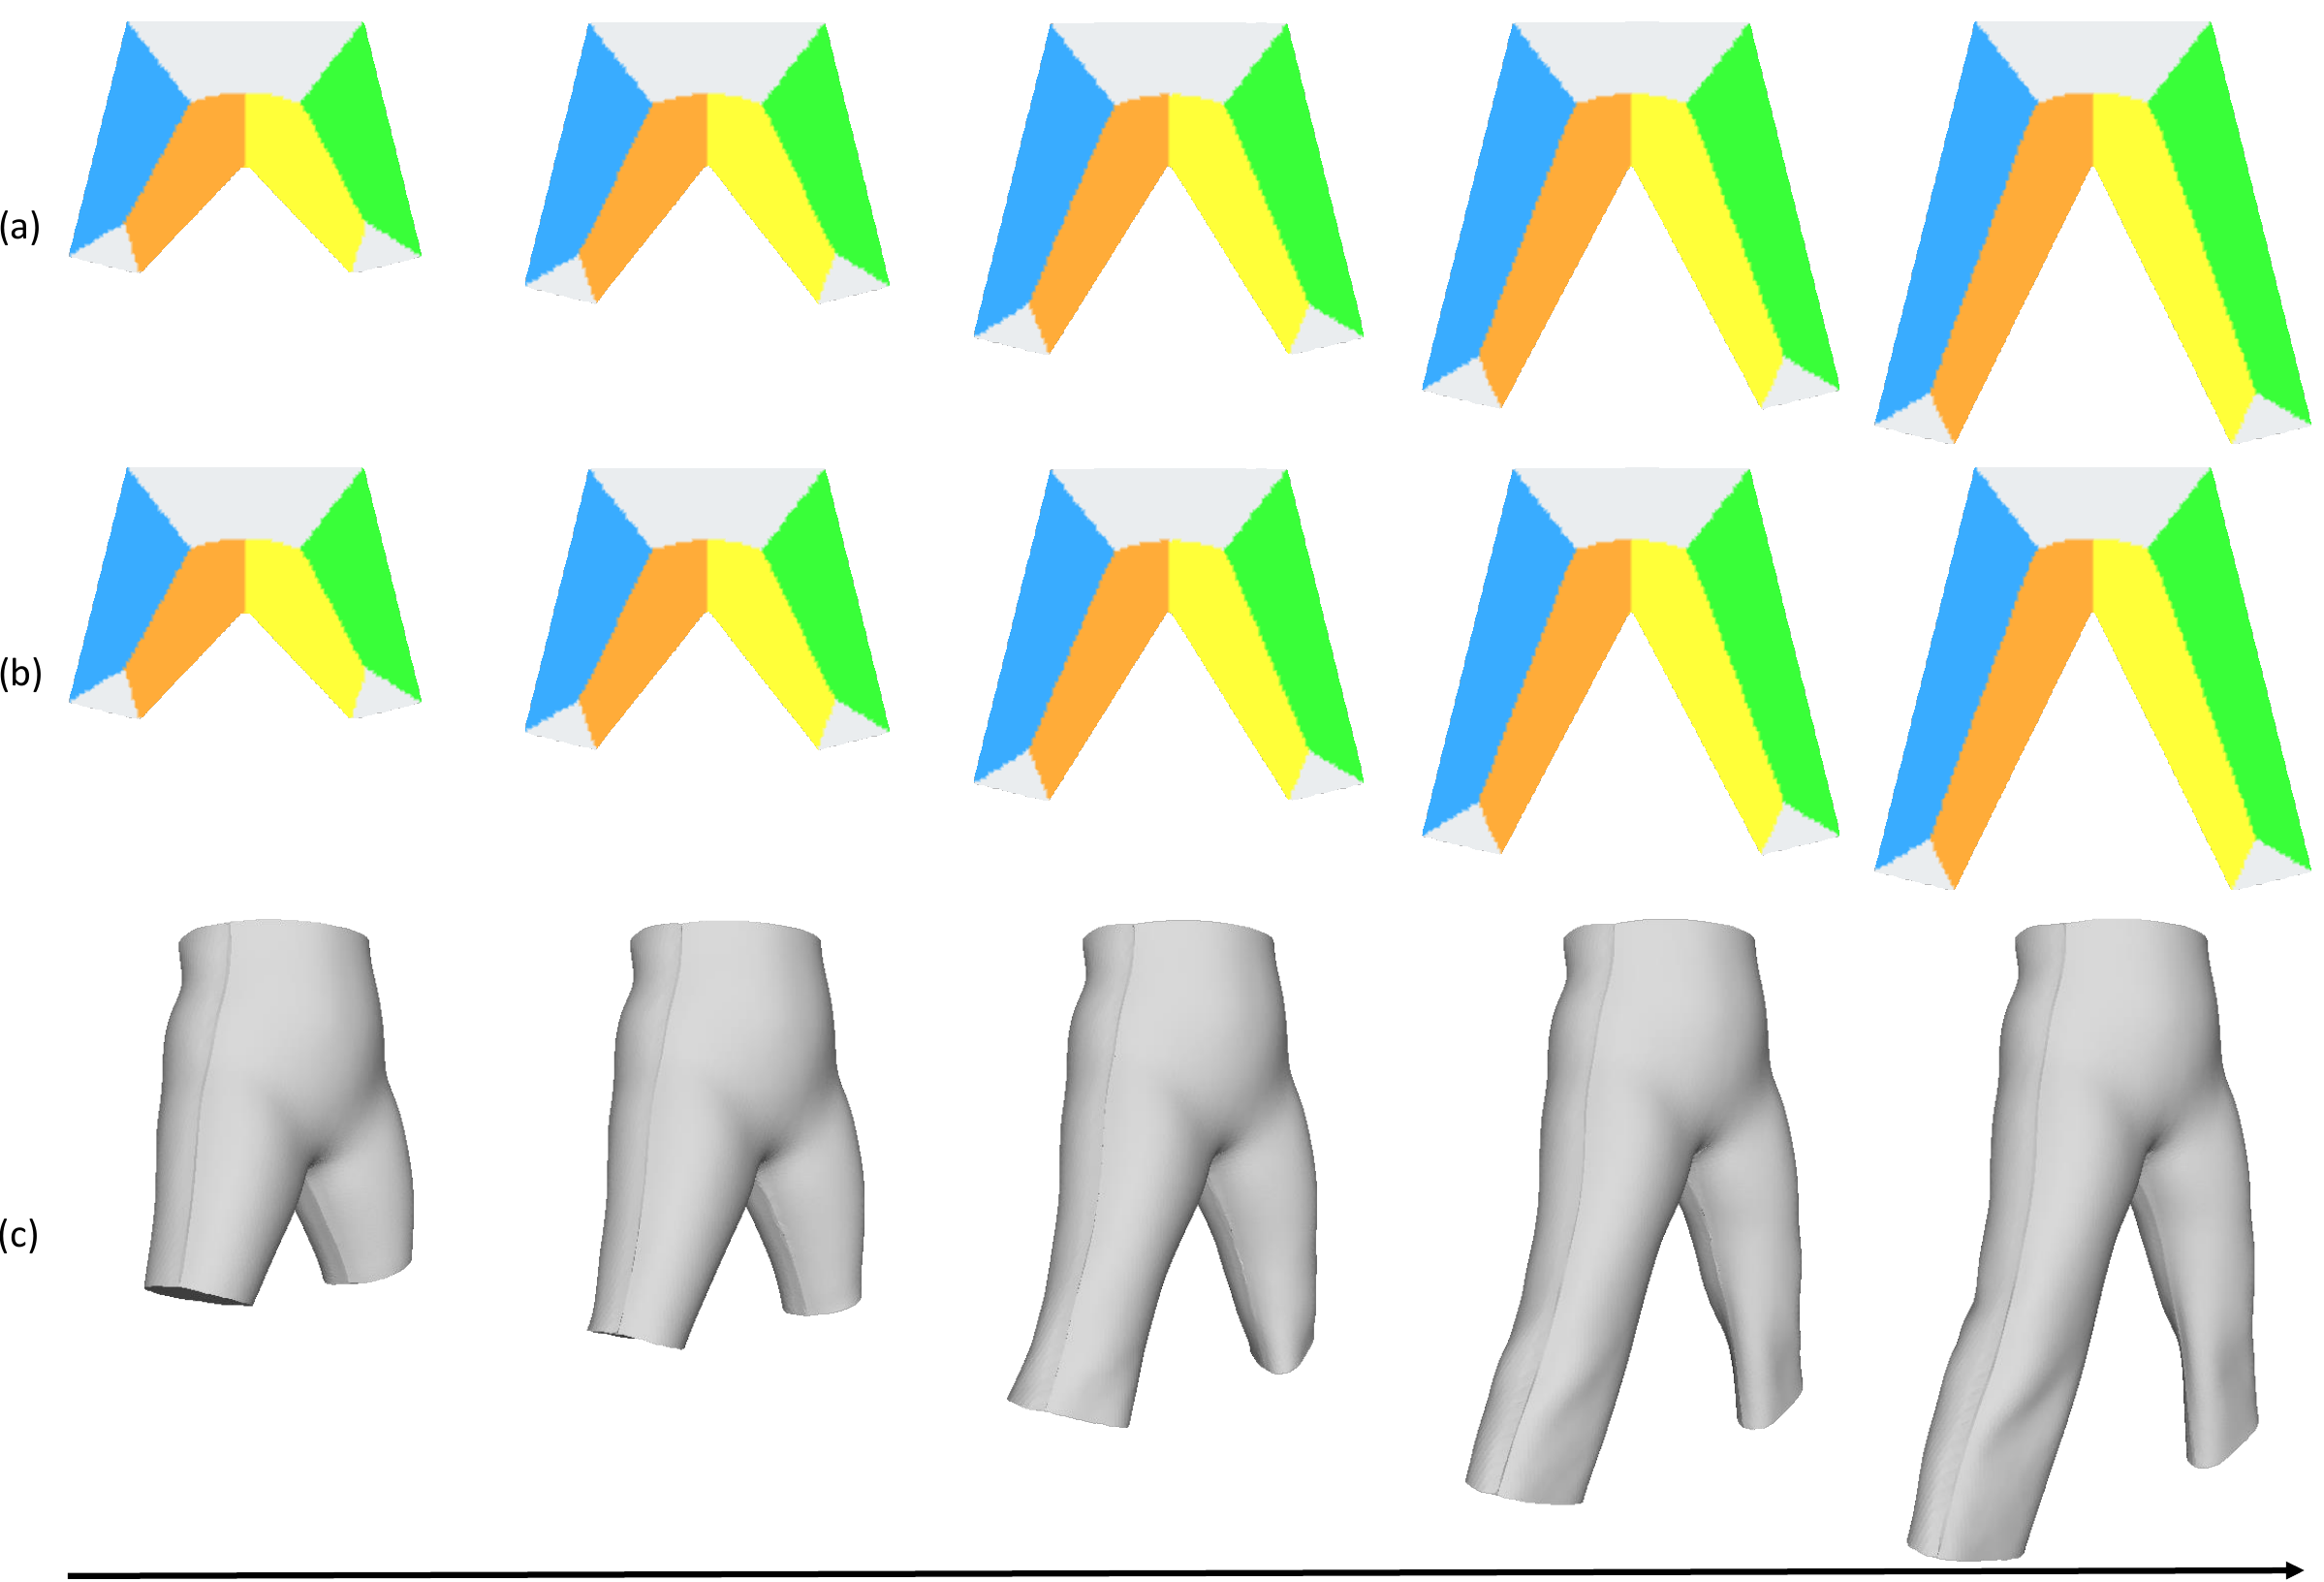}
    %\vspace{-0.35cm}
    \caption{\textbf{Interpolation}. We interpolate the latent code from a pair of short trousers to a pair of long trousers. (a) and (b) show the reconstructed front and back panels, where the colors on them denote the edge label fields. (c) shows the reconstructed mesh.}
    \label{fig:supp_interp_pants}
    %\vspace{-0.45cm}
\end{figure}
