# Supplementary material for: ISP: Multi-Layered Garment Draping with Implicit Sewing Patterns
Source: arXiv:2305.14100 source file (2023-10-14)
Supplement: Supplementary file 11 [file supp_layer.tex]

% !TEX root = ../top.tex
% !TEX spellcheck = en-US

\begin{figure}
    \centering
    \includegraphics[width=0.7\textwidth]{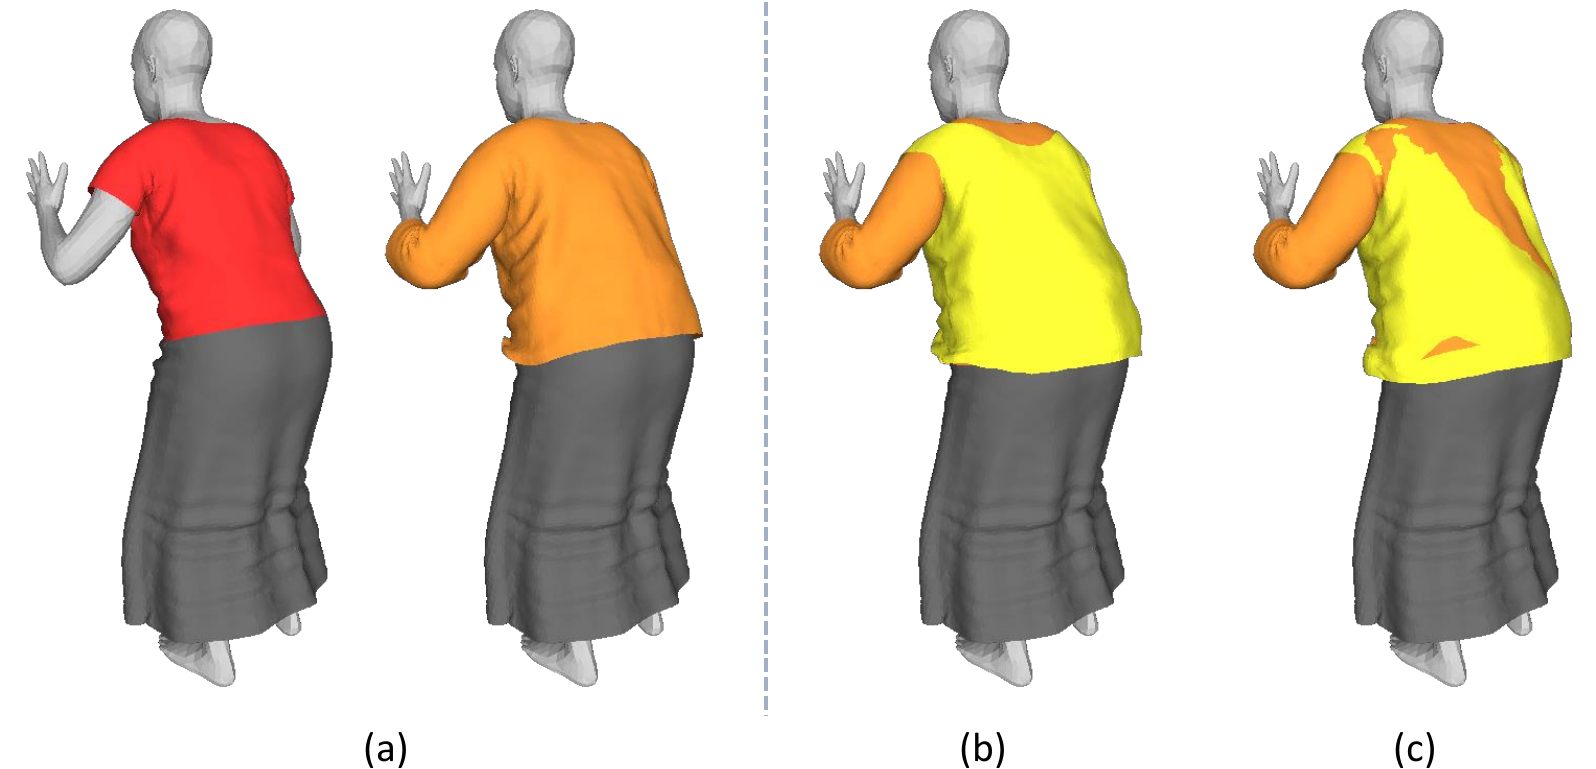}
    %\vspace{-0.35cm}
    \caption{\textbf{Ablation on layering.} We first drape a red and a orange shirts on the body (a), then a third one (yellow) is draped by the Algorithm \ref{alg:mld} (b) and the one-step algorithm (c).}
    \label{fig:supp_layer}
    %\vspace{-0.45cm}
\end{figure}
