# Supplementary material for: ISP: Multi-Layered Garment Draping with Implicit Sewing Patterns
Source: arXiv:2305.14100 source file (2023-10-14)
Supplement: Supplementary file 12 [file supp_mesh.tex]

% !TEX root = ../top.tex
% !TEX spellcheck = en-US

\begin{figure}[ht!]
    \centering
    \includegraphics[width=0.99\textwidth]{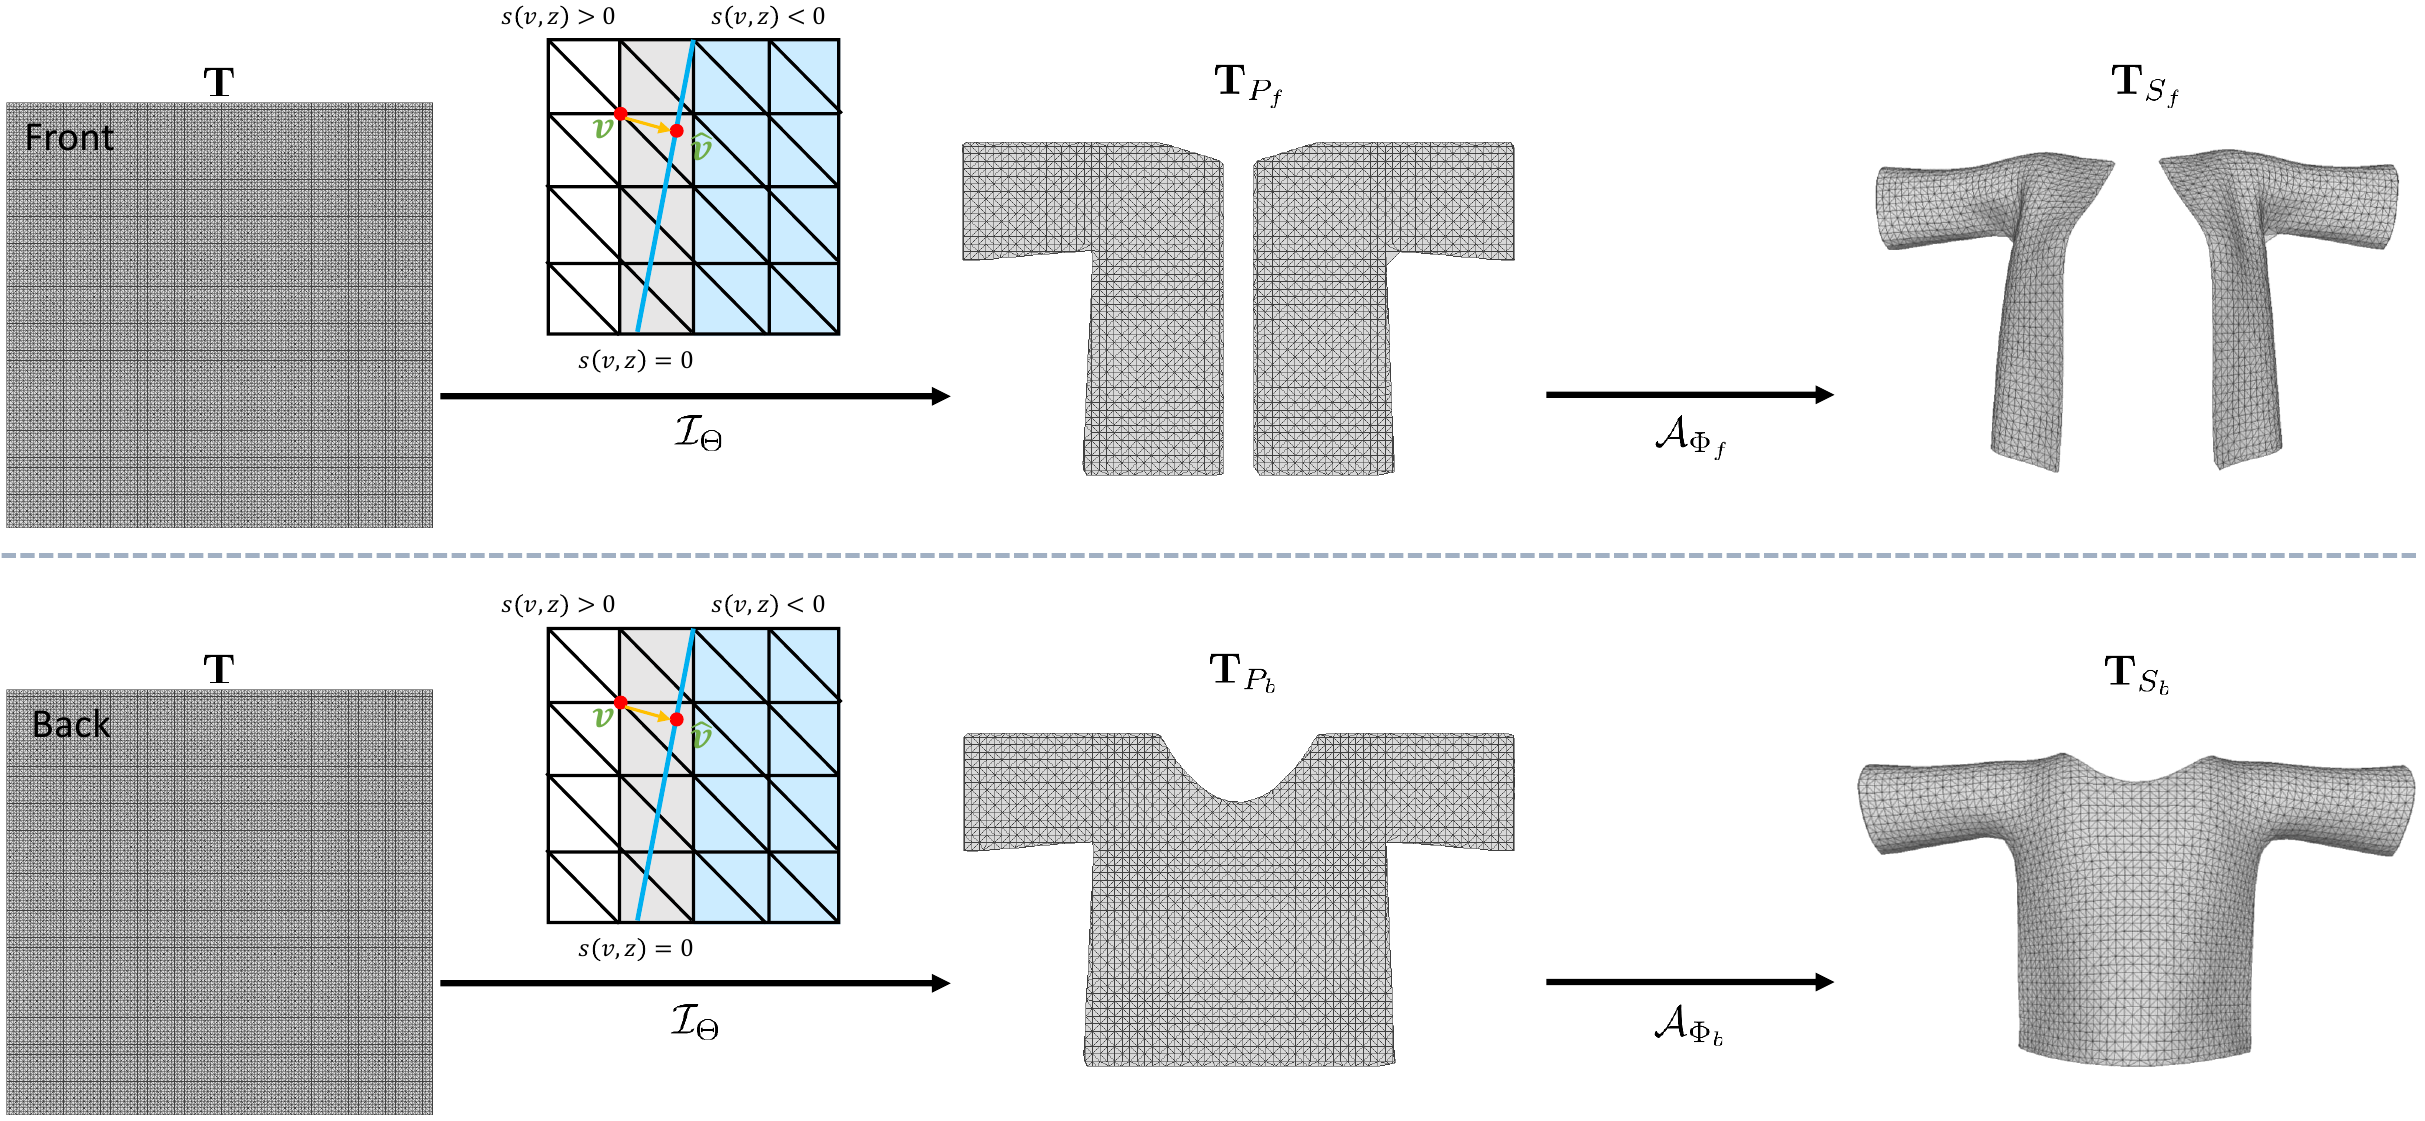}
    %\vspace{-0.35cm}
    \caption{\textbf{Meshing Process.} Starting with a square 2D mesh $\mathbf{T}$, we first extract the front and back panel meshes $\mathbf{T}_{P_f}$ and $\mathbf{T}_{P_b}$ using the implicit function $\mathcal{I}_{\Theta}$. Then we lift $\mathbf{T}_{P_f}$ and $\mathbf{T}_{P_b}$ to 3D to get the surface meshes $\mathbf{T}_{S_f}$ and $\mathbf{T}_{S_b}$ by querying $\mathcal{A}_{\Phi_f}$ and $\mathcal{A}_{\Phi_b}$ on their vertices respectively.}
    \label{fig:supp_mesh}
    %\vspace{-0.45cm}
\end{figure}
