# Supplementary material for: ISP: Multi-Layered Garment Draping with Implicit Sewing Patterns
Source: arXiv:2305.14100 source file (2023-10-14)
Supplement: Supplementary file 13 [file supp_pattern.tex]

% !TEX root = ../top.tex
% !TEX spellcheck = en-US

\begin{figure}[ht!]
    \centering
    \includegraphics[width=0.99\textwidth]{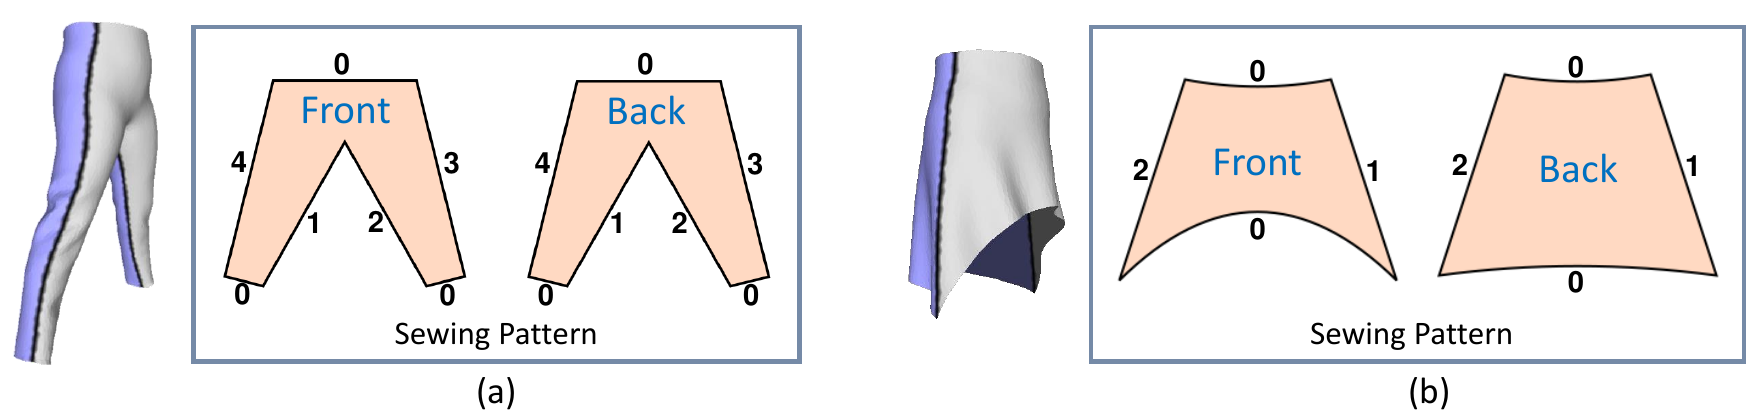}
    %\vspace{-0.35cm}
    \caption{The sewing patterns for (a) trousers and (b) skirts. The front mesh surfaces are in gray and the back ones in blue.}
    \label{fig:supp_pattern}
    %\vspace{-0.45cm}
  \end{figure}
