# Supplementary material for: ISP: Multi-Layered Garment Draping with Implicit Sewing Patterns
Source: arXiv:2305.14100 source file (2023-10-14)
Supplement: Supplementary file 14 [file supp_pipD.tex]

% !TEX root = ../top.tex
% !TEX spellcheck = en-US

\begin{figure}[ht!]
	\centering
		\begin{minipage}{.40\textwidth}
				\centering
		% \vspace{1mm}
		\includegraphics[width=0.99\textwidth]{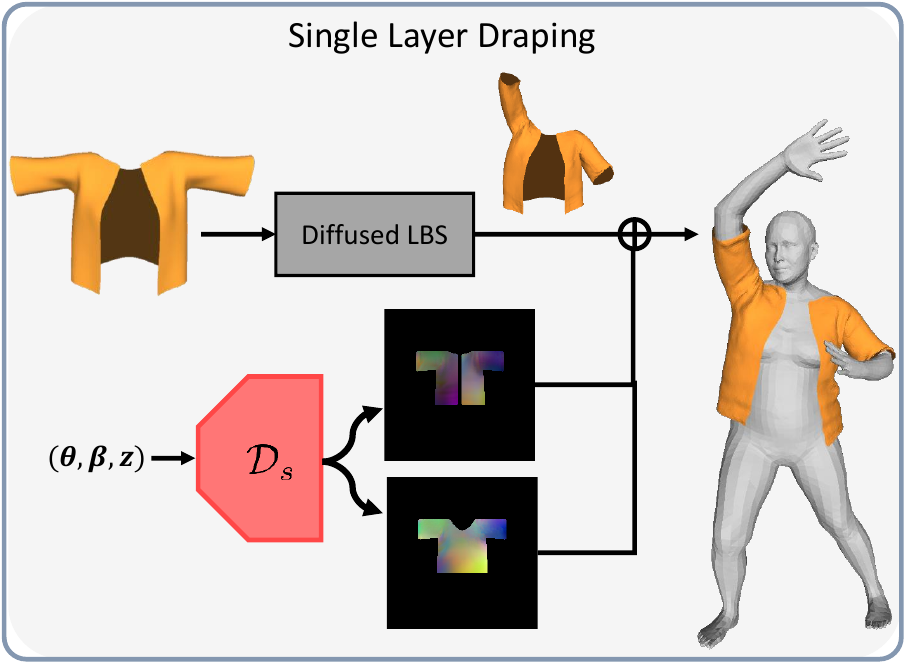}
		% \vspace{-7mm}
		\captionof{figure}{\textbf{Single layer draping.} The rest-state garment is first deformed by the diffused LBS to get the initial shape, and then refined by the displacement maps predicted by $\mathcal{D}_s$. }
		\label{fig:supp_pipD}
	\end{minipage}
	% \hspace{0mm}
    ~
	\begin{minipage}{.58\textwidth}
		\centering
		\includegraphics[width=.99\textwidth]{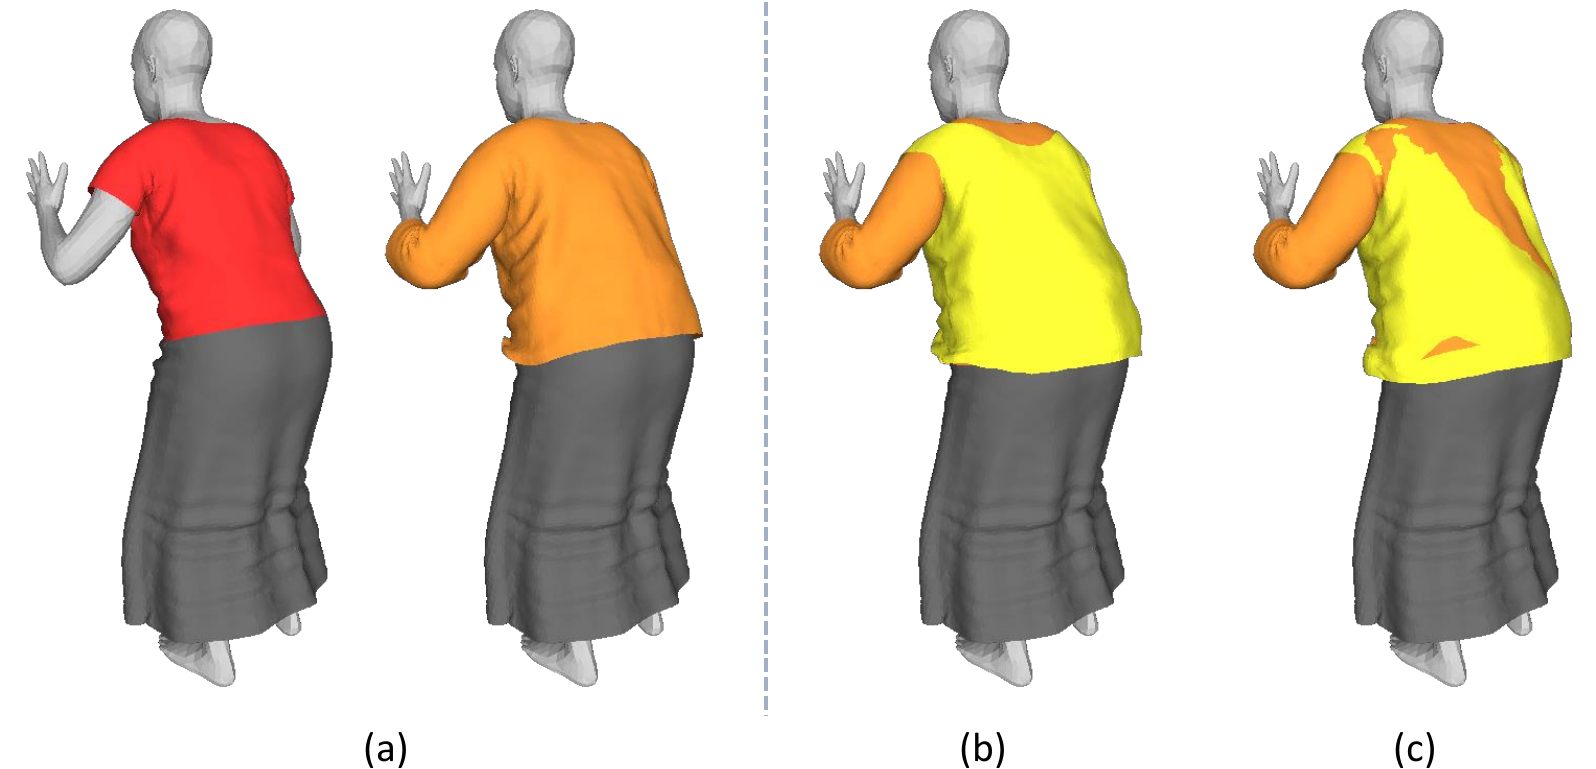}
		% \vspace{-10pt}
		\captionof{figure}{\textbf{Layering.} (a) We drape a red and an orange shirts on the body. A third one (yellow) is draped by (b) Algorithm \ref{alg:mld} and (c) by naively applying $\mathcal{D}_m$ to it.}
		\label{fig:supp_layer}
	\end{minipage}%
    \vspace{-0.45cm}
\end{figure}

\iffalse
\begin{figure}
    \centering
    \includegraphics[width=0.99\textwidth]{figs/supp_pipD_p.pdf}
    %\vspace{-0.35cm}
    \caption{\textbf{The pipeline of garment draping}. We first apply the network $\mathcal{D}_s$ to drape single garments. By utilizing the garment geometry and forces encoded in the input UV maps, we then rely on the network $\mathcal{D}_m$ to resolve garment intersections for multi-layered draping.}
    \label{fig:supp_pipD}
    %\vspace{-0.45cm}
\end{figure} 
\fi
