# Supplementary material for: ISP: Multi-Layered Garment Draping with Implicit Sewing Patterns
Source: arXiv:2305.14100 source file (2023-10-14)
Supplement: Supplementary file 17 [file supp_recon_skirt.tex]

\begin{figure}
    \centering
    \includegraphics[width=0.99\textwidth]{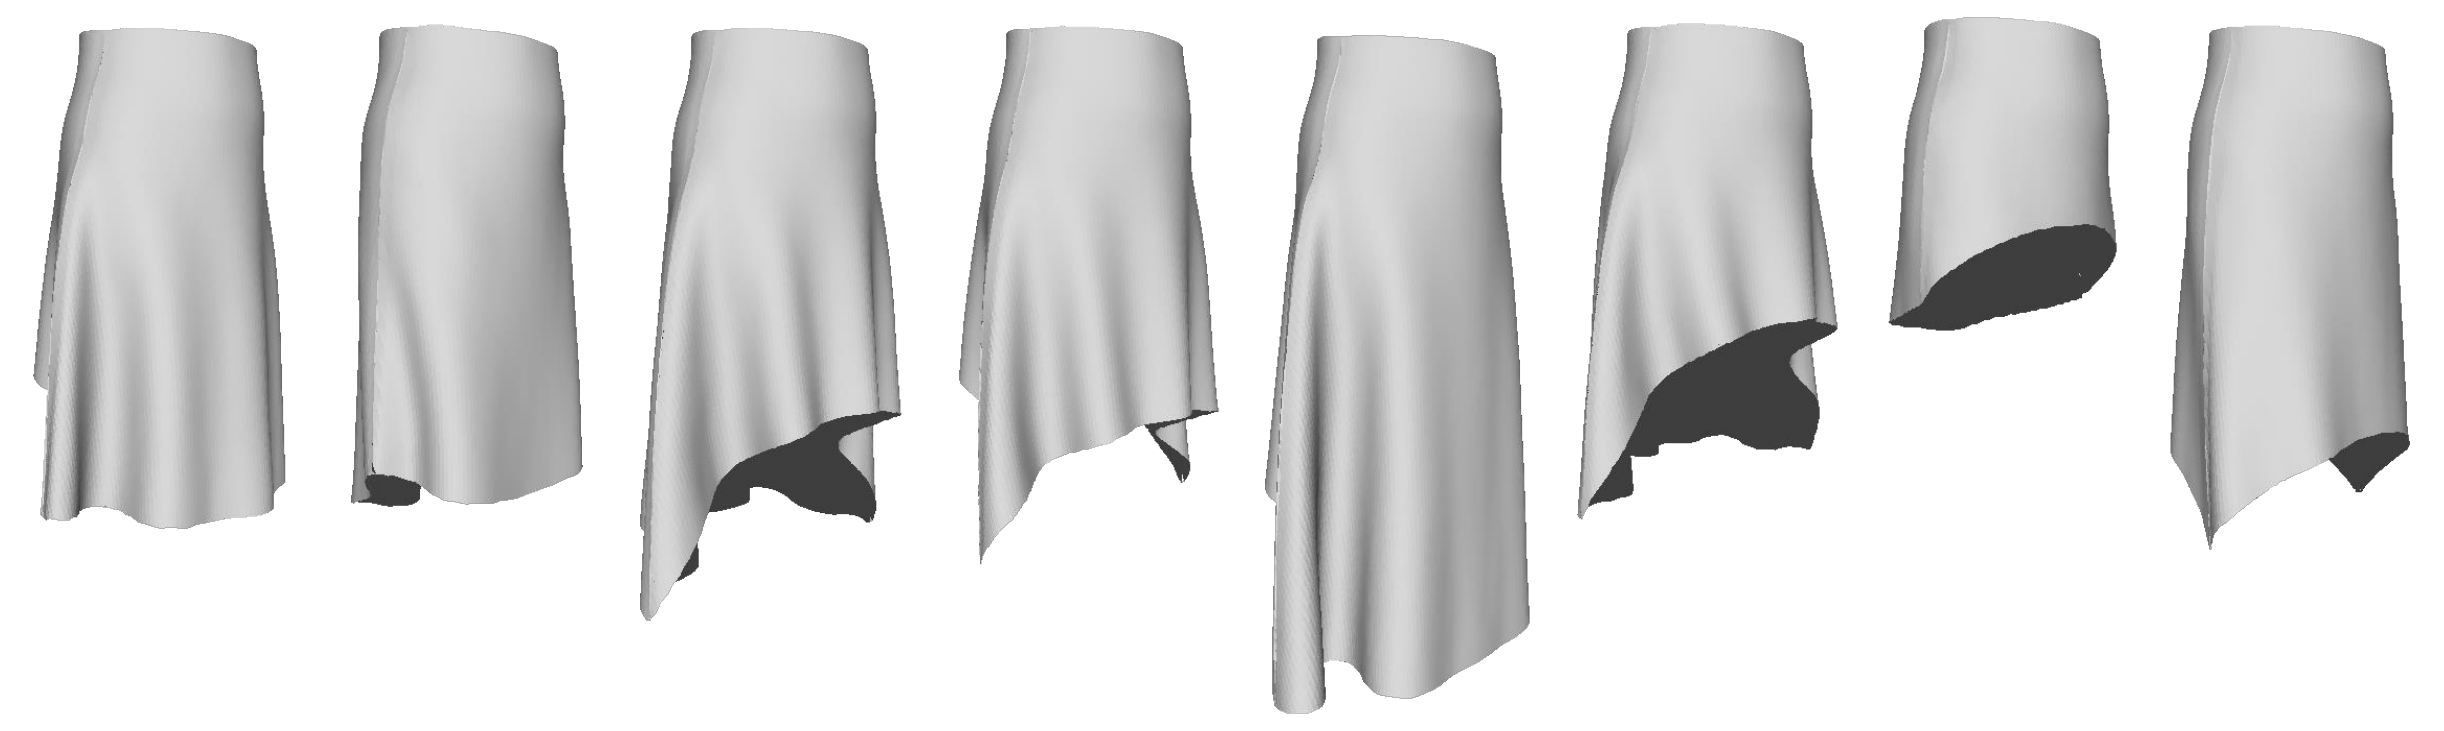}
    %\vspace{-0.35cm}
    \caption{Reconstruction samples of skirts.}
    \label{fig:supp_recon_skirt}
    %\vspace{-0.45cm}
\end{figure}
