# Supplementary material for: ISP: Multi-Layered Garment Draping with Implicit Sewing Patterns
Source: arXiv:2305.14100 source file (2023-10-14)
Supplement: Supplementary file 18 [file supp_seg.tex]

\begin{figure}[ht!]
    \centering
    \includegraphics[width=0.99\textwidth]{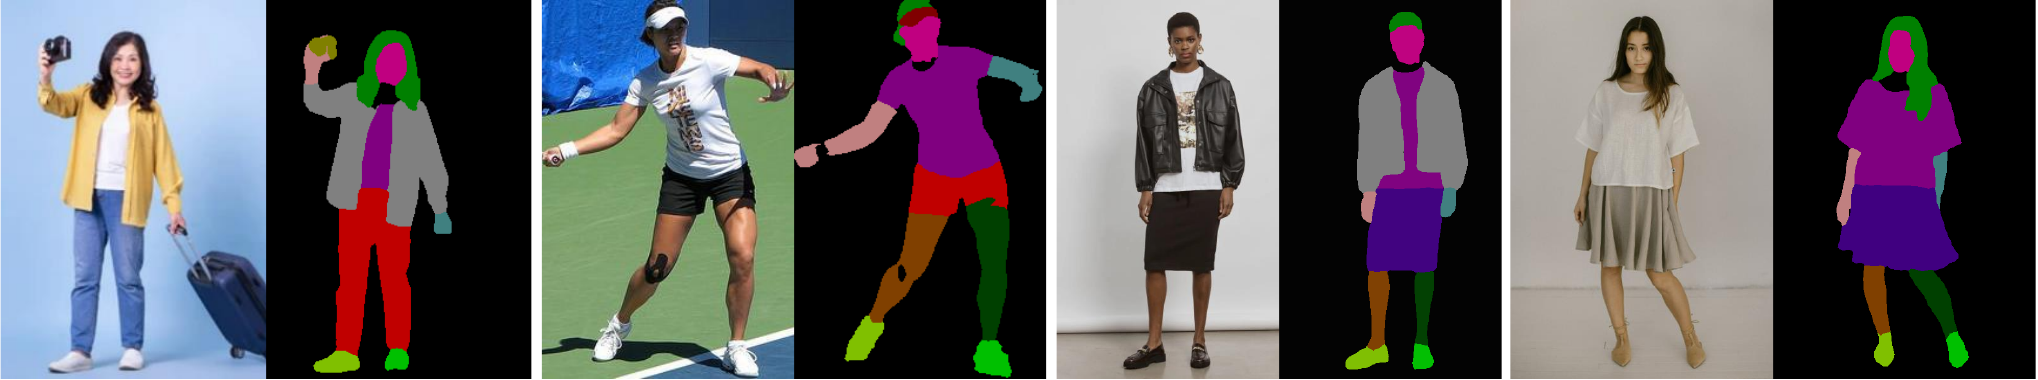}
    %\vspace{-0.35cm}
    \caption{Segmentation masks obtained from \cite{Li20i}. Jackets are marked in gray, shirts in purple, skirts in dark purple, trousers in red, and body parts in other colors.}
    \label{fig:supp_seg}
    %\vspace{-0.45cm}
\end{figure}
