# Supplementary material for: ISP: Multi-Layered Garment Draping with Implicit Sewing Patterns
Source: arXiv:2305.14100 source file (2023-10-14)
Supplement: Supplementary file 19 [file supp_sew.tex]

% !TEX root = ../top.tex
% !TEX spellcheck = en-US

\begin{figure}[ht!]
  \centering
  \includegraphics[width=0.9\textwidth]{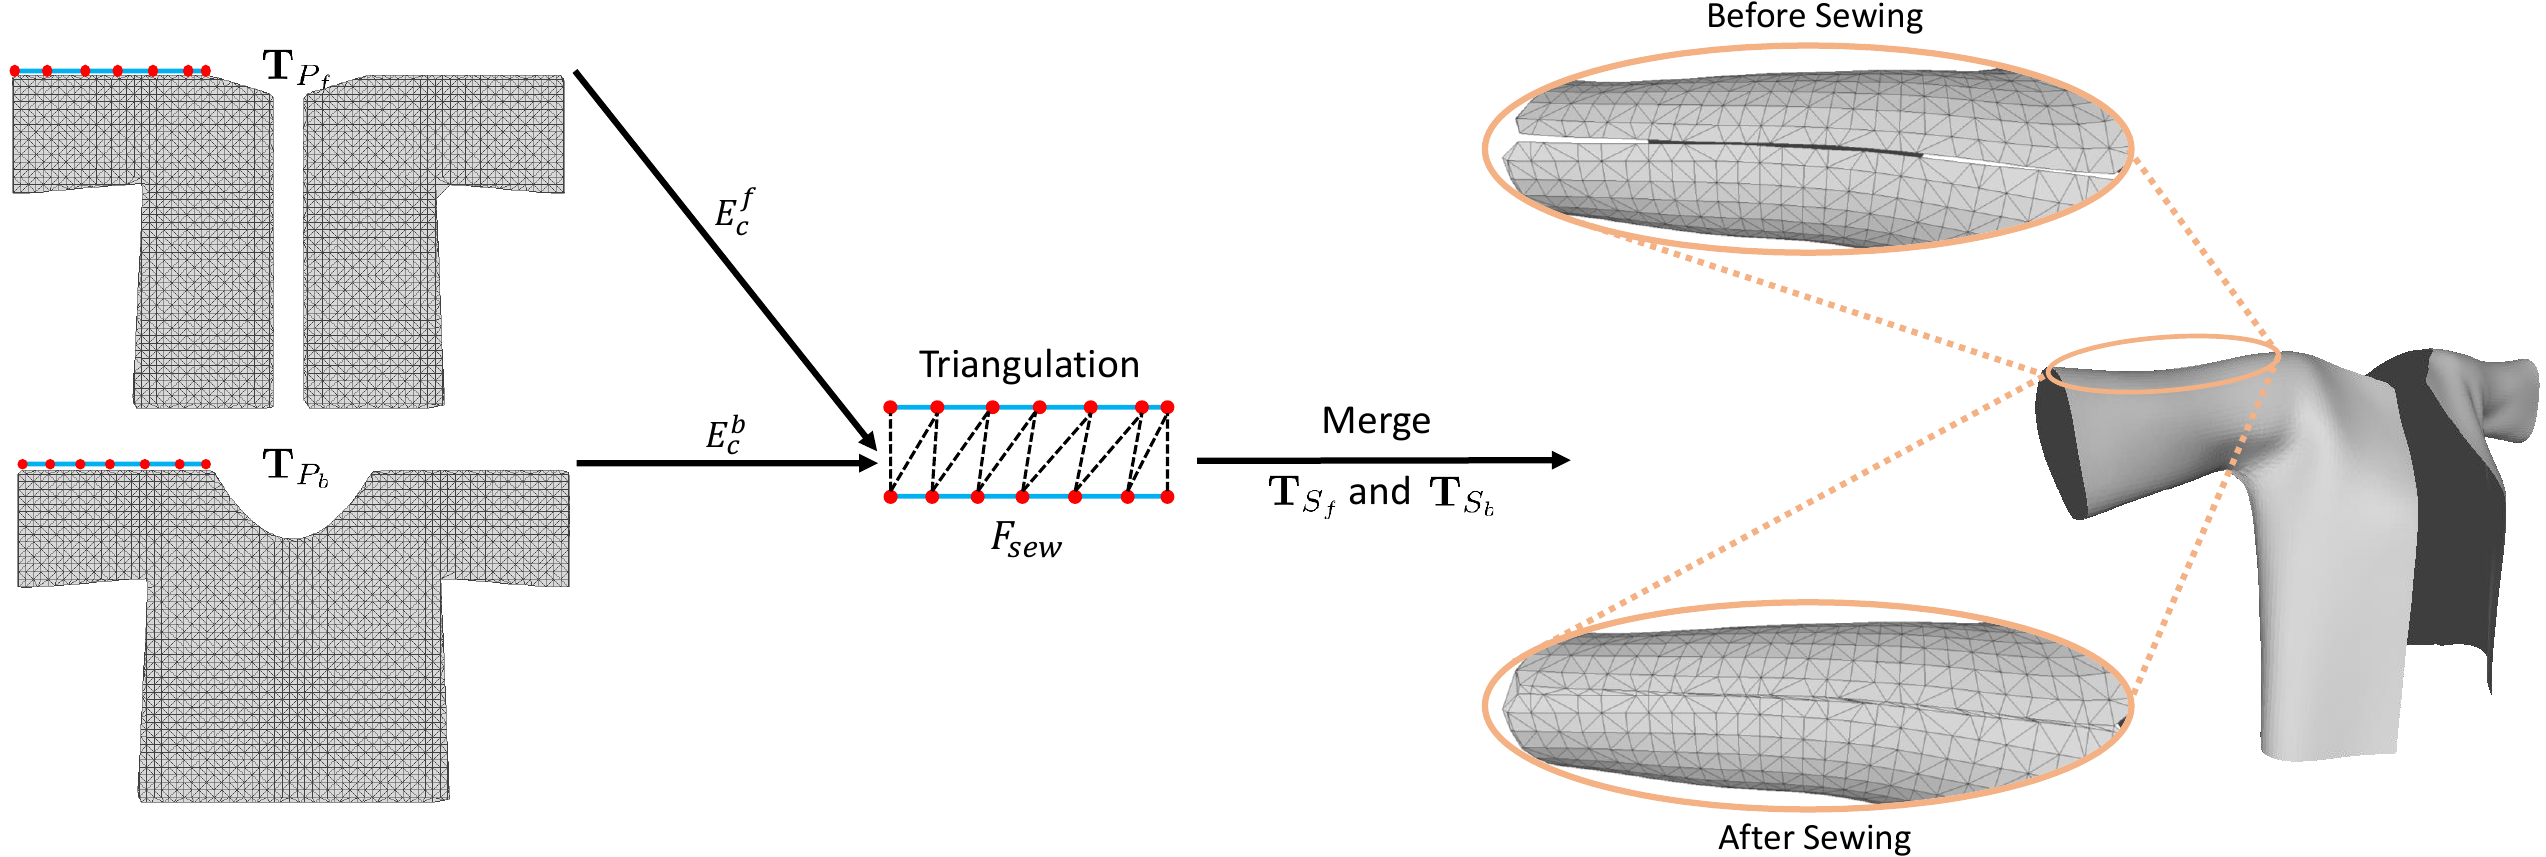}
  %\vspace{-0.35cm}
  \caption{\textbf{Sewing process.} Left: the boundary vertices belonging to the sewing edges $E_c^f$ and $E_c^b$ are marked in red. Middle: The triangulation is performed between $E_c^f$ and $E_c^b$ to create new faces $F_{sew}$. Right: The mesh generated by merging the front and back surfaces $\mathbf{T}_{S_f}$ and $\mathbf{T}_{S_b}$ with $F_{sew}$.}
  \label{fig:supp_sew}
  %\vspace{-0.45cm}
\end{figure}
